# Supplementary material for: SU(d)-Symmetric Random Unitaries: Quantum Scrambling, Error Correction, and Machine Learning
Source: arXiv:2309.16556 source file (2025-10-09)
Supplement: Supplementary file 1 [file CQA_SM2.pdf]

# Supplemental Material: $SU(d)$ -symmetric Random Unitaries: Quantum Scrambling, Error Correction, and Machine Learning

Zimu Li<sup>\*,1,\*</sup>, Han Zheng<sup>\*,2,3,†</sup>, Yunfei Wang<sup>\*,4</sup>, Liang Jiang<sup>\*,2,‡</sup>, Zi-Wen Liu<sup>\*,1,5,§</sup> and Junyu Liu<sup>\*,2,3,6,7,8,¶</sup>

<sup>1</sup>*Yau Mathematical Sciences Center, Tsinghua University, Beijing 100084, China*

<sup>2</sup>*Pritzker School of Molecular Engineering, The University of Chicago, Chicago, IL 60637, USA*

<sup>3</sup>*Department of Computer Science, The University of Chicago, Chicago, IL 60637, USA*

<sup>4</sup>*Martin A. Fisher School of Physics, Brandeis University, Waltham, MA, 02435, USA*

<sup>5</sup>*Perimeter Institute for Theoretical Physics, Waterloo, Ontario N2L 2Y5, Canada*

<sup>6</sup>*Kadanoff Center for Theoretical Physics, The University of Chicago, Chicago, IL 60637, USA*

<sup>7</sup>*qBraid Co., Chicago, IL 60637, USA*

<sup>8</sup>*SeQure, Chicago, IL 60637, USA*

In this Supplemental Material, we will provide more mathematical backgrounds and prove theorems given in the main text.

## CONTENTS

|                                                                                           |    |
|-------------------------------------------------------------------------------------------|----|
| I. Preliminaries                                                                          | 1  |
| A. Miscellaneous Facts on $S_n$ Representation Theory                                     | 1  |
| B. Schur-Weyl Duality and CQA Architecture                                                | 6  |
| C. Useful Properties on Quantum Entropies                                                 | 7  |
| II. Characterizing Random Circuit Designs by Commutant under Group Representation         | 9  |
| A. Quantum $k$ -fold Channel                                                              | 9  |
| B. Approximate $k$ -design and Random Walk on Group                                       | 10 |
| C. Frame Potential, Form factors, and $k$ -Invariance                                     | 12 |
| D. Commutant of the Group $U(\bigoplus_\lambda S^\lambda)$ of $SU(d)$ Symmetric Unitaries | 14 |
| III. Applications of $SU(d)$ Symmetric 2-design                                           | 17 |
| A. General Setting and Explicit Expansion for $T_{k=2}^{CQA}$                             | 17 |
| B. Spreading of Local $SU(d)$ Conserved Quantities                                        | 20 |
| C. Spreading of Local $U(1)$ Conserved Quantities                                         | 27 |
| D. $SU(d)$ Covariant Error Correction Code                                                | 28 |
| E. Overparametrization Regime with $SU(d)$ Symmetric Local Quantities                     | 35 |
| References                                                                                | 38 |

## I. PRELIMINARIES

We briefly introduce some basic notions and facts from  $S_n$  representation theory, as well as our CQA model, that may provide a comprehensive understanding on the later mathematical proofs. We also recommend the interested readers to [1–5] for more systematic presentations on these topics.

### A. Miscellaneous Facts on $S_n$ Representation Theory

Irreducible representations (irreps) of the symmetric group  $S_n$  permuting  $n$  nodes are in one-to-one correspondence with the so-called *Young diagrams*, e.g., for  $S_6$  the following two Young diagrams stand for the *trivial* and the *fundamental* representation:

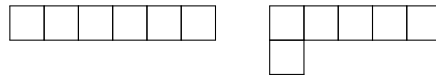

\* lizm@mail.sustech.edu.cn

† hanz98@uchicago.edu

‡ liangjiang@uchicago.edu

§ zwliu.permanent@gmail.com

¶ junyuliu@uchicago.edu

whose direct sum is more familiar as the 6-dimensional defining representation under which each  $\sigma \in S_6$  permutes the components of vectors from  $\mathbb{R}^6$ .

**Definition I.1.** Formally, let  $\lambda = (\lambda_1, \dots, \lambda_r)$  be a collection of positive integers such that  $\lambda_i \geq \lambda_{i+1}$  and  $\sum_i \lambda_i = n$ . Then  $\lambda$  is called a *partition of the integer  $n$* , denoted by  $\lambda \vdash n$ . Obviously,  $\lambda$  defines a Young diagram abstractly and the  $S_n$  irrep corresponding to this Young diagram is always denoted as  $S^\lambda$ . The dimension of this irrep is given by the *hook length formula*:

$$\dim S^\lambda = \frac{n!}{\prod_{(x,y) \in \lambda} h_{x,y}}, \quad (1)$$

where  $(x, y)$  specifies a box from  $\lambda$  by its *row* and *column numbers* and  $h(x, y)$  counts the number of all boxes on the right hand side and below  $(x, y)$ , including itself.

Given an arbitrary  $S_n$  irrep  $S^\lambda$ , there is a canonical way to label a basis, called *Gelfand-Tsetlin basis (GZ)* or *Young-Yamanouchi basis*, on the representation space using *standard Young tableau  $T$* , which are defined by filling into each box of  $\lambda$  a positive integer from  $1, 2, \dots, n$  in an increasing order from left to right and top to bottom. For instance, the fundamental representation of  $S_6$  mentioned above is 5-dimensional with 5 basis vectors being labeled as

$$\begin{array}{|c|c|c|c|c|} \hline 1 & 2 & 3 & 4 & 5 \\ \hline 6 & & & & \\ \hline \end{array}, \quad \begin{array}{|c|c|c|c|c|} \hline 1 & 2 & 3 & 4 & 6 \\ \hline 5 & & & & \\ \hline \end{array}, \quad \begin{array}{|c|c|c|c|c|} \hline 1 & 2 & 3 & 5 & 6 \\ \hline 4 & & & & \\ \hline \end{array}, \quad \begin{array}{|c|c|c|c|c|} \hline 1 & 2 & 4 & 5 & 6 \\ \hline 3 & & & & \\ \hline \end{array}, \quad \begin{array}{|c|c|c|c|c|} \hline 1 & 3 & 4 & 5 & 6 \\ \hline 2 & & & & \\ \hline \end{array}.$$

When we study the group commutant of  $SU(d)$  symmetric unitaries in the main text, Young basis  $\{|\alpha_T\rangle\}$  labeled by standard tableaux are implicitly used and a detailed treatment can be found in Section II D.

**Definition I.2.** For  $1 < k \leq n$ , the *Young-Jucys-Murphy element*, or YJM-element for short, is defined as a (formal) sum of *transpositions* or SWAPs

$$X_i = (1, i) + (2, i) + \dots + (i-1, i) \quad (2)$$

We set  $X_1 = 0$  as a convention.

YJM-element is the central concept used in our work developed by Young [6], Jucys [7] and Murphy [8] and later used by Okounkov and Vershik [9]. Under any  $S_n$  representation, it may be more comprehensible to treat  $X_i = (1, i) + (2, i) + \dots + (i-1, i)$  as the sum of matrix representations of these transpositions, or we can say that the representation is extended to the *group algebra*

$$\mathbb{C}[S_n] = \left\{ \sum_i c_i \sigma_i; \sigma_i \in S_n \right\} \quad (3)$$

consisting of formal finite linear combinations  $S_n$  group elements. By Wedderburn Theorem [2, 3],  $\mathbb{C}[S_n]$  is isomorphic with the direct sum of all inequivalent  $S_n$  irreps  $\bigoplus_\lambda S^\lambda$ . By Schur-Weyl duality, the  $\mathbb{C}[S_n]$  embraces all  $SU(d)$ -symmetric local Hamiltonian which is used to argue a quantum speedup in [5]. It also provides a perspective to discuss  $k$ -design through Lie group and Lie algebra.

Let us consider coordinate differences  $x - y$  of boxes from a Young diagram  $\lambda$ . Given any standard tableaux  $T$  of  $\lambda$ , its *content vector* is defined by rearranging them with respect to the order of boxes determined by the tableau. For example, content vectors of the above five standard tableaux are listed as follows:

$$(0, 1, 2, 3, 4, -1), \quad (0, 1, 2, 3, -1, 4), \quad (0, 1, 2, -1, 3, 4), \quad (0, 1, -1, 2, 3, 4), \quad (0, -1, 1, 2, 3, 4).$$

One significant feature of YJM-elements is their special actions under Young basis revealed by content vectors:

1. They are diagonal matrices under Young basis (even each single transposition  $(i, j)$  from Eq.(2) may not be diagonal).
2. The diagonal entries of  $X_i$  under the Young basis vector  $|\alpha_T\rangle$  corresponding to standard tableau  $T$  is just the  $i$ th component of the content vector.

On the irrep  $S^{(5,1)}$ ,

$$\begin{aligned} X_1 &= \begin{pmatrix} 0 & 0 & 0 & 0 & 0 \\ 0 & 0 & 0 & 0 & 0 \\ 0 & 0 & 0 & 0 & 0 \\ 0 & 0 & 0 & 0 & 0 \\ 0 & 0 & 0 & 0 & 0 \end{pmatrix}, & X_2 &= \begin{pmatrix} 1 & 0 & 0 & 0 & 0 \\ 0 & 1 & 0 & 0 & 0 \\ 0 & 0 & 1 & 0 & 0 \\ 0 & 0 & 0 & 1 & 0 \\ 0 & 0 & 0 & 0 & -1 \end{pmatrix}, & X_3 &= \begin{pmatrix} 2 & 0 & 0 & 0 & 0 \\ 0 & 2 & 0 & 0 & 0 \\ 0 & 0 & 2 & 0 & 0 \\ 0 & 0 & 0 & -1 & 0 \\ 0 & 0 & 0 & 0 & 1 \end{pmatrix}, \\ X_4 &= \begin{pmatrix} 3 & 0 & 0 & 0 & 0 \\ 0 & 3 & 0 & 0 & 0 \\ 0 & 0 & -1 & 0 & 0 \\ 0 & 0 & 0 & 2 & 0 \\ 0 & 0 & 0 & 0 & 2 \end{pmatrix}, & X_5 &= \begin{pmatrix} 4 & 0 & 0 & 0 & 0 \\ 0 & -1 & 0 & 0 & 0 \\ 0 & 0 & 3 & 0 & 0 \\ 0 & 0 & 0 & 3 & 0 \\ 0 & 0 & 0 & 0 & 3 \end{pmatrix}, & X_6 &= \begin{pmatrix} -1 & 0 & 0 & 0 & 0 \\ 0 & 4 & 0 & 0 & 0 \\ 0 & 0 & 4 & 0 & 0 \\ 0 & 0 & 0 & 4 & 0 \\ 0 & 0 & 0 & 0 & 4 \end{pmatrix} \end{aligned} \quad (4)$$

In summary, *Young basis vectors*  $|\alpha_T\rangle$ , *standard tableaux*  $T$  and *content vectors*  $\alpha_T$  are in one-to-one correspondence and uniquely determine the matrix representations of *YJM-elements*.

As mentioned when introducing our numerical method in the main text, Matrix representation of each *adjacent transposition*  $(i, i+1)$  can be explicitly read off under Young basis by *Young orthogonal form*: let  $r = \alpha_T(i+1) - \alpha_T(i)$  be the *axial distance* and let  $(i, i+1) \cdot T$  denote the tableau defined by exchanging integers  $i, i+1$  from  $T$ . It is easy to check that as long as  $r \neq \pm 1$ ,  $(i, i+1) \cdot T$  is still a standard Young tableau. Then

$$(i, i+1) |\alpha_T\rangle = \frac{1}{r} |\alpha_T\rangle + \sqrt{1 - \frac{1}{r^2}} |\alpha_{(i,i+1) \cdot T}\rangle, \quad (i, i+1) |\alpha_{(i,i+1) \cdot T}\rangle = \sqrt{1 - \frac{1}{r^2}} |\alpha_T\rangle - \frac{1}{r} |\alpha_{(i,i+1) \cdot T}\rangle. \quad (5)$$

On the irrep  $S^{(5,1)}$ ,

$$\begin{aligned} (1, 2) &= \begin{pmatrix} 1 & 0 & 0 & 0 & 0 \\ 0 & 1 & 0 & 0 & 0 \\ 0 & 0 & 1 & 0 & 0 \\ 0 & 0 & 0 & 1 & 0 \\ 0 & 0 & 0 & 0 & -1 \end{pmatrix}, & (2, 3) &= \begin{pmatrix} 1 & 0 & 0 & 0 & 0 \\ 0 & 1 & 0 & 0 & 0 \\ 0 & 0 & 1 & 0 & 0 \\ 0 & 0 & 0 & -\frac{1}{2} & \frac{\sqrt{3}}{2} \\ 0 & 0 & 0 & \frac{\sqrt{3}}{2} & \frac{1}{2} \end{pmatrix}, & (3, 4) &= \begin{pmatrix} 1 & 0 & 0 & 0 & 0 \\ 0 & 1 & 0 & 0 & 0 \\ 0 & 0 & -\frac{1}{3} & \frac{2\sqrt{2}}{3} & 0 \\ 0 & 0 & \frac{2\sqrt{2}}{3} & \frac{1}{3} & 0 \\ 0 & 0 & 0 & 0 & 1 \end{pmatrix}, \\ (4, 5) &= \begin{pmatrix} 1 & 0 & 0 & 0 & 0 \\ 0 & -\frac{1}{4} & \frac{\sqrt{15}}{4} & 0 & 0 \\ 0 & \frac{\sqrt{15}}{4} & \frac{1}{4} & 0 & 0 \\ 0 & 0 & 0 & 1 & 0 \\ 0 & 0 & 0 & 0 & 1 \end{pmatrix}, & (5, 6) &= \begin{pmatrix} -\frac{1}{5} & \frac{2\sqrt{6}}{5} & 0 & 0 & 0 \\ \frac{2\sqrt{6}}{5} & \frac{1}{5} & 0 & 0 & 0 \\ 0 & 0 & 1 & 0 & 0 \\ 0 & 0 & 0 & 1 & 0 \\ 0 & 0 & 0 & 0 & 1 \end{pmatrix}. \end{aligned} \quad (6)$$

Having access to the matrix representations of all adjacent transpositions allows us to calculate that for any permutation  $\sigma \in S_n$  in principal and there are classical or quantum  $S_n$ -Fast Fourier Transform designed for this task [10, 11].

**Definition I.3.** Given an arbitrarily partition/Young diagram  $\lambda \vdash n$ . A permutation  $\sigma \in S_n$  is of *cycle type*  $\lambda$  if it is decomposed into cycles of lengths  $\lambda_1, \dots, \lambda_r$ .

For instance,  $\sigma = (134)(56) \in S_6$  is of the type  $\lambda = (3, 2, 1)$ . The trivial permutation  $\text{id} \in S_n$  is of type  $(1, \dots, 1)$ . Transpositions or SWAPs  $(i, j)$  are just 2-cycles. Products of transpositions like  $(i, j)(k, l) \cdots (s, t)$  are of the type  $(2, 2, \dots, 2, 1, \dots, 1)$ .

**Definition I.4.** Let  $p(n)$  denotes the *number of partitions of  $n$* . Then it equals the number of all inequivalent  $S_n$  irreps, as well as the number of possible cycle types in  $S_n$ . Analogously, we define  $p(n, d)$  as the *number of partitions of  $n$  with at most  $d$  parts*, i.e., the number of all Young diagrams of  $n$  boxes with at most  $d$  rows.

We encounter  $p(n)$  and  $p(n, d)$  in [12] when arguing the difficulty of computing frame potential with the presence of  $\text{SU}(d)$  symmetry and studying the locality required to achieve arbitrary  $k$ -design. They appear later when we turn to bound the so-called out-of-time-ordered correlation (OTOC) in Section III B. It is due to the celebrated work of Ramanujan and Hardy [13] and Uspensky [14] that

$$p(n) \sim \frac{e^{\sqrt{\pi^2 2n/3}}}{4n\sqrt{3}}, n \rightarrow \infty \quad (7)$$

with further researches [15, 16] and useful bounds on  $p(n)$  being found later such as [17, 18]

$$\frac{e^{2\sqrt{n}}}{an} < p(n) < e^{b\sqrt{n}}. \quad (8)$$

If  $d = 2$ ,  $p(n, 2) = \lfloor \frac{n}{2} \rfloor + 1$ . However, there is no closed formulas for these partition functions in general.

**Proposition I.5.** Let  $c_\mu \in \mathbb{C}[S]$  be the sum of all  $\sigma \in S_n$  with cycle type  $\mu$ . Consider all possible Young diagrams of size  $n$ , the collection  $\{c_\mu\}_{\mu \vdash n}$  forms a basis for the *center*  $Z(\mathbb{C}[S_n])$  consisting of all elements that commute with  $\mathbb{C}[S_n]$ .

It is by definition that  $c_\mu$  commutes with any  $\sigma \in S_n$ . By Wedderburn theorem [2, 3], its matrix representation, still denoted by  $c_\mu$  for simplicity, under any  $S_n$  irrep  $S^\lambda$  is just a scalar. As a result, the representation of  $Z(\mathbb{C}[S_n])$  consists of scalars matrices within any  $S_n$  irrep. Being a basis of  $Z(\mathbb{C}[S_n])$  means being a basis capable of spanning all scalars matrices, called *relative phase factors* when we study  $k$ -design with symmetry, respecting the direct sum  $\bigoplus S^\lambda$  of all inequivalent  $S_n$  irreps. The diagonal phase matrix  $e^{-ic_\mu}$  helps to replenish relative phase factors for the group of  $\text{SU}(d)$  symmetric unitaries.

Besides the basis  $\{c_\mu\}$  defined above, we still have the following two kinds of center bases:

**Theorem I.6.** *The following two collections also constitute bases for  $Z(\mathbb{C}[S_n])$ :*

1. *Let us consider the  $S_n$  group character*

$$\chi_\lambda(\sigma) = \text{tr}_\lambda \sigma \quad (9)$$

*defined by taking the trace of  $\sigma \in S_n$  restricted to the irrep  $S^\lambda$ , then*

$$\Pi_\mu := \frac{\dim S^\mu}{n!} \sum_{\sigma \in S_n} \bar{\chi}_\mu(\sigma) \sigma = \begin{cases} I, & \mu = \lambda \\ 0, & \text{otherwise} \end{cases}. \quad (10)$$

*The collection  $\{\Pi_\mu\}$  is an orthonormal basis.*

2. *Let us consider the YJM-elements  $X_i$ . For any  $\mu = (\mu_1, \dots, \mu_r) \vdash n$ , we set*

$$X_\mu = \sum_{2 \leq i_1 \neq i_2 \neq \dots \neq i_r \leq n} X_{i_1}^{\mu_1-1} X_{i_2}^{\mu_2-1} \dots X_{i_r}^{\mu_r-1} \quad (11)$$

*The collection  $\{X_\mu\}$  is also a basis for  $Z(\mathbb{C}[S_n])$  [4, 7, 8].*

For the purpose of efficient implementation into quantum circuits, we would always construct center basis elements through  $X_\mu$  because encoding  $c_\mu$  requires to sum over all permutations of a given cycle type  $\mu$  and encoding  $\Pi_\mu$  even needs doing that over the whole symmetric group with  $n!$  elements. However, it should be noted that for either cases, building a complete basis finally employs non-local operator acting on all qudits.

In Section III B and III E, we also need to compute the character  $\chi_\lambda(\sigma)$  explicitly for some  $\sigma \in S_n$ , so we briefly introduce the method here. We first present the following proposition:

**Proposition I.7.** For any  $\sigma \in S_n$ ,  $\chi_\lambda(\sigma) \in \mathbb{Z}$ . That is,  $S_n$  characters are integer-valued.

One can prove a bunch of similar facts by Galois Theory for general finite groups. In our case, we simply note that there is the so-called *Young's natural representation* which is a *non-unitary* representation of  $S^\lambda$  under which each  $\sigma$  is expressed as matrices with integer entries [2]. As trace is invariant under matrix similarity,  $\chi_\lambda(\sigma) = \text{tr}_\lambda \sigma \in \mathbb{Z}$  in general.

It is also well known that permutations  $\sigma, \sigma'$  with the same cycle type are conjugate to each other, so  $\chi_\lambda(\sigma) = \chi_\lambda(\sigma')$  and thus we only concern the value of  $\chi_\lambda$  for a given cycle type  $\mu$ . The so-called *Frobenius character formula* [3] expresses  $S_n$  character values as coefficients of a power series. The coefficient can be compute by, for instance, contour integrals with residue theorem in principal. However, closed formulas are only seen for very few simple cases [19, 20]. For instance, characters for 2-cycles (transpositions/SWAPs) equals

$$\frac{\chi_\lambda(i, j)}{\dim S^\lambda} = \frac{2}{n(n-1)} \sum_i \left( \binom{\lambda_i}{2} - \binom{\lambda'_i}{2} \right) = \frac{1}{n(n-1)} \sum_i [(\lambda_i - 1)(\lambda_i - 1 + i) - i(i - 1)], \quad (12)$$

where  $\lambda'$  denotes the conjugate of  $\lambda$ , e.g.,

$$\lambda = \begin{array}{|c|c|c|c|} \hline & & & \\ \hline & & & \\ \hline & & & \\ \hline & & & \\ \hline \end{array} \quad \lambda' = \begin{array}{|c|c|c|} \hline & & \\ \hline & & \\ \hline & & \\ \hline & & \\ \hline \end{array}$$

If  $\lambda_i < 2$ , the corresponding binomial coefficient is set to zero.

Let us relate the above character formula to some techniques involving YJM-elements. Restricted to any irrep  $S^\lambda$ , we can associate the following invariants:

$$P_l = \left( \sum_i X_i \right)^l, l = 1, 2, \dots \quad (13)$$

where  $\sum_i X_i$  is the summation of all YJM-elements. Let us check its matrix form under Young basis  $|\alpha_T\rangle$ :

$$\left( \sum_i X_i \right) |\alpha_T\rangle = \sum_i \alpha_T(i) |\alpha_T\rangle \quad (14)$$

with  $\alpha_T$  being the content vector. Obviously, for any fixed Young diagram  $\lambda$ , the sum of all components of any of its content vector  $\alpha_T$  is simply equal to the sum of all coordinate differences, and we denote it as  $\alpha_\lambda$ . Then

$$P_l |\alpha_T\rangle = (\alpha_\lambda)^l |\alpha_T\rangle \quad (15)$$

for all standard tableaux/Young basis vectors of the Young diagram  $\lambda$ .

Let  $\text{tr}_\lambda$  denote by taking trace within  $S^\lambda$  (it is actually just the  $S_n$  character in Eq.(9)). When  $l = 1$ , we note that

$$\alpha_\lambda = \frac{\text{tr}_\lambda(P_l)}{\dim S^\lambda} = \frac{\text{tr}_\lambda \sum_i X_i}{\dim S^\lambda} = \frac{n(n-1)}{2} \frac{\text{tr}_\lambda(i, j)}{\dim S^\lambda} = \frac{n(n-1)}{2} \frac{\chi_\lambda(i, j)}{\dim S^\lambda} \quad (16)$$

which gives another way to compute the character value of 2-cycles by summing all components from the content vector. The method using YJM-elements and content vectors to express general  $S_n$  characters can be found in [21].

**Definition I.8.** Given two partitions  $\lambda = (\lambda_i), \mu = (\mu_i) \vdash n$ . We say that  $\lambda$  *dominates*  $\mu$ , denoted by  $\lambda \triangleright \mu$ , if for all  $j > 0$ ,  $\sum_i^j \lambda_i \geq \sum_i^j \mu_i$ .

For instance, we have

$$(6) \triangleright (5, 1) \triangleright (4, 2) \triangleright (4, 1^2) \quad (17)$$

where  $(4, 1^2)$  is the abbreviation of  $(4, 1, 1)$ . The dominance relation is not *totally ordered*, e.g., we cannot compare  $(4, 1^2)$  and  $(3, 3)$ . However, in the case of qubits ( $d = 2$ ), where we focus on two-row Young diagrams by Schur-Weyl duality introduced in the following, partitions  $\lambda = (\lambda_1, \lambda_2)$  with  $\lambda_1 \geq \lambda_2$  clearly give rise to a total ordering.

**Lemma I.9.** For any two partitions unequal  $\lambda, \mu \vdash n$ , if  $\lambda \triangleright \mu$ , then  $\alpha_\lambda > \alpha_\mu$ .

*Proof.* We prove the lemma by induction. Suppose the statement holds for  $n - 1$ . Given unequal  $\lambda, \mu \vdash n$  with  $\lambda \triangleright \mu$ , there should be some  $i$  such that  $\lambda_i > \mu_i$  as the lengths of  $i$ th rows of  $\lambda$  and  $\mu$  respectively. If  $\lambda_i > \lambda_{i+1}$  and  $\mu_i > \mu_{i+1}$ , then we discard the RHS boxes on the  $i$ th rows of  $\lambda$  and  $\mu$ . The resultant Young diagrams, denoted by  $\lambda'$  and  $\mu'$  still satisfy the relation  $\lambda' \triangleright \mu'$ . Then by induction hypothesis,  $\alpha_{\lambda'} > \alpha_{\mu'}$ . On the other hand, the content of the discarded box from  $\lambda$  is larger than that from  $\mu$  by definition, hence we conclude that  $\alpha_\lambda > \alpha_\mu$ .

Suppose  $\lambda_i = \lambda_{i+1} = \dots = \lambda_r$  or  $\mu_i = \mu_{i+1} = \dots = \mu_s$ . Then we are only allowed to discard the RHS boxes of  $\lambda_r, \mu_s$  to ensure that  $\lambda'$  and  $\mu'$  are well-defined Young diagrams. Even when  $r \neq s$ , the dominance relation still holds because  $\lambda_r > \mu_s$ . By the same argument as above, we complete the proof.  $\square$

By Eq.(16), the above lemma says that  $\frac{\chi_\lambda(1,2)}{\dim S^\lambda}$  is strictly increasing with respect to the dominance order of  $\lambda$ . Lots of counterexamples occurs when this order fails to hold: e.g.,  $(3, 3)$  and  $(4, 1^2)$ .

Let us end this subsection with some explicit analysis on the dimension of  $S_n$  irreps of two-row Young diagram. In this circumstance, the hook length formula in I.1 can be further simplified as [2, 19]:

$$\dim S^\lambda = d_\lambda = \binom{n}{r} - \binom{n}{r-1} = \frac{n-2r+1}{n-r+1} \binom{n}{r}. \quad (18)$$

For binomial coefficient, we have another two useful bounds (assume  $n = 2m$ ) [22]:

$$\frac{2^n}{\sqrt{\pi(\frac{n}{2} + \frac{1}{3})}} \leq \binom{n}{n/2} \leq \frac{2^n}{\sqrt{\pi(\frac{n}{2} + \frac{1}{4})}}, \quad e^{-(\frac{n}{2}-r)^2/(n-r+1)} \leq \binom{n}{r} / \binom{n}{\frac{n}{2}} \leq e^{-(\frac{n}{2}-r)^2/(n-r)}. \quad (19)$$

Therefore, the ratio of  $\dim S^\lambda$  to the dimension of the entire Hilbert space is

$$\frac{1}{\sqrt{\pi(\frac{n}{2} + \frac{1}{3})}} \frac{n-2r+1}{n-r+1} \binom{n}{r} / \binom{n}{\frac{n}{2}} \leq \frac{\dim S^\lambda}{2^n} = \frac{1}{2^n} \frac{n-2r+1}{n-r+1} \binom{n}{r} \leq \frac{1}{\sqrt{\pi(\frac{n}{2} + \frac{1}{4})}} \frac{n-2r+1}{n-r+1} \binom{n}{r} / \binom{n}{\frac{n}{2}}. \quad (20)$$

A lower bound for general  $d$ -row Young diagram is also useful [23, 24]: suppose the first row  $\lambda_1, \lambda'_1$  of  $\lambda$  and its conjugate is upper bounded by  $\frac{n}{\alpha}$  for some  $\alpha > 1$ . Then

$$\dim S^\lambda \geq \frac{\alpha^n}{n^{d(d+2)/2}}. \quad (21)$$

We will use these results for specific cases in Section III B and III D.

### B. Schur-Weyl Duality and CQA Architecture

We now make a brief review on  $S_n$ -Convolutional Quantum Alternating Ansätze and the group CQA proposed in [5] which is proved to form the exact  $k$ -design with  $SU(d)$  symmetry and motivates the definition of CQA ensemble in approximating unitary  $k$ -design.

In quantum systems there is a discrete set of translations corresponding to permuting the qudits as well as a continuous notion of translation corresponding to spatial rotations by elements of  $SU(d)$ . To be precise, let  $V$  be a  $d$ -dimensional complex Hilbert space with orthonormal basis  $\{e_1, \dots, e_d\}$ . The tensor product space  $V^{\otimes n}$  admits two natural representations: the *tensor product representation*  $\pi_{SU(d)}$  of  $SU(d)$  acting as

$$\pi_{SU(d)}(g)(e_{i_1} \otimes \dots \otimes e_{i_n}) := g \cdot e_{i_1} \otimes \dots \otimes g \cdot e_{i_n}, \quad (22)$$

where  $g \cdot e_{i_k}$  is the fundamental representation of  $SU(d)$ , and the *permutation representation*  $\pi_{S_n}$  of  $S_n$  acting as

$$\pi_{S_n}(\sigma)(e_{i_1} \otimes \dots \otimes e_{i_n}) := e_{i_{\sigma^{-1}(1)}} \otimes \dots \otimes e_{i_{\sigma^{-1}(n)}}. \quad (23)$$

We treat  $H = V^{\otimes n}$  as the Hilbert space of an  $n$ -qudit system. The so-called Schur-Weyl duality says that the action of  $SU(d)$  and  $S_n$  on  $V^{\otimes n}$  jointly decompose the space into irreducible representations of both groups in the form

$$V^{\otimes n} = \bigoplus_{\lambda} W_{\lambda} \otimes S^{\lambda}. \quad (24)$$

Recall that  $\lambda$  denotes a Young diagram. It corresponds not only to a unique  $S_n$  irrep  $S^{\lambda}$ , but also an  $SU(d)$  irrep  $W_{\lambda}$  in this setting [3, 4].

It should be noted that within an  $n$ -qudit system, only irreps corresponding to  $\lambda$  ranging over *Young diagrams of size  $n$  with at most  $d$  rows* can be found in the decomposition. Consequently,

$$\pi_{SU(d)} \cong \bigoplus_{\mu} W_{\mu} \otimes 1_{m_{SU(d), \mu}}, \quad \pi_{S_n} \cong \bigoplus_{\lambda} 1_{m_{S_n, \lambda}} \otimes S^{\lambda}, \quad (25)$$

where  $m_{SU(d), \mu} = \dim S^{\mu}$  and  $m_{S_n, \lambda} = \dim W_{\lambda}$ .

Given any operator  $A$  acting on the system, being  $SU(d)$  symmetric/invariant means

$$\pi_{SU(d)}(g)A = A\pi_{SU(d)}(g) \text{ or } g^{\otimes n}A = Ag^{\otimes n}. \quad (26)$$

One can check Eq.(22) and (23) that these permutation actions clearly commute with  $g^{\otimes n}$ . Furthermore Schur-Weyl duality, as well as double commutant theorem [3, 4], confirms that  $SU(d)$  symmetric operators are exactly built from permutations in the symmetric group  $S_n$ . That is, they can be written as linear combinations, like  $\sum c_i \sigma_i$ , of permutations.

Even decomposing the entire space into  $SU(d)$  irreps is quite conventional in physics. Quantum states living in these subspaces are actually permutation-invariant or  $S_n$  symmetric. Since our focuses are quantum circuits with  $SU(d)$  symmetry, we should decompose the entire Hilbert space with respect to  $S_n$  irreps (see [4, 5, 25] for more details). As a reminder, even the entire Hilbert space is decomposed into smaller subspaces, there is no reason to expect that related problems, like searching the ground state energy of  $SU(d)$  symmetric Hamiltonian or construing  $SU(d)$  symmetric random quantum circuit, would become easier. There are two reasons in general,

- (a) There are various inequivalent  $S_n$  irreps from the decomposition to deal with, and the total number is  $p(n, d)$ , which scales at most super-polynomially (Eq.(7)) with  $n$  and has no closed form to evaluate.
- (b) Even for qubits with  $d = 2$ , using the hook length formula from Definition I.1, we know that (cf.Eq.(18))

$$\dim S^{(m, m)} = \frac{(2m)!}{(m+1)!m!} = \frac{2^m}{m+1} \prod_{k=1}^m \frac{2k-1}{k} > \frac{2^m}{m+1} \quad (27)$$

for the  $S_n$  irrep of Young diagram  $\lambda = (m, m)$  on a  $2m$ -qubit system. One can find other examples with exponential large subspaces respecting the  $SU(d)$  symmetry [24], which still cause difficulties when approaching the problem.

We now introduce the mathematical definition of  $S_n$ -CQA ansatz:

**Definition I.10.** The  $S_n$ -CQA ansatz is defined as

$$\dots \exp(-i \sum_{k,l} \beta_{kl} X_k X_l) \exp(-i\gamma H_S) \exp(-i \sum_{k,l} \beta'_{kl} X_k X_l) \exp(-i\gamma' H_S) \dots, \quad (28)$$

where  $X_k X_l$  are product of YJM-elements, which is 4-local and still diagonal under Young basis (see Example.(4)). The Hamiltonian  $H_S$  is defined as the summation of adjacent transpositions  $\sum_{i=1}^{n-1} (i, i+1)$ .

Moreover, let us define the group generated by alternating exponentials from Eq.(28)

$$\text{CQA} = \left\langle \exp(-i \sum_{k,l} \beta_{kl} X_k X_l), \quad \exp(-i\gamma H_S) \right\rangle. \quad (29)$$

Obviously, CQA is contained in the *group of SU(d) symmetric unitaries*. To define this group, let  $U(S^\lambda)$  denote the unitary group acting on the representation space  $S^\lambda$ , i.e.,  $U(S^\lambda) \cong U(\dim S^\lambda)$ . A typical element  $g$  from the group of  $SU(d)$  symmetric unitaries is then a collection of unitaries:

$$g = \bigoplus_{\lambda} U_{\lambda}^{\oplus m_{S_n, \lambda}}, \quad (30)$$

where  $U_{\lambda} \in U(S^\lambda)$  and  $\lambda$  ranges over all Young diagrams of size  $n$  with at most  $d$  rows. For simplicity, we omit the multiplicities and denote this group by

$$\mathcal{H}_{\times} = U(\bigoplus_{\lambda} S^{\lambda}). \quad (31)$$

Equivalent copies of  $S_n$  irreps poses no more difficulties in computing  $k$ -fold channel/ $k$ th moment operator twirled through  $SU(d)$  symmetric unitaries [12], but it is one of the obstacles when we calculate frame potential/dimension of the commutant of  $\mathcal{H}_{\times} = U(\bigoplus_{\lambda} S^{\lambda})$  in Section II C.

On the other hand, by restricting the phase factors to be 1 on each  $S^\lambda$ , we have the special unitary group  $SU(S^\lambda)$  as well as  $S\mathcal{H}_{\times} = SU(\bigoplus_{\lambda} S^{\lambda})$  consisting of  $SU(d)$  symmetric unitaries with unit determinant on each  $S_n$  irrep block, i.e., unitaries with trivial relative phase factors with respect to. each irrep sector. It is proved in [5] that

$$S\mathcal{H}_{\times} \subsetneq \text{CQA} \subsetneq \mathcal{H}_{\times} \quad (32)$$

which establishes a theoretical guarantee in searching the ground state energy of  $SU(d)$  symmetric frustrated 2D Heisenberg model using  $S_n$ -CQA ansatz because relative phase factors can be ignored when we measure the expectation value in the experiment.

With the focus on locality, 2-local unitaries are proved to be universal to common quantum circuits [26], as well as approximate polynomial-designs [27, 28]. After imposing the  $SU(d)$  symmetry however, it is shown in [29–31] that when  $d \geq 3$ , 2-local  $SU(d)$  symmetric unitaries cannot even generate  $S\mathcal{H}_{\times}$ . The group CQA accomplishes this task by incorporating 4-local  $SU(d)$  symmetric unitaries, and we present in the following sections the mathematical details on using CQA to establish unitary  $k$ -design under  $SU(d)$  symmetry in both exact and approximate senses.

### C. Useful Properties on Quantum Entropies

We note that the intuitive treatments relating the mutual information, relative entropy, and operator distance measure can be made rigorous. We refer the curious readers to a rather systematic treatment presented in Ch.5 of [32]. The key question in the setting presented in Section II is the relation between the mutual information between the register  $R$  and  $\bar{B}$ ,  $I(R : \bar{B})$  and the (trace) norm distance between  $\rho_{R\bar{B}}$  and  $\sigma_{R\bar{B}}$ . We first review some basic definitions. Assuming the Hilbert space is a composite system  $\mathcal{H} = \mathcal{H}_A \otimes \mathcal{H}_{\bar{A}}$  and a pure state  $\psi$  defined on the Hilbert space. Its Von Neumann entropy can be uniquely given by

$$S(\rho_A) = -\text{Tr}[\rho_A \log \rho_A] \quad (33)$$

Where  $\rho_A \equiv \text{Tr}_{\bar{A}}[\psi]$  the partial trace over the subsystem  $A$  and  $S(\rho_A) = S(\rho_{\bar{A}})$  as the system is bipartite. It is important to note that although the mathematical notion of Von Neumann entropy is well-defined as long as it is given a positive semi-definite operator acting on  $\mathcal{H}$ , the physical meaning of entropy of some quantum states might not exist if the system is multipartite or the quantum state is not pure in  $\mathcal{H}$ , which is still a frontier in quantum information research. Another useful quantity is called the quantum relative entropy given two density matrix  $\rho, \sigma$  such that the image of  $\rho$  lies inside that of  $\sigma$

$$D(\rho||\sigma) \equiv \text{Tr}[\rho \log \rho - \rho \log \sigma] \quad (34)$$



Otherwise  $D(\rho\|\sigma) = \infty$ . In the setting mentioned in Section II of the main text with  $\rho_{R\cup\bar{B}}$  and  $\sigma_{R\cup\bar{B}} \equiv \rho_R \otimes \rho_{\bar{B}}$  with the subscript denoting the reduced density matrices after partial trace

$$\begin{aligned}
D(\rho_{R\cup\bar{B}}\|\sigma_{R\cup\bar{B}}) &= D(\rho_{R\cup\bar{B}}\|\rho_R \otimes \rho_{\bar{B}}) \\
&= \text{Tr} \{ \rho_{R\cup\bar{B}} \log(\rho_{R\cup\bar{B}}) - \rho_{R\cup\bar{B}} \log(\rho_R \otimes I) - \rho_{R\cup\bar{B}} \log(I \otimes \rho_{\bar{B}}) \} \\
&= \text{Tr}[\rho_{R\cup\bar{B}} \log(\rho_{R\cup\bar{B}})] - \sum_{ij} \lambda_{ij} \log(r_i) |i, j\rangle \langle i, j| - \lambda_{ij} \log(\bar{b}_i) |i, j\rangle \langle i, j| \\
&= S(\rho_{R\cup\bar{B}}) - S(\rho_R) - S(\rho_{\bar{B}}) \\
&= I(R : \bar{B})
\end{aligned} \tag{35}$$

Where the second equality uses the fact that

$$\text{span} \{ \ker(\rho_R \otimes I), \ker(I \otimes \rho_{\bar{B}}) \} = \ker(\rho_R \otimes \rho_{\bar{B}}) \subset \ker \rho_{R\cup\bar{B}} \tag{36}$$

Hence, the relative entropy formula is used. The third equality assumes the Schdmit decomposition of  $\rho_{R\cup\bar{B}}$

$$\rho_{R\cup\bar{B}} = \sum_n \sigma_n |n\rangle \langle n|_{R\cup\bar{B}} = \sum_{ij} \lambda_{ij} |i, j\rangle \langle i, j| \tag{37}$$

So that

$$\rho_R = \sum_i \left( \sum_j \lambda_{ij} \right) |i\rangle \langle i|_R \equiv \sum_i r_i |i\rangle \langle i|_R \tag{38}$$

Similarly for  $\rho_{\bar{B}}$ . We note the following properties of quantum entropy

- $S(\rho \otimes \sigma) = S(\rho) + S(\sigma)$
- $D(\rho_0 \otimes \rho_1 \| \sigma_0 \otimes \sigma_1) = D(\rho_0 \| \sigma_0) + D(\rho_1 \| \sigma_1)$

Using the above property, we could also rewrite  $D(\rho_{R\cup\bar{B}}\|\rho_R \otimes \rho_{\bar{B}}) = I(R : \bar{B}) = |S(\rho_R \otimes \rho_{\bar{B}}) - S(\rho_{R\cup\bar{B}})|$ . Mutual information can be thought of as a useful criterion to determine how much information is lost. Alternatively, if we wish to express in terms of fidelity, which is defined in the average case [33], it is shown that the saturation of mutual information  $I(R : B \cup \text{MEM})$  is a necessary condition to obtain the optimal recovery. Infidelity measures, such as the ones used in [34, 35], often involve the purified distance  $P(\rho, \sigma)$  which is related with the trace norm distance

$$\frac{1}{2} \|\rho - \sigma\|_1 \leq P(\rho, \sigma) \leq \sqrt{2 \|\rho - \sigma\|_1} \tag{39}$$

It turns out that the smallness of the mutual information  $I(R : \bar{B})$  is a necessary condition for the decoupling in terms of the trace norm distance and purified distance. For a pathological review, given two arbitrary density states  $\rho, \sigma$ ,

$$D(\rho\|\sigma) \geq 0, \quad \text{and } D(\rho\|\sigma) = 0 \text{ if and only if } \rho = \sigma \tag{40}$$

This inequality is known as the *Klein inequality*. First note that when  $\rho_{R\cup\bar{B}}$  is completely decoupled as a product state, it is easy to see that  $I(R : \bar{B}) = 0$  and Eq.(39) trivially vanishes, while A sense of continuity exists for the mutual information in this case, known as the *Fannes-Audenaert inequality*. Let

$$\delta = \frac{1}{2} \|\rho_{R\cup\bar{B}} - \rho_R \otimes \rho_{\bar{B}}\|_1 \tag{41}$$

it holds that

$$I(R : \bar{B}) \leq \delta \log(d_{R\cup\bar{B}} - 1) + H(\delta, 1 - \delta) \leq \delta \log(d_{R\cup\bar{B}}) + H(\delta, 1 - \delta) \tag{42}$$

If  $\delta$  is assumed to be sufficiently small, the classical Shannon entropy

$$H(\delta, 1 - \delta) = -\delta \log(\delta) - (1 - \delta) \log(1 - \delta) \approx \delta(1 - \delta + \log(\frac{1}{\delta})) \leq \delta \log(\frac{e}{\delta}) \tag{43}$$



In this regime, we have the bound

$$I(R : \bar{B}) \leq \delta \log\left(\frac{e d_{R \cup \bar{B}}}{\delta}\right) \quad (44)$$

As long as  $\frac{1}{\delta} = o(n)$  where  $n$  is the total number of physical qudits, the expression  $\delta \log\left(\frac{e d_{R \cup \bar{B}}}{\delta}\right)$  decays asymptotically to 0. Hence, there must exist  $n$  such that,  $\forall \epsilon > 0$ ,  $\delta \log\left(\frac{e d_{R \cup \bar{B}}}{\delta}\right) < \epsilon$ . Hence the continuity relation establishes that the smallness of mutual information is a necessary condition to a good decoupling via trace norm distance or by Eq.(39) the purified distance. Conversely, by the quantum Pinsker inequality, we have that

$$2\delta^2 \leq I(R : \bar{B}) \leq \delta \log\left(\frac{e d_{R \cup \bar{B}}}{\delta}\right) \quad (45)$$

So that the (asymptotic) smallness of mutual information to the  $1/4$  power can be regarded as a sufficient condition to conclude decoupling in trace distance and purified distance.

## II. CHARACTERIZING RANDOM CIRCUIT DESIGNS BY COMMUTANT UNDER GROUP REPRESENTATION

To study whether an ensemble forms a  $k$ -design in both exact and approximate sense, there are two deeply related two approaches: computing the frame potential of the ensemble, or analyzing the commutant algebra in the representation space. In this section, we illustrate these strategies in details, show their relationship mathematically (Proposition II.7) and finally move to determine the commutant of the group  $U(\bigoplus_{\lambda} S^{\lambda})$  of  $SU(d)$  symmetric unitaries (Theorem II.8) and discuss the limitation of computing frame potential for Haar measure with the presence of  $SU(d)$  symmetry. These perspectives connect various approaches to understand unitary design such as using the tensor product expander [27, 28, 36, 37],  $k$ th moment operators channel [38, 39] or frame potential [40–45].

### A. Quantum $k$ -fold Channel

We first give definition of  $k$ -fold channel [39, 43] or  $k$ th-moment operator of a compact group  $G$ .

**Definition II.1.** Given a compact group  $G$  with the Haar measure  $\mu$  and a unitary representation  $\rho$  on the concerned Hilbert space  $H$ . For any operator  $M \in \text{End}(H^{\otimes k})$ , the  $k$ -fold channel twirled over  $G$  acting on  $M$  is:

$$T_k^G(M) = \int_G d\mu(g) \rho^{\otimes k}(g) M (\rho^{\otimes k}(g))^{\dagger} = \int_G dU U^{\otimes k} M U^{\dagger \otimes k}, \quad (46)$$

where we denote matrix representations of group elements simply by  $U, V$  on the RHS of the above identity. Despite its integral form, as a super-operator,  $T_k^G$  is merely a linear map acting on  $\text{End}(H^{\otimes k})$  and can be reformulated as the  $k$ th moment operator:

$$T_k^G = \int_G U^{\otimes k} \otimes \bar{U}^{\otimes k} dU. \quad (47)$$

Replacing  $G$  by an arbitrary ensemble  $\mathcal{E}$  with a precised measure  $\nu$ ,  $T_k^{\mathcal{E}}$  can be defined similarly when studying approximate  $k$ -design.

Since Haar measure is left-invariant,  $T_k(M)$  commutes with the  $k$ -fold tensor product representation  $\rho^{\otimes k}$  of  $G$ :

$$V^{\otimes k} T_k^G(M) V^{\dagger \otimes k} = \int_G (VU)^{\otimes k} M (UV)^{\dagger \otimes k} dU = T_k^G(M). \quad (48)$$

To put this identity in another way,  $T_k^G$  projects  $M$  into the *commutant algebra*:

$$\text{Comm}_k(G) := \{M \in \text{End}(H^{\otimes k}); U^{\otimes k} M = M U^{\otimes k}\}, \quad (49)$$

i.e., the subspace of all operators that commute with the tensor product representation  $\rho^{\otimes k}$ . The operator  $T_k^G$  is surjective since if  $M \in \text{Comm}(M)$ ,  $T_k^G(M) = M$  by definition. It is thus a *projector* from  $\text{End}(H^{\otimes k})$  onto  $\text{Comm}_k(G)$ . Then we have the following identity by either the invariance of Haar measure or the property of projector:

$$T_k^G(T_k^G(M)) = \int_G dU dV (VU)^{\otimes k} M (UV)^{\dagger \otimes k} = \int_G d(UV) (VU)^{\otimes k} M (UV)^{\dagger \otimes k} = T_k^G(M), \quad (50)$$

which further implies that  $T_k^G$  has eigenvalues either 0 or 1.

For the common case of unitary designs without any assumption on symmetries of the system,  $G = \text{U}(d^n) \equiv \text{U}(N)$  with  $\rho^{\otimes k}$  is given by the  $k$ -fold tensor products of fundamental representation of  $\text{U}(N)$ . Therefore, by the Schur-Weyl duality and double commutant theorem (cf. Schur-Weyl duality on an  $n$ -qudit system), the commutant algebra is isomorphic to the representation of the symmetric group algebra  $\mathbb{C}[S_k]$  which permutes elements from  $H^{\otimes k}$ . With the presence of  $\text{SU}(d)$  symmetry, the group of interests is replaced by  $\text{U}(\bigoplus_\lambda S^\lambda)$  defined in Section IB. We particularly denote by  $T_k^{\text{Haar}}$  the  $k$ -fold channel twirled over the group  $\text{U}(\bigoplus_\lambda S^\lambda)$  respecting symmetry.

### B. Approximate $k$ -design and Random Walk on Group

The viewpoint that  $T_k^G$  is a projector to the commutant of  $G$  offers a convenient characterization for unitary  $k$ -design, with the usual definition [27, 39] (also see [36, 37, 43] for several alternative definitions and comparison on operator norms [46, 47]):

**Definition II.2.** For  $\epsilon > 0$ , an ensemble of unitaries  $\mathcal{E}$  is an  $\epsilon$ -approximate  $k$ -design if the diamond norm of the difference of  $k$ -fold channels satisfies

$$\|T_k^\mathcal{E} - T_k^G\|_\diamond \leq \epsilon. \quad (51)$$

**Lemma II.3.** Recall that  $T_k^\mathcal{E}$  is merely a linear map on  $\text{End}(H^{\otimes k})$ . With further conditions on the measure  $\nu$  of  $\mathcal{E}$  being specified,  $T_k^\mathcal{E}$  satisfies the following properties:

1. If  $\nu$  is left-invariant, then  $T_k^\mathcal{E}$  becomes a projector onto  $\text{Comm}_k(\mathcal{E})$ .
2. If  $\nu$  is invariant under inverse, i.e.,

$$\int_{\mathcal{E}} d\nu(g) f(g^{-1}) = \int_{\mathcal{E}} d\nu(g) f(g) \quad (52)$$

for any function  $f$  defined on  $\mathcal{E}$ , then  $T_k^\mathcal{E}$  is Hermitian.

*Epecially when  $\mathcal{E}$  is taken as a certain compact subgroup of  $G$  with the restricted Haar measure, then both of the above properties hold.*

We have seen the first property in Section IIA. The second property is also straightforward by using  $U^{-1} = U^\dagger$  for unitary representation:

$$T_k^{\mathcal{E}\dagger} = \int_S V^{\dagger \otimes k} \bar{V}^{\dagger \otimes k} dV = \int_S (V^{-1})^{\otimes k} M (\bar{V}^{-1})^{\otimes k} dV = T_k^\mathcal{E}. \quad (53)$$

Most ensembles encountered in literature like [27, 28, 39], as well as our CQA ensemble defined in [12], produces Hermitian  $k$ -fold channel which can be diagonalized with operator norm equal to its largest abstract value of its eigenvalues. This fact is used throughout the context in proving our results. The concept of frame potential works more general for non-Hermitian case, which we also use in [12] to demonstrate that general ensembles approximating  $\text{SU}(d)$  symmetric  $k$ -design with arbitrary large  $k$  can never admit a constant locality.

Besides, applying the bi-invariance of Haar measure and Fubini theorem, which holds for well-behaved measures likes restricted Haar measures on compact subgroups, we note that  $T_k^\mathcal{E}$  commutes with  $T_k^G$ :

$$\begin{aligned} T_k^\mathcal{E} T_k^G(M) &= \int_{\mathcal{E}} \int_G V^{\otimes k} U^{\otimes k} M U^{\dagger \otimes k} V^{\dagger \otimes k} dU dV = \int_G U^{\otimes k} M U^{\dagger \otimes k} dU = T_k^G(M) \\ &= \int_{\mathcal{E}} \int_G U^{\otimes k} V^{\otimes k} M V^{\dagger \otimes k} U^{\dagger \otimes k} dU dV \\ &= \int_G \int_{\mathcal{E}} U^{\otimes k} V^{\otimes k} M V^{\dagger \otimes k} U^{\dagger \otimes k} dV dU = T_k^G T_k^\mathcal{E}(M). \end{aligned} \quad (54)$$

By Lemma II.3,  $T_k^G$  is always diagonalizable. Assume  $T_k^\mathcal{E}$  is Hermitian and hence diagonalizable, then they can be *simultaneously diagonalized*, e.g.,

$$T_k^G = \begin{pmatrix} 1 & & & \\ & 1 & & \\ & & 0 & \\ & & & 0 \end{pmatrix}, \quad T_k^\mathcal{E} = \begin{pmatrix} 1 & & & \\ & 1 & & \\ & & \lambda & \\ & & & \mu \\ & & & & \nu \end{pmatrix}. \quad (55)$$

Obviously, the eigenspace corresponding to the unit eigenvalue of  $T_k^G$  is exactly  $\text{Comm}_k(G)$  whose eigenvectors, by definition, also commute with the restricted representation on the ensemble  $\mathcal{E}$ . Therefore,

$$\text{Comm}_k(G) \subset \text{Comm}_k(\mathcal{E}). \quad (56)$$

as instantiate in Eq.(55). It is now clear that only when  $0 \leq |\lambda|, |\mu|, |\nu| < 1$ , applying  $T_k^{\mathcal{E}}$  many times, i.e., sampling from the ensemble into a circuit depth  $p$ , would approximate  $T_k^G$  in the sense of Definition II.2. Within this framework, evaluating the upper bound of the *second largest abstract value* of these  $\lambda, \mu, \nu$  helps to determine the convergence speed of achieving unitary  $k$ -design through  $\mathcal{E}$ . The case when  $T_k^{\mathcal{E}}$  is non-Hermitian is tackled by calculating the frame potential introduced in the subsequent subsection.

As a basic application of this perspective, suppose  $\mathcal{E}$  is taken as a compact subgroup of  $G$ , e.g, an one-parameter subgroup, equipped with the Haar measure inherited from that of  $G$ . Then  $T_k^{\mathcal{E}}$  is also a projector and the eigenvalues  $\lambda, \mu, \nu$  exemplified above is either 0 or 1. Therefore,  $T_k^{\mathcal{E}} = T_k^G$  if and only if  $\text{Comm}_k(\mathcal{E}) = \text{Comm}_k(G)$  which further indicates the following simple but significant result:

**Theorem II.4.** *If the unitary ensemble  $\mathcal{E}$  is taken as a compact Lie subgroup of  $G$  with restricted Haar measure, then either  $\mathcal{E}$  forms exact unitary  $k$ -design or it can never form any design even in the approximate sense.*

As an immediate and insightful example, one-parameter subgroups generally do not even form approximate  $k$ -design when the ambient group  $G$  is of large dimension. However, the CQA ensemble consisting of various one-parameter subgroups (and their generalizations) is proved to be able to fulfill the task in [12].

We now review the relationship between unitary  $k$ -design and *random walks on compact groups* [48–50], which would elaborate the strategy of computing second largest eigenvalue with more deep insights from probability and representation theory of groups. To begin with, let us define the convergence of measures over groups:

**Definition II.5.** Suppose  $\{\mu_p\}$  is a sequence of probability densities/measures over a compact group  $G$ , then it *converges under the weak star topology*, or simply *converges weakly*, to the Haar measure  $\mu$ , denoted by  $\mu_p \xrightarrow{w} \mu$ , if for any continuous (and automatically bounded) function  $f$  defined on  $G$ ,

$$\lim_{p \rightarrow \infty} \int_G f(g) d\mu_p(g) = \int_G f(g) d\mu(g) \text{ or equivalently } \lim_{p \rightarrow \infty} \mathbb{E}_{\mu_p}(f) = \mathbb{E}_{\mu}(f). \quad (57)$$

Note that the limit is considered independently for each single function  $f$ . Requiring the *uniform convergence* for all  $f$  is somewhat too strong on continuous compact groups [48, 50].

In order to check whether  $\mu_p \rightarrow \mu$  in this sense, we have the following famous Lévy continuity theorem generalized from classical Euclidean space to compact group which translates the convergence of expectations by *Fourier transformation* to the convergence of certain operators acting on irreducible representations of  $G$ .

**Theorem II.6** (Lévy continuity theorem). [49] *Given any irrep  $\pi$  of the compact group  $G$  and any density function  $\nu$ , the operator*

$$\hat{\nu}(\pi) := \int_G \pi(g) d\nu(g) \quad (58)$$

*acting on the representation space of  $\pi$  is called the Fourier transform or characteristic function of  $\nu$ . The convergence of  $\mu_n \rightarrow \mu$  defined above is equivalent to the convergence of matrix entries  $\hat{\mu}_n(\pi)_{ij} \rightarrow \hat{\mu}(\pi)_{ij}$  for all inequivalent  $G$  irreps.*

Let us check the Fourier transformation of the Haar measure  $\mu$ :

$$\hat{\mu}(\pi) = \int_G \pi(g) d\mu(g) = \begin{cases} 1 & \pi \text{ is the trivial representation} \\ 0 & \text{otherwise} \end{cases}. \quad (59)$$

This is due to the so-called *Schur orthogonality* which we formally used, together with Littlewood-Richardson rule, as the very first step to prove that CQA forms exact  $k$ -design in [12]. Since  $\hat{\mu}_n(\pi) \equiv 1$  on the trivial representation, the operator norm

$$\left\| \bigoplus_{\lambda} \hat{\mu}_n(\pi) - \bigoplus_{\lambda} \hat{\mu}(\pi) \right\| \quad (60)$$

taking over all inequivalent  $G$  irreps or the second largest abstract value of eigenvalues of  $\bigoplus_{\lambda} \hat{\mu}_n(\pi)$  (if they are diagonalizable) determine whether and how fast  $\mu_n$  converges to  $\mu$ .

*Remark.* A random walk on the group  $G$  is simply a sequence  $\{S_n\}$  of random variables  $S_n = X_1 \cdots X_n$  for which  $X_i$  are independent random variable with values in the group  $G$  distributed according to the same density  $\nu$ . This induces a sequence of densities  $\{\nu^{*n}\}$  with which one can examine its convergence via the previous theorem.

On the other hand, on a quantum circuit, we define the  $k$ -fold channel

$$T_k^\mathcal{E} = \int_{\mathcal{E}} V^{\otimes k} \otimes \bar{V}^{\otimes k} dV \quad (61)$$

of an ensemble  $\mathcal{E}$  and compare it with  $T_k^G$ . The ensemble would be applied several times which imitates a random walk on the quantum circuit and we note that the tensor product  $V^{\otimes k} \otimes \bar{V}^{\otimes k}$  from the integral can be in principle decomposed further with respect to the irreps of  $G$ , therefore we may interpret  $T_k^\mathcal{E}$  as a *truncated* Fourier transform of the measure  $\nu$  associated to  $\mathcal{E}$ , which tells the reason to compute  $\|(T_k^\mathcal{E})^p - T_k^G\|$  as in the example of Eq.(55) from a viewpoint of random walk.

It should be careful that unitary  $k$ -design is a weaker concept than the convergence of measures. For instance,  $\text{SU}(N)$  is an exact  $k$ -design to  $\text{U}(N)$  for arbitrary  $k$ , but  $\text{SU}(N) \neq \text{U}(N)$  and hence there is no reason to say that the Haar measure of  $\text{SU}(N)$  converges to that of  $\text{U}(N)$ . Even comparing the integral with respect to these measures, there are still counterexamples: let  $\det$  denote the determinant function. Then

$$\int_{\text{SU}(N)} \det V dV = 1 \neq \int_{\text{U}(N)} \det U dU = 0. \quad (62)$$

The formal reason is that there is no guarantee that  $V^{\otimes k} \otimes \bar{V}^{\otimes k}$  encompasses all inequivalent irreps even when  $k \rightarrow \infty$ , e.g., the 1-dimensional representation  $\det$  given by taking determinant [1, 3]. However, unitary  $k$ -design is more practical and reasonably fits into the case of quantum computation where we twirl states or density matrices by unitaries as  $U^{\otimes k} \rho U^{\dagger \otimes k}$ . Henceforth, instead of worrying about the convergence of arbitrary function as in Eq.(57), we only focus on functions involves entries and their conjugates of  $U$  equally which can be expanded by homogeneous polynomials of these variables captured by unitary  $k$ -design [40]. Nevertheless, representation theory are still of great importance and used throughout this work.

### C. Frame Potential, Form factors, and $k$ -Invariance

We now show that the perspective of defining  $k$ -fold channel and computing their second largest eigenvalues are tightly related with the following two quantities: the *spectral form factor*  $R_{2k}^\mathcal{E}$  and the *frame potential*  $F_\mathcal{E}^{(k)}$  developed and used in recent physics literature [40–45]. The former is defined as

$$R_{2k}^\mathcal{E} := \int_{\mathcal{E}} dU |\text{tr}(U)|^{2k}. \quad (63)$$

Using the facts that traces interchange with integrals and the identity  $\text{tr}(U \otimes V) = \text{tr } U \text{tr } V$ , we get

$$R_{2k}^\mathcal{E} = \text{tr} \left( \int_{\mathcal{E}} U^{\otimes k} \otimes \bar{U}^{\otimes k} dU \right) = \text{tr } T_k^\mathcal{E}. \quad (64)$$

Especially when  $\mathcal{E} = G$ ,  $R_{2k}^G = \text{tr } T_k^G$  measures precisely the *dimension* of the commutant  $\text{Comm}_k(G)$  explained previously. For  $k$ -design without symmetry, we set  $G = \text{U}(d^n) \equiv \text{U}(N)$ . It is well-known by Schur-Weyl duality that  $R_{2k}^G = k!$  when  $k < d^n = N$  [3, 4]. In the most general setting for arbitrary large  $k$ ,  $R_{2k}^G$  is proved to be equal to the number of permutations having no *increasing subsequence* of length greater than  $d^n$  [51], which relates to the so-called *increasing subsequence problem* from combinatorics [2].

The frame potential characterizes the 2-norm distance between a given ensemble and the Haar random unitary:

$$F_\mathcal{E}^{(k)} = \int_{\mathcal{E}} dU dV \|\text{tr}(UV^\dagger)\|^{2k} \quad (65)$$

Comparing with spectral form factor, frame potential is defined for a more general choices of the ensembles:

**Proposition II.7.** Given an arbitrary ensemble  $\mathcal{E}$ ,

$$F_\mathcal{E}^{(k)} = \text{tr}(T_k^{\mathcal{E}^\dagger} T_k^\mathcal{E}). \quad (66)$$

As an immediate result, if  $T_k^\mathcal{E}$  is Hermitian,  $F_\mathcal{E}^{(k)} = \text{tr}((T_k^\mathcal{E})^2)$ . When  $\mathcal{E}$  is compact subgroup,

$$F_\mathcal{E}^{(k)} = R_{2k}^\mathcal{E}. \quad (67)$$

In either cases, the frame potential is lower-bounded by  $F_G^{(k)} = R_{2k}^G$ .

*Proof.* Just as we derive  $R_{2k}^\mathcal{E} = \text{tr } T_k^\mathcal{E}$  from above,

$$\begin{aligned} F_\mathcal{E}^{(k)} &= \int_{U,V \in \mathcal{E}} |\text{tr}(U^\dagger V)|^{2k} dV dU = \int_{U,V \in \mathcal{E}} \text{tr}((U^\dagger V)^{\otimes k} \otimes (\overline{U^\dagger V})^{\otimes k}) dV dU \\ &= \text{tr} \int_{U,V \in \mathcal{E}} (U^\dagger V)^{\otimes k} \otimes (\overline{U^\dagger V})^{\otimes k} dV dU = \text{tr} \int_{U \in \mathcal{E}} \int_{V \in \mathcal{E}} (U^{\dagger \otimes k} \otimes \bar{U}^{\dagger \otimes k}) (V^{\otimes k} \otimes \bar{V}^{\otimes k}) dV dU \\ &= \text{tr} (T_k^{\mathcal{E}^\dagger} T_k^\mathcal{E}). \end{aligned} \quad (68)$$

When  $\mathcal{E}$  is taken as a compact subgroup of  $G$  with the restricted Haar measure,  $T_k^\mathcal{E} = T_k^{\mathcal{E}^\dagger}$  becomes a projector by Lemma II.3. Then

$$F_\mathcal{E}^{(k)} = \text{tr} ((T_k^\mathcal{E})^2) = \text{tr } T_k^\mathcal{E} = R_{2k}^\mathcal{E}. \quad (69)$$

Finally, no matter  $T_k^\mathcal{E}$  is Hermitian or not,  $T_k^{\mathcal{E}^\dagger} T_k^\mathcal{E}$  is always diagonalizable with nonnegative eigenvalues. Let  $W_{k,\mathcal{E}}^{\lambda=1}$  denote its unit eigenspace, as the example of Eq.(55), for any  $M \in \text{Comm}_k(G)$ ,

$$\begin{aligned} U^{\otimes k} M &= U^{\otimes k} M, U^{\dagger \otimes k} M = U^{\dagger \otimes k} M \\ \implies T_k^{\mathcal{E}^\dagger} T_k^\mathcal{E}(M) &= M \\ \implies F_G^{(k)} = R_{2k}^G &= \text{tr}(T_k^G) = \dim \text{Comm}_k(G) \leq \dim W_{k,\mathcal{E}}^{\lambda=1} \leq F_\mathcal{E}^{(k)}. \end{aligned} \quad (70)$$

This finishes the proof.  $\square$

Note that the last statement  $F_G^{(k)} \leq F_\mathcal{E}^{(k)}$  is verified directly using the bi-invariance of Haar measure in literature [41–45] when comparing the real Haar randomness with that assigned by the ensemble  $\mathcal{E}$ . Our method incorporates insights from commutant theory which shows its usefulness in study  $\text{SU}(d)$  symmetric  $k$ -design [12].

We now introduce the  $k$ -invariance [44] which characterizes how invariant it is under the Haar random unitary. For a given ensemble,  $k$ -invariance  $I_\mathcal{E}^{(k)}$  is defined by

$$I_\mathcal{E}^{(k)} = F_\mathcal{E}^{(k)} - F_{\tilde{\mathcal{E}}}^{(k)} \quad (71)$$

where  $\tilde{\mathcal{E}}$  is obtained from averaging  $\mathcal{E}$  over the Haar measure

$$\tilde{\mathcal{E}} = \left\{ \int_G dW (W U W^\dagger) : U \in \mathcal{E} \right\} \quad (72)$$

By simialr methods used above,

$$\begin{aligned} F_{\tilde{\mathcal{E}}}^{(k)} &= \text{tr} \left( \left( \int_{\tilde{\mathcal{E}}} d\tilde{U} \int_{\tilde{\mathcal{E}}} d\tilde{V} (\tilde{U}^{\dagger \otimes k} \otimes \tilde{U}^{\dagger \otimes k}) (V^{\otimes k} \otimes \bar{V}^{\otimes k}) \right) \right) \\ &= \text{tr} \left( \int_{\mathcal{E}} dU \int_G dW \int_{\mathcal{E}} dV \int_G dX ((W U^\dagger W^\dagger)^{\otimes k} \otimes (\overline{W U^\dagger W^\dagger})^{\otimes k}) ((X V X^\dagger)^{\otimes k} \otimes (\overline{X V X^\dagger})^{\otimes k}) \right) \\ &= \text{tr} \left( (T_k^G T_k^{\mathcal{E}^\dagger} T_k^G) (T_k^G T_k^\mathcal{E} T_k^G) \right) = \text{tr} (T_k^G T_k^{\mathcal{E}^\dagger} T_k^\mathcal{E} T_k^G) = \text{tr}(T_k^G). \end{aligned} \quad (73)$$

Obviously, the  $k$ -invariance  $I_\mathcal{E}^{(k)} \geq 0$ . If  $\mathcal{E}$  is an exact  $k$ -design,  $I_\mathcal{E}^{(k)} = 0$ . We say that any ensemble for which  $I_\mathcal{E}^{(k)} = 0$  is  $k$ -invariant.

*Remark.* With the previous introduction on commutant, eigenvalues or spectral of  $k$ -fold channel and frame potential, we now reveal their relationship. Given an arbitrary ensemble  $\mathcal{E}$  with measure  $\nu$ , we sample unitaries from the ensemble  $\mathcal{E}$  into a circuit depth  $p$ , or we take a  $p$  steps random walk via the ensemble, which by definition yields the twirling channel  $(T_k^\mathcal{E})^p$ . We also assume that  $T_k^\mathcal{E}$  is Hermitian with nonnegative eigenvalues (*positive semidefinite*).

With this assumption, in the language of commutant theory, we evaluate the *second largest eigenvalue*  $\lambda$  of  $T_k^\mathcal{E}$ . It has been shown in [27, 36, 37] that to obtain an  $\epsilon$ -approximate  $k$ -design  $\|(T_k^\mathcal{E})^p - T_k^G\|_\diamond \leq \epsilon$ ,

$$p = \frac{1}{\log 1/\lambda} \log \frac{N^{2k}}{\epsilon}. \quad (74)$$

Since for large  $x$ ,  $x \leq (x+1) \log(x+1)$ ,

$$\frac{1}{\log \frac{1}{\lambda}} = \frac{1}{\log \frac{1-\lambda}{\lambda} + 1} \leq \frac{\frac{1-\lambda}{\lambda} + 1}{\frac{1-\lambda}{\lambda}} = \frac{1}{1-\lambda} \implies p \leq \frac{1}{1-\lambda} \log \frac{N^{2k}}{\epsilon}. \quad (75)$$

Therefore, a polynomial *spectral gap* between first and second largest eigenvalues of  $T_k^{\mathcal{E}}$  guarantees an efficient random circuit scheme (also see [46, 47]).

On the other hand, suppose we turn to estimate the frame potential  $F_{\mathcal{E}}^{(k)}(p)$  for each step  $p$ . Then the inequality

$$\|(T_k^{\mathcal{E}})^p - T_k^G\|_{\diamond}^2 \leq N^{2k} (F_{\mathcal{E}}^{(k)}(p) - F_G^{(k)}) \quad (76)$$

can be applied to bound the difference under diamond norm [43–45]. By Proposition II.7, knowing both the second largest eigenvalue  $\lambda$  and  $F_G^{(k)} = \dim \text{Comm}_k(G)$  is sufficient to bound

$$F_{\mathcal{E}}^{(k)}(p) = \text{tr}((T_k^{\mathcal{E}})^{2p}) = \sum_i \lambda_i^{2p}, \quad (77)$$

where  $\lambda_i$  denote eigenvalues of  $T_k^{\mathcal{E}}$ . Conversely, knowing  $F_{\mathcal{E}}^{(k)}(p)$  for all  $p \in \mathbb{N}$  determines these eigenvalues  $\lambda_i$  uniquely by the so-called *moment problem* studied in number theory and algebraic geometry [52]. Even it is generally impossible to solve  $\lambda_i$  explicitly in Eq.(77), this consideration finally relates the concepts of frame potential, commutant, operator traces and eigenvalues together in approximating  $k$ -design.

#### D. Commutant of the Group $U(\bigoplus_{\lambda} S^{\lambda})$ of $SU(d)$ Symmetric Unitaries

In later sections proving our main results on unitary  $k$ -design under  $SU(d)$  symmetry, we always adopt the approach using  $S_n$  representation theory and analyzing commutant and eigenvalues, instead of computing the frame potential. At the end of this section, we explain the potential difficulty of working with frame potential at the presence of  $SU(d)$  symmetry and describe the commutant of  $U(\bigoplus_{\lambda} S^{\lambda})$  with a explicit spanning set, which stands at the center of Section III for our computation of  $T_{k=2}^{\text{CQA}}(M)$  to analyze several related applications.

To motivate the following proof, we first consider the commutant algebra  $\text{Comm}_k(U(d^n))$  for a generic  $n$ -qudit system  $H = V^{\otimes n}$  with no symmetry. It is well-known by Schur-Weyl duality and double commutant theorem [3, 4] that

$$\text{Comm}_k(U(d^n)) = \text{span}\{\sigma, \sigma \in S_k\}, \quad (78)$$

where  $\sigma$  should be understood as the permutation on the  $k$ -fold tensor product  $H^{\otimes k}$  (cf. permutations on  $n$  qudits). Let us move furthermore to express  $\sigma$  explicitly. To this end, we note that any  $M \in \text{Comm}_k(U(N))$  is just an element from  $\text{End}(H^{\otimes k})$  which possess a standard basis given by tensor products of matrix units, i.e., matrices  $E_{ij}$  with unit entry in the position  $(i, j)$  and zero entries elsewhere. Under computational basis  $\{|i\rangle\}_{i=1}^N$ ,

$$E_{ij} = |i\rangle \langle j|. \quad (79)$$

Then it is straightforward to check by definition that

$$\sum_{i,j} E_{ii} \otimes E_{jj}, \quad \sum_{i,j} E_{ij} \otimes E_{ji}, \quad \sum_{i,j,k,r,s} E_{is} \otimes E_{jk} \otimes E_{kr} \otimes E_{rj} \otimes E_{si} \quad (80)$$

correspond respectively to the identity matrix, the transposition  $(1, 2)$  on the first two indices, and the permutation  $(15)(234)$  which swaps the first and fifth indices while translates the second, third and forth indices cyclically. Note that we define these operators on  $H^{\otimes k}$  for arbitrary  $k$ , but we omit the cumbersome tensor products with identity matrix  $I$  in the above expression. A general permutation  $\sigma$  of cycle type  $\mu = (\mu_1, \dots, \mu_r) \vdash k$  (Definition I.3) can be written out following this procedure: when there is a basis vector label  $i$  appearing as a covariant/contravariant index of some matrix unit from the tensor product, it should be assigned again as a contravariant/covariant index. Except using computational basis, permutations can also be expanded by (generalized) Pauli matrices with nice properties being used in Section III A. Any of these expansions are significant to study common unitary  $k$ -design [27, 38, 41].

We now discuss the more involved case for  $\text{Comm}_k(U(\bigoplus_{\lambda} S^{\lambda}))$ . Recall that as we study  $SU(d)$  symmetric quantum circuit, the entire Hilbert space  $H = V^{\otimes n}$  of qudits decomposes by Schur-Weyl duality into irreps  $S^{\lambda}$  of  $S_n$  with multiplicities  $m_{S_n, \lambda}$  (Section IB):

$$H \cong \bigoplus_{\lambda} I_{m_{S_n, \lambda}} \otimes S^{\lambda}. \quad (81)$$

We also introduced in Section I A spanning these irreps by Young-Yamanouchi basis. Thus we change from computational basis  $\{|i\rangle\}$  to Young basis  $\{|\alpha_T, m\rangle\}$ , with  $\alpha_T$  labeling a basis vector and  $m$  recording the irrep multiplicity by Schur transform [4, 5, 25] and redefine the matrix unit as

$$E_{(\alpha_T, m), (\alpha_{T'}, m')} = |\alpha_T, m\rangle \langle \alpha_{T'}, m'|. \quad (82)$$

It turns out that the commutant  $\text{Comm}_k(U(\bigoplus_\lambda S^\lambda))$  is spanned by "permutations" generalized from Eq.(80) using  $E_{(\alpha_T, m), (\alpha_{T'}, m')}$ . As the simplest but enlightening example, we have

$$\sum_{T_1, T_2} E_{(\alpha_{T_1}, m_1), (\alpha_{T_1}, m'_1)} \otimes E_{(\alpha_{T_2}, m_2), (\alpha_{T_2}, m'_2)} \quad (83)$$

generalized from  $\sum_{i,j} E_{ii} \otimes E_{jj}$ . However, Eq.(83) no longer represents the identity matrix because the summation is taken within two  $S_n$  irreps labeled by the Young diagrams of  $T_1, T_2$ , but not over the entire space  $H^{\otimes k}$ . Besides, the multiplicity indices can vary arbitrarily: there is *no need* to require  $m_1 = m'_1$  or  $m_2 = m'_2$ . We only couple each basis vector label in pair as covariant and contravariant indices. Moreover, when  $k = 2$  or  $5$ ,

$$\sum_{T_1, T_2} E_{(\alpha_{T_1}, m_1), (\alpha_{T_2}, m_2)} \otimes E_{(\alpha_{T_2}, m'_2), (\alpha_{T_1}, m'_1)}, \quad (84)$$

$$\begin{aligned} \sum_{T_1, T_2, T_3, T_4, T_5} E_{(\alpha_{T_1}, m_1), (\alpha_{T_5}, m_5)} \otimes E_{(\alpha_{T_2}, m_2), (\alpha_{T_3}, m_3)} \\ \otimes E_{(\alpha_{T_3}, m'_3), (\alpha_{T_4}, m_4)} \otimes E_{(\alpha_{T_4}, m'_4), (\alpha_{T_2}, m'_2)} \otimes E_{(\alpha_{T_5}, m'_5), (\alpha_{T_1}, m'_1)}, \end{aligned} \quad (85)$$

show how to generalize the left two examples from Eq.(80). With all these preparation, we prove the following theorem:

**Theorem II.8.** *The commutant  $\text{Comm}_k(U(\bigoplus_\lambda S^\lambda))$  is spanned by a generalized form of permutations exemplified in Eq.(83) and Eq.(84).*

*Proof.* By definition, matrix representations  $U$  of group elements  $g \in U(\bigoplus_\lambda S^\lambda)$  are just collections of unitary matrices acting on inequivalent  $S_n$  irrep blocks with identical copies on the multiplicity spaces (Eq.(30)). Thus the conjugation action of  $U(\bigoplus_\lambda S^\lambda)$  on any simple tensor product of matrix units is given by,

$$(U_1 E_{(\alpha_{T_1}, m_1), (\alpha_{T_2}, m_2)} U_2^\dagger) \otimes (U_3 E_{(\alpha_{T_3}, m_3), (\alpha_{T_4}, m_4)} U_4^\dagger) \otimes \cdots \otimes (U_{2k-1} E_{(\alpha_{T_{2k-1}}, m_{2k-1}), (\alpha_{T_{2k}}, m_{2k})} U_{2k}^\dagger) \quad (86)$$

where  $U_i$  are unitaries acting on decomposed  $S_n$  irreps spanned by  $\{|\alpha_{T_i}\rangle\}$ . A generic element  $M \in \text{End}(H^{\otimes k})$  is a linear combination of simple tensor products of matrix units:

$$M = \sum_{T_i, M_i} c_{T_i, M_i} E_{(\alpha_{T_1}, m_1), (\alpha_{T_2}, m_2)} \otimes E_{(\alpha_{T_3}, m_3), (\alpha_{T_4}, m_4)} \otimes \cdots \otimes E_{(\alpha_{T_{2k-1}}, m_{2k-1}), (\alpha_{T_{2k}}, m_{2k})}, \quad (87)$$

as they form a standard basis for  $\text{End}(H^{\otimes k})$ . Belonging to  $\text{Comm}_k(U(\bigoplus_\lambda S^\lambda))$  means being invariant under the conjugate action for arbitrary  $U = \rho(g)$ .

We first select  $U_i$  as arbitrary diagonal phase matrices. Then the conjugate action accounts for scalar products with phases factors on each simple tensor. Since these simple tensors are linearly independent, being invariant under phase change implies such invariance for individual simple tensor from Eq.(87), which leads to the requirement on coupling basis vector labels in pairs of covariant and contravariant indices. For instance, when  $k = 2$ , phase-change invariant simple tensors are of the following forms:

$$(U_1 E_{(\alpha_{T_1}, m_1), (\alpha_{T_1}, m'_1)} U_1^\dagger) \otimes (U_2 E_{(\alpha_{T_2}, m_2), (\alpha_{T_2}, m'_2)} U_2^\dagger) \quad (88)$$

or

$$(U_1 E_{(\alpha_{T_1}, m_1), (\alpha_{T_2}, m_2)} U_2^\dagger) \otimes (U_2 E_{(\alpha_{T_2}, m'_2), (\alpha_{T_1}, m'_1)} U_1^\dagger). \quad (89)$$

With this example, let  $U_1$  be matrices exchanging arbitrary rows and columns like

$$U_1 = \begin{pmatrix} 1 & 0 & 0 \\ 0 & 0 & 1 \\ 0 & 1 & 0 \end{pmatrix} \quad (90)$$



while we set  $U_2$  being the identity matrix. Conjugated by this kind of  $U(\bigoplus_\lambda S^\lambda)$  group elements, the basis vector label  $\alpha_{T_1}$  varies arbitrarily inside the  $S_n$  irrep acted on by  $U_1$ . Therefore, being invariant indicates that we should take summations over  $T_1, T_2$  which yield:

$$\sum_{T_1, T_2} E_{(\alpha_{T_1}, m_1), (\alpha_{T_1}, m'_1)} \otimes E_{(\alpha_{T_2}, m_2), (\alpha_{T_2}, m'_2)} \quad (91)$$

and

$$\sum_{T_1, T_2} E_{(\alpha_{T_1}, m_1), (\alpha_{T_2}, m_2)} \otimes E_{(\alpha_{T_2}, m'_2), (\alpha_{T_1}, m'_1)}. \quad (92)$$

However, these consideration have no influence on the choices of multiplicity labels  $m_i$  and that is why they are assigned arbitrarily.

We still need to prove that operators  $M$  spanned with the above requirements commutes all other unitaries from  $U(\bigoplus_\lambda S^\lambda)$ . This is done by arguing through the Lie algebra  $\mathfrak{g} = \mathfrak{L}(U(\bigoplus_\lambda S^\lambda))$  consisting of

$$E \otimes I \otimes \cdots \otimes I + I \otimes E \otimes \cdots \otimes I + \cdots I \otimes \cdots \otimes I \otimes E \in \text{End}(H^{\otimes k}) \quad (93)$$

with  $E$  being an anti-Hermitian matrix respecting the decomposition of  $H^{\otimes k}$  under  $SU(d)$  symmetry. We expand  $E$  by matrix units and examine the commutativity: Using the example:

$$M = \sum_{T_1, T_2} E_{(\alpha_{T_1}, m_1), (\alpha_{T_2}, m_2)} \otimes E_{(\alpha_{T_2}, m'_2), (\alpha_{T_1}, m'_1)}, \quad (94)$$

we have

$$(E_{(\alpha_T, m), (\alpha_{T'}, m')} \otimes I)M = \sum_{T_2} E_{(\alpha_T, m), (\alpha_{T_2}, m_2)} \otimes E_{(\alpha_{T_2}, m'_2), (\alpha_{T'}, m')} = M(I \otimes E_{(\alpha_T, m), (\alpha_{T'}, m')}) \quad (95)$$

by contracting the same tensor indices. Analogously,  $(I \otimes E_{(\alpha_T, m), (\alpha_{T'}, m')})M = M(E_{(\alpha_T, m), (\alpha_{T'}, m')} \otimes I)$  and hence  $M$  commutes with the Lie algebra elements. Generally case for arbitrary  $k$  is deduced similarly and we complete the proof.  $\square$

*Remark.* With this theorem, let us try to compute the frame potential  $F_{\text{Haar}}^{(k)}$  for  $G = U(\bigoplus_\lambda S^\lambda)$ . The simplest case is  $k = 1$ , when  $\text{Comm}_k(U(\bigoplus_\lambda S^\lambda))$  is spanned by

$$\sum_T E_{(\alpha_T, m), (\alpha_T, m')} \quad (96)$$

for each  $S_n$  irrep appearing in the decomposition and with arbitrary copies. When the system consists of  $n$ -qubits, Schur-Weyl duality says that there are  $p(n, 2) = \lfloor \frac{n}{2} \rfloor + 1$  inequivalent  $S_n$  irreps corresponding to two-row Young diagrams in the decomposition. Moreover, the multiplicity of the irrep  $S^\lambda$  with  $\lambda = (n - r, r)$  is  $n - 2r + 1$ . Therefore, for qubits,

$$F_{\text{Haar}}^{(1)} = \dim \text{Comm}_{k=1}(U(\bigoplus_\lambda S^\lambda)) = \sum_{0 \leq r \leq \lfloor n/2 \rfloor} (n - 2r + 1)^2. \quad (97)$$

When  $k = 2$ ,

$$\begin{aligned} F_{\text{Haar}}^{(2)} = \dim \text{Comm}_{k=2}(U(\bigoplus_\lambda S^\lambda)) &= (n+1)^4 + 2 \sum_{1 \leq r \leq \lfloor n/2 \rfloor} (n - 2r + 1)^4 \\ &\quad + 2 \sum_{0 \leq r \neq s \leq \lfloor n/2 \rfloor} (n - 2r + 1)^2 (n - 2s + 1)^2, \end{aligned} \quad (98)$$

where the first two terms in the RHS appears when four indices of basis vectors  $\alpha_T$  from Eq.(83) are all selected from an equivalent  $S_n$  irrep. As the trivial irrep ( $r = 1$ ) of  $S_n$  is 1-dimensional with no freedom for exchanging indices, we separate it from the second term. The third term counts the case when two pairs of indices are chosen from two inequivalent  $S_n$  irreps. Then general case follows as above.

For qudits, the number of inequivalent  $S_n$  irreps is  $p(n, d)$  which denotes the number of Young diagrams with  $n$  boxes and at most  $d$  rows (Definition I.4). Unfortunately, there is no closed formula for  $p(n, d)$ , except the asymptotic formula due to Ramanujan, Hardy and Uspensky [13, 14], and later developed bounds in [17, 18] Consequently, it may not be easy to calculate the frame potential  $F_{\text{Haar}}^{(k)}$  for the group of  $SU(d)$  symmetric unitaries, no to mention comparing it with  $F_{\mathcal{E}}^{(k)}$  in (76). To bypass this obstacle to some extent, we would work exclusively with commutant algebra  $\text{Comm}_k(U(\bigoplus_\lambda S^\lambda))$  in the following context to present our main results.

### III. APPLICATIONS OF $\text{SU}(d)$ SYMMETRIC 2-DESIGN

We now present the details for analyzing quantum scrambling, quantum error correction and quantum machine learning with the presence of  $\text{SU}(d)$  symmetry using our previously developed results on  $\text{SU}(d)$ -symmetric  $k$ -design.

#### A. General Setting and Explicit Expansion for $T_{k=2}^{\text{CQA}}$

We first set up the scenario for general quantum information recovery process provide necessary mathematical techniques for computation under continuous symmetry. As described in the main text, the entire  $n$ -qudit system is divided into two parts  $A, \bar{A}$  where  $A$  contains  $k$  qudits carrying the information entangled with a reference system  $R$  depicted as the density matrix  $\rho_{R \cup A}$ . The left part  $\bar{A}$  bears a prescribed mixed state  $\rho_{\bar{A}}$ , which may be further purified by adding a memory MEM as  $\rho_{\bar{A} \cup \text{MEM}}$ . After being processed under certain quantum channel, we try to recover or decode the information by  $n - t$  qudits from the system, denoted by  $B$ , even by the memory MEM if it is applicable.

We adopt *abstract index notation* in order to give a clear and precise mathematical description for the process, plus tensor network diagrams illustrating the idea graphically. As a brief introduction, let us rewrite the initial state  $\rho_{R \cup A}, \rho_{\bar{A} \cup \text{MEM}}$  by

$$Q^{RA} Q_{R'A'}, \quad P^{\bar{A}M} P_{\bar{A}'M'}, \quad (99)$$

where  $Q^{RA}, P^{\bar{A}M}$  denotes the purified states in  $A$  and  $\bar{A}$  respectively. Superscript indices correspond to vectors (ket) while subscript indices correspond to dual vectors (bra). Then

$$U^{B\bar{B}}_{A\bar{A}} Q^{RA} P^{\bar{A}M} \quad (100)$$

represents the unitary action  $U^{B\bar{B}}_{A\bar{A}}$  on initial states. When a pair of the same indices appears, we contract tensors in that place which concretely means that we apply *Einstein summation convention* to sum all components of operators with the same indices in that place. One notable reason to use abstract index notation is that *tensor contractions* turn out to be matrix actions on vectors, matrix products, taking (partial) traces and so forth in different circumstances, which provides a unified framework for our later computations. As reminder, the initial states may be left mixed in some cases (see Section III D) and we simply write  $P^{\bar{A}}_{\bar{A}'}$  for the whole density matrix.

The total density matrix under unitary action is written as

$$D^{RB\bar{B}M}_{R'B'\bar{B}'M'} = (U^{B\bar{B}}_{A\bar{A}} Q^{RA} P^{\bar{A}M})(Q_{R'A'} P_{\bar{A}'M'} U_{B'\bar{B}'}^{A'\bar{A}'}). \quad (101)$$

We are going to expand the following terms using abstract indices

$$\rho_{B \cup \text{MEM}} = D^{RB\bar{B}M}_{RB'\bar{B}'M'} = D^{BM}_{B'M'} \text{ and } \text{Tr}(\rho_{B \cup \text{MEM}}^2) = D^{BM}_{B'M'} D^{B'M'}_{BM}, \quad (102)$$

which interestingly yields a form of out-of-time-ordered correlation (OTOC) for Pauli operators (Eq.(110)). It turns out that averaging these quantities or their *variants* under Haar randomness with or without the symmetry is the key step throughout this section. We proceed to show some basic computational techniques and apply them to concrete questions later.

#### Computation of $\text{Tr}(\rho_{B \cup \text{MEM}}^2)$

We first expand  $\text{Tr}(\rho_{B \cup \text{MEM}}^2)$  by abstract index notation with

$$\begin{aligned} \rho_{B \cup \text{MEM}} &= D^{RB\bar{B}M}_{RB'\bar{B}'M'} = D^{BM}_{B'M'} = (U^{B\bar{B}}_{A\bar{A}} Q^{RA} P^{\bar{A}M})(Q_{RA'} P_{\bar{A}'M'} U_{B'\bar{B}'}^{A'\bar{A}'}) \\ &= U^{B\bar{B}}_{A\bar{A}} \mu^A_{A'} U_{B'\bar{B}'}^{A'\bar{A}'} P^{\bar{A}M} P_{\bar{A}'M'}, \end{aligned} \quad (103)$$

where  $Q^{RA} Q_{RA'} = \mu^A_{A'}$  is the density matrix of the initial state in  $A$ . Similarly, the matrix product  $\rho_{B \cup \text{MEM}}^2$  gives us

$$P^{\bar{A}M} P_{\bar{A}'M'} P^{\bar{A}''M''} P_{\bar{A}'''M'''} = \rho^{\bar{A}}_{\bar{A}'''} \rho^{\bar{A}''}_{\bar{A}'} \quad (104)$$

with  $\rho$  denote the density matrix of the initial state in  $\bar{A}$ . Then

$$\begin{aligned}
\text{Tr}(\rho_{B \cup \text{MEM}}^2) &= D^{BM}_{B'M'} D^{B'M'}_{BM} \\
&= \left( U^{B\bar{B}}_{A\bar{A}} \mu^A_{A'} U_{B'\bar{B}}^{A'\bar{A}'} P^{\bar{A}M} P_{\bar{A}'M'} \right) \left( U^{B'\bar{B}'}_{A''\bar{A}''} \mu^{A''}_{A'''} U_{B\bar{B}'}^{A''' \bar{A}'''} P^{\bar{A}''M'} P_{\bar{A}'''M} \right) \\
&= (U^{B\bar{B}}_{A\bar{A}} \mu^A_{A'}) (U_{B'\bar{B}}^{A'\bar{A}'} \rho^{\bar{A}''}_{\bar{A}'''}) (U^{B'\bar{B}'}_{A''\bar{A}''} \mu^{A''}_{A'''}) (U_{B\bar{B}'}^{A''' \bar{A}'''} \rho^{\bar{A}'''}_{\bar{A}''''}) \\
&= \hat{U}^{B\bar{B}}_{A'\bar{A}} \tilde{U}_{B'\bar{B}}^{A'\bar{A}''} \hat{U}^{B'\bar{B}'}_{A''\bar{A}''} \tilde{U}_{B\bar{B}'}^{A''' \bar{A}'''} \\
&= \hat{U}^{B\bar{B}}_{A'\bar{A}} \tilde{U}_{B\bar{B}'}^{A''' \bar{A}'''} \hat{U}^{B'\bar{B}'}_{A''\bar{A}''} \tilde{U}_{B'\bar{B}}^{A'\bar{A}''}.
\end{aligned} \tag{105}$$

Let  $T^{Q_A''Q_A'}_{A'A''''}$ ,  $T^{Q_B'Q_B}_{B'B'}$  be transpositions/SWAPs exchanging  $A, A'$  and  $B, B'$  repetitively. As mentioned in Section II D, it is straightforward to check by definition that transpositions can be written as

$$\sum_{i,j} E_{ij} \otimes E_{ji}, \tag{106}$$

where  $E_{ij}$  is a matrix unit acting on the concerned (sub-)space which is  $A$  or  $B$  at present. It is also conventional to adopt another expansion of transpositions given by *generalized Pauli matrices*. Let  $d_A$  denote the dimension of  $A$ , we define

$$X|j\rangle = |j+1\rangle, \quad Z|j\rangle = \omega^j|j\rangle \tag{107}$$

with  $X|d_A\rangle = |1\rangle$  and  $\omega = e^{2i\pi/d_A}$ . Those are ingredients to build  $d_A^2$  generalized Pauli matrices  $P = X^i Y^j$ ,  $i, j = 1, \dots, d_A$  acting on  $d_A$ -dimensional spaces. Then by definition,

$$\frac{1}{d_A} \sum_P P \otimes P^\dagger, \tag{108}$$

has the same effect as Eq.(106). One can restrict to the case of qubits ( $d = 2$ ) and substitute common Pauli matrices and their tensor products to gain more intuition. We expand transpositions on  $B, B'$  by similar methods. To distinguish the notation from those for  $A, A'$ , we denote them by  $V$  and  $W$  respectively. Then

$$\begin{aligned}
&\hat{U}^{B\bar{B}}_{A'\bar{A}} \tilde{U}_{B\bar{B}'}^{A''' \bar{A}'''} \hat{U}^{B'\bar{B}'}_{A''\bar{A}''} \tilde{U}_{B'\bar{B}}^{A'\bar{A}''} \\
&= T^{Q_A''Q_A'}_{A'A''''} T^{Q_B'Q_B}_{B'B'} \hat{U}^{B\bar{B}}_{Q_A'\bar{A}} \tilde{U}_{Q_B\bar{B}'}^{A''' \bar{A}'''} \hat{U}^{B'\bar{B}'}_{Q_A''\bar{A}''} \tilde{U}_{Q_B'\bar{B}}^{A'\bar{A}''} \\
&= \frac{1}{d_A d_B} \sum_{W,V} W^{Q_A''}_{A'} W_{A''''}^{Q_A'} V^{Q_B}_{B'} V_{B'}^{Q_B'} \hat{U}^{B\bar{B}}_{Q_A'\bar{A}} \tilde{U}_{Q_B\bar{B}'}^{A''' \bar{A}'''} \hat{U}^{B'\bar{B}'}_{Q_A''\bar{A}''} \tilde{U}_{Q_B'\bar{B}}^{A'\bar{A}''} \\
&= \frac{1}{d_A d_B} \sum_{W,V} \left( \hat{U}^{B\bar{B}}_{Q_A'\bar{A}} W_{A''''}^{Q_A'} \tilde{U}_{Q_B\bar{B}'}^{A''' \bar{A}'''} \right) V_{B'}^{Q_B} \left( \hat{U}^{B'\bar{B}'}_{Q_A''\bar{A}''} W_{Q_A''''}^{Q_A'} \tilde{U}_{Q_B'\bar{B}}^{A'\bar{A}''} \right) V_{Q_B'}^{Q_B'} \\
&= \frac{1}{d_A d_B} \sum_{W,V} \left( \hat{U}^{B\bar{B}}_{Q_A'\bar{A}} W_{A''''}^{Q_A'} \tilde{U}_{Q_B\bar{B}'}^{A''' \bar{A}'''} \right) \left( V_{B'}^{Q_B} \delta_{\bar{B}'}^{\bar{B}''} \right) \left( \hat{U}^{B'\bar{B}'}_{Q_A''\bar{A}''} W_{Q_A''''}^{Q_A'} \tilde{U}_{Q_B'\bar{B}}^{A'\bar{A}''} \right) \left( V_{Q_B'}^{Q_B'} \delta_{\bar{B}''}^{\bar{B}'''} \right) \\
&= \frac{1}{d_A d_B} \sum_{W,V} \left( U^{B\bar{B}}_{A\bar{A}} ((\mu^A_{Q_A'} W_{A''''}^{Q_A'}) \rho^{\bar{A}}_{\bar{A}''''}) U_{Q_B\bar{B}'}^{A''' \bar{A}'''} \right) \left( V_{B'}^{Q_B} \delta_{\bar{B}'}^{\bar{B}''} \right) \\
&\quad \left( U^{B'\bar{B}'}_{A''\bar{A}''} ((\mu^{A''}_{Q_A'''} W_{Q_A''''}^{Q_A'}) \rho^{\bar{A}''}_{\bar{A}''''}) U_{Q_B'\bar{B}}^{A'\bar{A}''} \right) \left( V_{Q_B'}^{Q_B'} \delta_{\bar{B}''}^{\bar{B}'''} \right).
\end{aligned} \tag{109}$$

We have the following indices when taking contractions:

$$(A, A', A'', A'''), \quad (B, B'), \quad (Q_A', Q_A'''), \quad (Q_B, Q_B'), \quad (\bar{A}, \bar{A}', \bar{A}'', \bar{A}'''), \quad (\bar{B}, \bar{B}', \bar{B}'', \bar{B}''').$$

It would be formidable to integrate Eq.(109) in its most general form. Instead, assume the initial states are taken to be maximally entangled, i.e.,  $\mu = \frac{1}{d_A} I$ ,  $\rho = \frac{1}{d_A} I$ . Then

$$\begin{aligned}
\text{Tr}(\rho_{B \cup \text{MEM}}^2) &= \frac{1}{d_A d_B d_A^2 d_A^2} \sum_{W,V} \left( U^{B\bar{B}}_{A\bar{A}} (W_{A''''}^A \delta_{\bar{A}''''}^{\bar{A}}) U_{B\bar{B}'}^{A''' \bar{A}'''} \right) \left( V_{B'}^B \delta_{\bar{B}'}^{\bar{B}''} \right) \\
&\quad \left( U^{B'\bar{B}'}_{A''\bar{A}''} (W_{A''''}^{A''} \delta_{\bar{A}''''}^{\bar{A}'}) U_{B'\bar{B}}^{A'\bar{A}''} \right) \left( V_{B'}^{B'} \delta_{\bar{B}''}^{\bar{B}'''} \right) \\
&= \frac{1}{d^k d^{n-t} d^{2n}} \sum_{W,V} \text{Tr}((UW^\dagger U^\dagger) V^\dagger (UWU^\dagger) V).
\end{aligned} \tag{110}$$

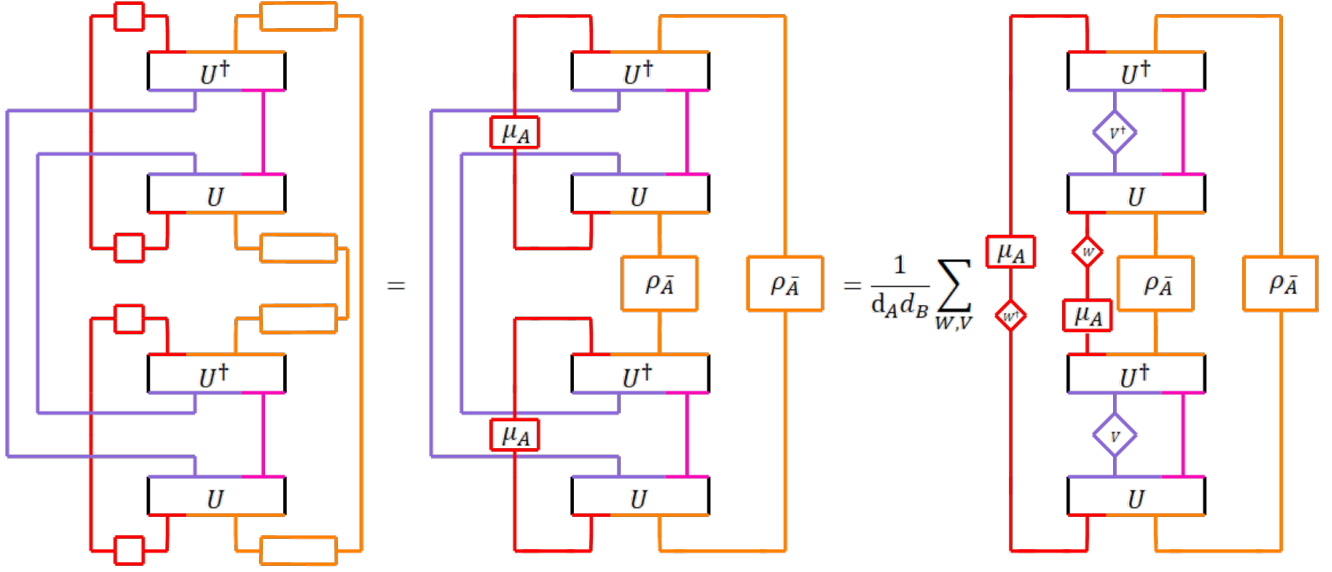

FIG. 1. Tensor network diagram illustrating the deduction from Eq.(105) to (109).

### 2-design Formula

To average Eq.(110) with its several variants appearing in subsequent subsections, we apply the 2th-fold channel  $T_{k=2}^{\text{Haar}}$  to  $W^\dagger \otimes W$  and then contract with  $V^\dagger \otimes V$ . Recall that with no concerning on the symmetry,  $\text{Comm}_{k=2}(\text{U}(d^n))$  is spanned by the following two basis elements (see Section IID):

$$I = \sum_{i,j=1}^{d_n} E_{ii} \otimes E_{jj}, \quad S = \sum_{i,j=1}^{d_n} E_{ij} \otimes E_{ji}, \quad (111)$$

where the indices  $i, j$  label any basis, e.g., the computational basis, of the  $d^n$ -dimensional entire Hilbert space. We orthogonalize this two basis vectors for the commutant. Then for any  $M \in \text{End}(H^{\otimes 2})$ ,

$$T_{k=2}^{\text{Haar}}(M) = \int_{\text{U}(d^n)} U^{\otimes 2} M U^{\dagger \otimes 2} dU = \frac{1}{d^{2n} - 1} \left( \text{Tr}(M) I + \text{Tr}(SM) S - \frac{1}{d^n} \text{Tr}(M) S - \frac{1}{d^n} \text{Tr}(SM) I \right). \quad (112)$$

Substituting  $M = W^\dagger \otimes W$  into the above identity, using the expansions from Eq.(111) and contracting with  $V^\dagger \otimes V$ , we have ( $A$  contains  $k$  qudits while  $B$  contains  $n - t$  qudits)

$$\sum_W \text{Tr}(W^\dagger \otimes W) = \sum_W \text{Tr}(W^\dagger) \text{Tr}(W) = d^{2n}, \quad \sum_W \text{Tr}(S(W^\dagger \otimes W)) = d^{2k} d^n, \quad (113)$$

$$\sum_V \text{Tr}(V^\dagger V) = d^{2n-2t} d^n, \quad \sum_{i,j,V} \text{Tr}(E_{ij} V^\dagger E_{ji} V) = \sum_V \text{Tr}(V^\dagger) \text{Tr}(V) = d^{2n}, \quad (114)$$

which assembles to

$$\int \text{Tr}(\rho_{B \cup \text{MEM}}^2) dU = \frac{1}{d^{k+n-t} d^{2n}} \left( \frac{1}{d^{2n} - 1} (d^{2n-2t} d^{3n} + d^{2k} d^{3n} - d^{3n} - d^n d^{2k+2n-2t}) \right). \quad (115)$$

This technique is immediately applied to calculate the *out-of-time-ordered correlation* (OTOC) for arbitrary operator  $W$  as long as we assume  $\text{Tr}(W) = 0$ ,  $\text{Tr}(W^\dagger W) \leq d^n$ . For nontrivial local Pauli basis element acting on one qudit ( $n - t = 1$ ),

$$\frac{1}{d^2 - 1} \frac{1}{d^n} \sum_{V \neq I} \text{Tr}((U W^\dagger U^\dagger) V^\dagger (U W U^\dagger) V) = \frac{1}{d^2 - 1} \frac{1}{d^n} \left( \frac{1}{d^{2n} - 1} \left( -\frac{1}{d^n} d^n (d^2 - 1) d^n \right) \right) = -\frac{1}{d^{2n} - 1} \rightarrow 0 \quad (116)$$

for large  $n$ .

The systematic framework to compute  $T_k^{\text{Haar}}(M)$  for larger  $k$  is called *Weingarten calculus* [41, 50, 53]. For our purpose, we only consider the case when  $k = 2$  and reformulate Eq.(112) at the presence of  $SU(d)$  symmetry. As illustrated in Section II D,  $\text{Comm}_{k=2}(U(d^n))$  is spanned by basis elements resembling those in (111), however we need to replace the computational basis indices by Young basis indices consisting of content vector  $\alpha_i$  (see Section I A) and multiplicities  $m$ :

$$\sum_{i,j} E_{(\alpha_i^\lambda, m_1), (\alpha_i^\lambda, m_2)} \otimes E_{(\alpha_j^\lambda, m_3), (\alpha_j^\lambda, m_4)}, \quad \sum_{i,j} E_{(\alpha_i^\lambda, m_1), (\alpha_i^\lambda, m_2)} \otimes E_{(\alpha_j^\lambda, m_3), (\alpha_j^\lambda, m_4)}, \quad (117)$$

$$\sum_{i,j} E_{(\alpha_i^\lambda, m_1), (\alpha_i^\lambda, m_2)} \otimes E_{(\alpha_j^\mu, m'_1), (\alpha_j^\mu, m'_2)}, \quad \sum_{i,j} E_{(\alpha_i^\lambda, m_1), (\alpha_j^\mu, m'_1)} \otimes E_{(\alpha_j^\mu, m'_2), (\alpha_i^\lambda, m_2)}, \quad (118)$$

We write  $\alpha$  with superscripts  $\lambda, \mu$  in order to explicitly show the concerned irrep sectors. The first two terms are selected from one irrep  $S^\lambda$  (but maybe from different equivalent copies). The last two terms indicates the exceptions that we also have commutant basis elements formed from inequivalent irrep sectors. Let  $d_\lambda = \dim S^\lambda$ . Orthogonalizing these basis vectors, then

$$T_{k=2}^{\text{Haar}}(M) = T_{k=2}^{\text{CQA}}(M) = \int_{U(\oplus_\lambda (S^\lambda))} U^{\otimes 2} M U^{\dagger \otimes 2} dU \quad (119)$$

is expanded in the following terms ranging from all  $S_n$  irreps with multiplicities decomposed from the entire Hilbert space by Schur-Weyl duality:

$$\begin{aligned} & \frac{1}{d_\lambda^2 - 1} \left( \text{Tr} \left( \left( \sum_{i,j} E_{(\alpha_i^\lambda, m_1), (\alpha_i^\lambda, m_2)} \otimes E_{(\alpha_j^\lambda, m_3), (\alpha_j^\lambda, m_4)} \right) M \right) \left( \sum_{i,j} E_{(\alpha_i^\lambda, m_1), (\alpha_i^\lambda, m_2)} \otimes E_{(\alpha_j^\lambda, m_3), (\alpha_j^\lambda, m_4)} \right) \right. \\ & \quad \left. + \text{Tr} \left( \left( \sum_{i,j} E_{(\alpha_i^\lambda, m_1), (\alpha_i^\lambda, m_2)} \otimes E_{(\alpha_j^\lambda, m_3), (\alpha_i^\lambda, m_4)} \right) M \right) \left( \sum_{i,j} E_{(\alpha_i^\lambda, m_1), (\alpha_i^\lambda, m_2)} \otimes E_{(\alpha_j^\lambda, m_3), (\alpha_i^\lambda, m_4)} \right) \right. \\ & \quad - \frac{1}{d_\lambda} \text{Tr} \left( \left( \sum_{i,j} E_{(\alpha_i^\lambda, m_1), (\alpha_i^\lambda, m_2)} \otimes E_{(\alpha_j^\lambda, m_3), (\alpha_j^\lambda, m_4)} \right) M \right) \left( \sum_{i,j} E_{(\alpha_i^\lambda, m_1), (\alpha_i^\lambda, m_2)} \otimes E_{(\alpha_j^\lambda, m_3), (\alpha_i^\lambda, m_4)} \right) \\ & \quad \left. - \frac{1}{d_\lambda} \text{Tr} \left( \left( \sum_{i,j} E_{(\alpha_i^\lambda, m_1), (\alpha_i^\lambda, m_2)} \otimes E_{(\alpha_j^\lambda, m_3), (\alpha_i^\lambda, m_4)} \right) M \right) \left( \sum_{i,j} E_{(\alpha_i^\lambda, m_1), (\alpha_i^\lambda, m_2)} \otimes E_{(\alpha_j^\lambda, m_3), (\alpha_j^\lambda, m_4)} \right) \right). \end{aligned} \quad (120)$$

with exceptional terms:

$$\begin{aligned} & \frac{1}{d_\lambda d_\mu} \text{Tr} \left( \left( \sum_{i,j} E_{(\alpha_i^\lambda, m_1), (\alpha_i^\lambda, m_2)} \otimes E_{(\alpha_j^\mu, m'_1), (\alpha_j^\mu, m'_2)} \right) M \right) \left( \sum_{i,j} E_{(\alpha_i^\lambda, m_1), (\alpha_i^\lambda, m_2)} \otimes E_{(\alpha_j^\mu, m'_1), (\alpha_j^\mu, m'_2)} \right), \\ & \frac{1}{d_\lambda d_\mu} \text{Tr} \left( \left( \sum_{i,j} E_{(\alpha_i^\lambda, m_1), (\alpha_j^\mu, m'_1)} \otimes E_{(\alpha_j^\mu, m'_2), (\alpha_i^\lambda, m_2)} \right) M \right) \left( \sum_{i,j} E_{(\alpha_i^\lambda, m_1), (\alpha_j^\mu, m'_1)} \otimes E_{(\alpha_j^\mu, m'_2), (\alpha_i^\lambda, m_2)} \right). \end{aligned} \quad (121)$$

We apply these formulas to study conserved quantity scrambling in the next subsection.

## B. Spreading of Local $SU(d)$ Conserved Quantities

We now apply the expansion of  $T_{k=2}^{\text{CQA}}$  to evaluate the out-of-time-ordered correlation (OTOC)  $\frac{1}{d^n} \text{Tr}(W^\dagger V^\dagger W V)$  for  $SU(d)$  conserved quantities. The local operator basis elements  $V$  are first taken from Pauli set by convention and then replaced by  $SU(d)$  symmetric local basis defined by permutations. In either case, we verify that for conserved quantities determined by exchanging interaction on qubits ( $d = 2$ ), OTOC is lower bounded by  $\Omega(\frac{1}{n^{3/2}})$  (Eq.(156)) in contrast to exponential decay with no symmetry (Eq.(116)). Moreover, our expansion of  $T_{k=2}^{\text{CQA}}$  is easily rephrased for general compact Lie group actions and we showcase an example of OTOC under  $U(1)$  symmetry for exchanging interaction and demonstrate a linear decay in Eq.(185).

*OTOC under Local Pauli Basis*

Let  $W$  denote a generic  $SU(d)$  conserved quantity, i.e.,  $W$  commutes with  $U^{\otimes n}$  for any  $U \in SU(d)$ . The 2-design projection acting on  $W^{\otimes 2}$  consists of the following term:

$$\begin{aligned} & \frac{1}{d_\lambda^2 - 1} \left( \text{Tr} \left( \left( \sum_{i,j} E_{(\alpha_i^\lambda, m_1), (\alpha_i^\lambda, m_2)} \otimes E_{(\alpha_j^\lambda, m_3), (\alpha_j^\lambda, m_4)} \right) (W^\dagger \otimes W) \right) \left( \sum_{i,j} E_{(\alpha_i^\lambda, m_1), (\alpha_i^\lambda, m_2)} \otimes E_{(\alpha_j^\lambda, m_3), (\alpha_j^\lambda, m_4)} \right) \right. \\ & \quad \left. + \text{Tr} \left( \left( \sum_{i,j} E_{(\alpha_i^\lambda, m_1), (\alpha_j^\lambda, m_2)} \otimes E_{(\alpha_j^\lambda, m_3), (\alpha_i^\lambda, m_4)} \right) (W^\dagger \otimes W) \right) \left( \sum_{i,j} E_{(\alpha_i^\lambda, m_1), (\alpha_j^\lambda, m_2)} \otimes E_{(\alpha_j^\lambda, m_3), (\alpha_i^\lambda, m_4)} \right) \right) \\ & - \frac{1}{d_\lambda} \text{Tr} \left( \left( \sum_{i,j} E_{(\alpha_i^\lambda, m_1), (\alpha_i^\lambda, m_2)} \otimes E_{(\alpha_j^\lambda, m_3), (\alpha_j^\lambda, m_4)} \right) (W^\dagger \otimes W) \right) \left( \sum_{i,j} E_{(\alpha_i^\lambda, m_1), (\alpha_j^\lambda, m_2)} \otimes E_{(\alpha_j^\lambda, m_3), (\alpha_i^\lambda, m_4)} \right) \\ & - \frac{1}{d_\lambda} \text{Tr} \left( \left( \sum_{i,j} E_{(\alpha_i^\lambda, m_1), (\alpha_j^\lambda, m_2)} \otimes E_{(\alpha_j^\lambda, m_3), (\alpha_i^\lambda, m_4)} \right) (W^\dagger \otimes W) \right) \left( \sum_{i,j} E_{(\alpha_i^\lambda, m_1), (\alpha_i^\lambda, m_2)} \otimes E_{(\alpha_j^\lambda, m_3), (\alpha_j^\lambda, m_4)} \right). \end{aligned} \quad (122)$$

Since  $W$  admits the symmetry,

$$\begin{aligned} & \text{Tr} \left( \left( \sum_{i,j} E_{(\alpha_i^\lambda, m_1), (\alpha_i^\lambda, m_2)} \otimes E_{(\alpha_j^\lambda, m_3), (\alpha_j^\lambda, m_4)} \right) (W^\dagger \otimes W) \right) = \text{Tr} \left( \sum_i E_{(\alpha_i^\lambda, m_1), (\alpha_i^\lambda, m_2)} W^\dagger \right) \text{Tr} \left( \sum_j E_{(\alpha_j^\lambda, m_3), (\alpha_j^\lambda, m_4)} W \right) \\ & = \sum_{i,j} W_{(\alpha_i^\lambda, m_2), (\alpha_i^\lambda, m_1)}^\dagger W_{(\alpha_j^\lambda, m_4), (\alpha_j^\lambda, m_3)}, \end{aligned} \quad (123)$$

$$\begin{aligned} & \text{Tr} \left( \left( \sum_{i,j} E_{(\alpha_i^\lambda, m_1), (\alpha_j^\lambda, m_2)} \otimes E_{(\alpha_j^\lambda, m_3), (\alpha_i^\lambda, m_4)} \right) (W^\dagger \otimes W) \right) = \text{Tr} \left( \sum_i E_{(\alpha_i^\lambda, m_1), (\alpha_j^\lambda, m_2)} W^\dagger \right) \text{Tr} \left( \sum_j E_{(\alpha_j^\lambda, m_3), (\alpha_i^\lambda, m_4)} W \right) \\ & = \sum_{i,j} W_{(\alpha_j^\lambda, m_2), (\alpha_i^\lambda, m_1)}^\dagger W_{(\alpha_i^\lambda, m_4), (\alpha_j^\lambda, m_3)} \end{aligned} \quad (124)$$

vanishes unless  $m_1 = m_2 = m_\lambda, m_3 = m_4 = m'_\lambda$ , which can be further simplified as

$$\sum_{i,j} W_{(\alpha_i^\lambda, m_2), (\alpha_i^\lambda, m_1)}^\dagger W_{(\alpha_j^\lambda, m_4), (\alpha_j^\lambda, m_3)} = \text{Tr}(\Pi_{\lambda, m_\lambda} W^\dagger) \text{Tr}(\Pi_{\lambda, m'_\lambda} W), \quad (125)$$

$$\sum_{i,j} W_{(\alpha_j^\lambda, m_2), (\alpha_i^\lambda, m_1)}^\dagger W_{(\alpha_i^\lambda, m_4), (\alpha_j^\lambda, m_3)} = \sum_{i,j} W_{(\alpha_j^\lambda, m_\lambda), (\alpha_i^\lambda, m_\lambda)}^\dagger W_{(\alpha_i^\lambda, m'_\lambda), (\alpha_j^\lambda, m'_\lambda)} \quad (126)$$

where  $\Pi_{\lambda, m_\lambda}, \Pi_{\lambda, m'_\lambda}$  restricts the matrix into the irrep  $S^\lambda$  corresponding to the multiplicities  $m_\lambda, m'_\lambda$  respectively. Obviously,  $\Pi_{\lambda, m_\lambda} W = \Pi_{\lambda, m'_\lambda} W$  in terms of their entries, so the last term could be understood as the trace of the matrix product of  $W$  with its conjugate in  $S^\lambda$ . Symbolically, let  $\Pi_{\lambda, m_\lambda, m'_\lambda} = \sum_i E_{(\alpha_i, m_\lambda), (\alpha_i, m'_\lambda)}$ ,

$$\sum_{i,j} W_{(\alpha_j, m_\lambda), (\alpha_i, m_\lambda)}^\dagger W_{(\alpha_i, m'_\lambda), (\alpha_j, m'_\lambda)} = \text{Tr}(\Pi_{\lambda, m_\lambda} W^\dagger \Pi_{\lambda, m_\lambda, m'_\lambda} W). \quad (127)$$

The expansion still contains another two kinds of terms for a pair of inequivalent irreps  $S^\lambda \not\cong S^\mu$ ,

$$\frac{1}{d_\lambda d_\mu} \text{Tr} \left( \left( \sum_{i,j} E_{(\alpha_i^\lambda, m_1), (\alpha_i^\lambda, m_2)} \otimes E_{(\alpha_j^\mu, m'_1), (\alpha_j^\mu, m'_2)} \right) (W^\dagger \otimes W) \right) \left( \sum_{i,j} E_{(\alpha_i^\lambda, m_1), (\alpha_i^\lambda, m_2)} \otimes E_{(\alpha_j^\mu, m'_1), (\alpha_j^\mu, m'_2)} \right), \quad (128)$$

$$\frac{1}{d_\lambda d_\mu} \text{Tr} \left( \left( \sum_{i,j} E_{(\alpha_i^\lambda, m_1), (\alpha_j^\mu, m'_1)} \otimes E_{(\alpha_j^\mu, m'_2), (\alpha_i^\lambda, m_2)} \right) (W^\dagger \otimes W) \right) \left( \sum_{i,j} E_{(\alpha_i^\lambda, m_1), (\alpha_j^\mu, m'_1)} \otimes E_{(\alpha_j^\mu, m'_2), (\alpha_i^\lambda, m_2)} \right). \quad (129)$$

The first remains when  $m_1 = m_2 = m_\lambda, m'_1 = m'_2 = m_\mu$  but the second term always vanishes since  $\sigma$  is block diagonal under Young basis.

To compute

$$\frac{1}{d^n} \int_{U(\oplus_{\lambda} S^\lambda)} \text{Tr} \left( (UW^\dagger U^\dagger) V^\dagger (UWU^\dagger) V \right), \quad (130)$$

we contract the above terms with a general basis operator  $V$  may not respecting the symmetry, which gives

$$\begin{aligned}
& \frac{1}{d_\lambda^2 - 1} \left( \text{Tr}(\Pi_{\lambda, m_\lambda} W^\dagger) \text{Tr}(\Pi_{\lambda, m'_\lambda} W) \text{Tr}(\Pi_{\lambda, m_\lambda} V^\dagger \Pi_{\lambda, m'_\lambda} V) \right. \\
& \quad + \left( \sum_{i,j} W_{(\alpha_j^\lambda, m_\lambda), (\alpha_i^\lambda, m_\lambda)}^\dagger W_{(\alpha_i^\lambda, m'_\lambda), (\alpha_j^\lambda, m'_\lambda)} \right) \left( \sum_{i,j} V_{(\alpha_j^\lambda, m_\lambda), (\alpha_j^\lambda, m'_\lambda)}^\dagger V_{(\alpha_i^\lambda, m'_\lambda), (\alpha_i^\lambda, m_\lambda)} \right) \\
& \quad - \frac{1}{d_\lambda} \text{Tr}(\Pi_{\lambda, m_\lambda} W^\dagger) \text{Tr}(\Pi_{\lambda, m'_\lambda} W) \left( \sum_{i,j} V_{(\alpha_j^\lambda, m_\lambda), (\alpha_j^\lambda, m'_\lambda)}^\dagger V_{(\alpha_i^\lambda, m'_\lambda), (\alpha_i^\lambda, m_\lambda)} \right) \\
& \quad - \frac{1}{d_\lambda} \left( \sum_{i,j} W_{(\alpha_j^\lambda, m_\lambda), (\alpha_i^\lambda, m_\lambda)}^\dagger W_{(\alpha_i^\lambda, m'_\lambda), (\alpha_j^\lambda, m'_\lambda)} \right) \text{Tr}(\Pi_{\lambda, m_\lambda} V^\dagger \Pi_{\lambda, m'_\lambda} V), \\
& = \frac{1}{d_\lambda^2 - 1} \left( \text{Tr}(\Pi_{\lambda, m_\lambda} W^\dagger) \text{Tr}(\Pi_{\lambda, m'_\lambda} W) \text{Tr}(\Pi_{\lambda, m_\lambda} V^\dagger \Pi_{\lambda, m'_\lambda} V) \right. \\
& \quad + \text{Tr}(\Pi_{\lambda, m_\lambda} W^\dagger \Pi_{\lambda, m_\lambda, m'_\lambda} W) \text{Tr}(\Pi_{\lambda, m'_\lambda, m_\lambda} V^\dagger) \text{Tr}(\Pi_{\lambda, m_\lambda, m'_\lambda} V) \\
& \quad - \frac{1}{d_\lambda} \text{Tr}(\Pi_{\lambda, m_\lambda} W^\dagger) \text{Tr}(\Pi_{\lambda, m'_\lambda} W) \text{Tr}(\Pi_{\lambda, m'_\lambda, m_\lambda} V^\dagger) \text{Tr}(\Pi_{\lambda, m_\lambda, m'_\lambda} V) \\
& \quad \left. - \frac{1}{d_\lambda} \text{Tr}(\Pi_{\lambda, m_\lambda} W^\dagger \Pi_{\lambda, m_\lambda, m'_\lambda} W) \text{Tr}(\Pi_{\lambda, m_\lambda} V^\dagger \Pi_{\lambda, m'_\lambda} V), \right.
\end{aligned} \tag{131}$$

with

$$\frac{1}{d_\lambda d_\mu} \text{Tr}(\Pi_{\lambda, m_\lambda} W^\dagger) \text{Tr}(\Pi_{\mu, m_\mu} W) \text{Tr}(\Pi_{\lambda, m_\lambda} V^\dagger \Pi_{\mu, m_\mu} V). \tag{132}$$

As a reminder, if  $S^\lambda$  is the 1-dimensional trivial representation (we omit the 1-dimensional sign representation appears whose occurrence demands  $d \geq n$ ), Eq.(131) degenerates to

$$\text{Tr}(\Pi_\lambda W^\dagger) \text{Tr}(\Pi_\lambda W) \text{Tr}(\Pi_\lambda V^\dagger \Pi_\lambda V) = \text{Tr}(\Pi_\lambda V^\dagger \Pi_\lambda V). \tag{133}$$

Let us comment on each term before proceeding:

1. Matrix products with restricted projections like  $\Pi_{\lambda, m_\lambda}$  have straightforward meaning.
2. As mentioned earlier, Eq.(127) can be seen as the *trace of the matrix product* of copies of  $W^\dagger$  and  $W$  in isomorphic  $S_n$  irrep  $S^\lambda$ , which equals  $\text{Tr}(\Pi_{\lambda, m_\lambda} W^\dagger W)$  quantitatively.
3. Resembling *product of traces*,

$$\sum_{i,j} V_{(\alpha_j^\lambda, m_\lambda), (\alpha_j^\lambda, m'_\lambda)}^\dagger V_{(\alpha_i^\lambda, m'_\lambda), (\alpha_i^\lambda, m_\lambda)} = \text{Tr}(\Pi_{\lambda, m'_\lambda, m_\lambda} V^\dagger) \text{Tr}(\Pi_{\lambda, m_\lambda, m'_\lambda} V) \tag{134}$$

counts off-diagonal entries of  $V$  if  $m_\lambda \neq m'_\lambda$  represents different isomorphic copies of  $S^\lambda$ , which will vanish if  $V$  is  $SU(d)$  symmetric.

We still need summing over all inequivalent irreps with different multiplicities. We now take the convention using  $V = V_r$  as a Pauli basis operator located at the  $r$ th site of the system with

$$W = (i, j) - \frac{1}{d} I = \frac{1}{d} \sum_{P \neq I} P_i \otimes P_j^\dagger, \tag{135}$$

being the conserved quantity determined by SWAPs, or *exchanging interactions* for  $d = 2$ :

$$W = (i, j) - \frac{1}{2} I = \frac{1}{2} \sum_{P \neq I} P_i \otimes P_j^\dagger = 2 \hat{S}_i \cdot \hat{S}_j, \tag{136}$$

where  $\hat{S}_i = \frac{1}{2}(X_i + Y_i + Z_i)$  is the familiar spin operator [54]. In order to make an appropriate comparison with the case when no symmetry is considered,  $\text{Tr}(W) = 0$  is prescribed and we may further multiply  $W$  with the factor  $\frac{1}{\sqrt{1-1/d^2}}$  with which  $\text{Tr}(W^\dagger W) = d^n$ .



As a common property of  $S_n$  group characters [19–21],

$$\left| \text{Tr}(\Pi_{\lambda, m_\lambda} \sigma) \right| = \left| \chi_\lambda(\sigma) \right| \leq d_\lambda \implies \left| \text{Tr}(\Pi_{\lambda, m_\lambda} W) \right| \leq \left(1 - \frac{1}{d}\right) d_\lambda. \quad (137)$$

Moreover, since  $V$  is unitary,

$$0 \leq \text{Tr}(\Pi_{\lambda, m_\lambda} V^\dagger \Pi_{\lambda, m'_\lambda} V) \leq d_\lambda, \quad 0 \leq \text{Tr}(\Pi_{\lambda, m_\lambda} V^\dagger \Pi_{\lambda, m_\mu} V) \leq \min\{d_\lambda, d_\mu\}. \quad (138)$$

Let  $\#(S^\lambda)$  denote the number of multiplicities of  $S^\lambda$ , which equals the dimension of the dual  $SU(d)$  irrep under Schur-Weyl duality. Since there are at most super-polynomially many inequivalent  $S_n$  irreps (see Eq.(7)), the sum of absolute value of the last term in Eq.(131)

$$\frac{1}{d^n} \sum_\lambda \sum_{m_\lambda, m'_\lambda} \frac{1}{d_\lambda^2 - 1} \frac{1}{d_\lambda} \left| \text{Tr}(\Pi_{\lambda, m_\lambda} W^\dagger \Pi_{\lambda, m'_\lambda} W) \right| \text{Tr}(\Pi_{\lambda, m_\lambda} V^\dagger \Pi_{\lambda, m'_\lambda} V) \leq \frac{1}{d^n} \sum_\lambda \frac{\#^2(S^\lambda)}{d_\lambda} \quad (139)$$

decays faster than any inverse polynomial of  $n$ . It would be omitted later after we study the scaling behavior of other terms from Eq.(131) and (132).

As a basic result in  $S_n$  representation theory, except the trivial representation (and sign representation), the second lowest dimension of  $S_n$  irreps is  $n - 1$  [2, 55, 56]. Thus  $d_\lambda^2 - 1 \approx d_\lambda^2$  for nontrivial case and we sum the first term in Eq.(131) with Eq.(132) as

$$\begin{aligned} & \frac{1}{d^n} \left( \sum_\lambda \sum_{m_\lambda, m'_\lambda} \frac{1}{d_\lambda^2} \text{Tr}(\Pi_{\lambda, m_\lambda} W^\dagger) \text{Tr}(\Pi_{\lambda, m'_\lambda} W) \text{Tr}(\Pi_{\lambda, m_\lambda} V_r^\dagger \Pi_{\lambda, m'_\lambda} V_r) \right. \\ & \quad \left. + \sum_{\lambda \neq \mu} \sum_{m_\lambda, m_\mu} \frac{1}{d_\lambda d_\mu} \text{Tr}(\Pi_{\lambda, m_\lambda} W^\dagger) \text{Tr}(\Pi_{\mu, m_\mu} W) \text{Tr}(\Pi_{\lambda, m_\lambda} V_r^\dagger \Pi_{\mu, m_\mu} V_r) \right) \\ &= \frac{1}{d^n} \sum_{\lambda, \mu} \sum_{m_\lambda, m_\mu} \frac{1}{d_\lambda d_\mu} \text{Tr}(\Pi_{\lambda, m_\lambda} W^\dagger) \text{Tr}(\Pi_{\mu, m_\mu} W) \text{Tr}(\Pi_{\lambda, m_\lambda} V_r^\dagger \Pi_{\mu, m_\mu} V_r) \\ &= \frac{1}{d^n} \sum_{\lambda, \mu} \sum_{m_\lambda, m_\mu} \left( \frac{\chi_\lambda(i, j)}{d_\lambda} - \frac{1}{d} \right) \left( \frac{\chi_\mu(i, j)}{d_\mu} - \frac{1}{d} \right) \text{Tr}(\Pi_{\lambda, m_\lambda} V_r^\dagger \Pi_{\mu, m_\mu} V_r). \end{aligned} \quad (140)$$

We are still left with

$$\begin{aligned} & \frac{1}{d^n} \sum_\lambda \sum_{m_\lambda, m'_\lambda} \frac{1}{d_\lambda^2 - 1} \left( \text{Tr}(\Pi_{\lambda, m_\lambda} W^\dagger \Pi_{\lambda, m'_\lambda} W) \text{Tr}(\Pi_{\lambda, m'_\lambda} V_r^\dagger) \text{Tr}(\Pi_{\lambda, m_\lambda} V_r) \right. \\ & \quad \left. - \frac{1}{d_\lambda} \text{Tr}(\Pi_{\lambda, m_\lambda} W^\dagger) \text{Tr}(\Pi_{\lambda, m'_\lambda} W) \text{Tr}(\Pi_{\lambda, m'_\lambda} V_r^\dagger) \text{Tr}(\Pi_{\lambda, m_\lambda} V_r) \right) \\ &= \frac{1}{d^n} \sum_\lambda \sum_{m_\lambda, m'_\lambda} \frac{1}{d_\lambda^2 - 1} \left( d_\lambda - \left(1 - \frac{2}{d}\right) \chi_\lambda(i, j) - \frac{1}{d_\lambda} \chi_\lambda(i, j)^2 \right) \text{Tr}(\Pi_{\lambda, m'_\lambda} V_r^\dagger) \text{Tr}(\Pi_{\lambda, m_\lambda} V_r) \end{aligned} \quad (141)$$

which is nonnegative and we are going to estimate them in turns. One more trick may further simplify the computation is that Pauli matrices are similar under unitary transformation: for any two Pauli matrices  $P, Q$  there exists  $U \in SU(d)$  such that

$$UPU^\dagger = Q \implies \text{Tr}(\tilde{W} Q_r \tilde{W} Q_r) = \text{Tr}(\tilde{W} U^{\otimes n} P_r U^{\dagger \otimes n} \tilde{W} U^{\otimes n} P_r U^{\dagger \otimes n}) = \text{Tr}(\tilde{W} P_r \tilde{W} P_r). \quad (142)$$

because  $W$  as well as its time evolution is assumed to be  $SU(d)$  symmetric. This fact only holds for non-symmetric case after taking Haar average.

### Explicit Computation under $SU(2)$ Symmetry

To make further computation, we have to restrict ourselves to systems of qubits ( $d = 2$ ) because we need calculating terms like  $\text{Tr}(\Pi_{\lambda, m'_\lambda, m_\lambda} V^\dagger)$  under explicit Young basis (total spin basis) constructing by sequential coupling (addition of  $SU(2)$  quantum angular momenta) [5, 57, 58] and evaluating  $\chi_\lambda(i, j)$  in precise. To begin with, as we introduce at the end of Section IA, Lemma I.9 confirms that for two-row Young diagrams  $\lambda = (n - r, r)$ ,

$$\frac{n - 4}{2n - 2} = \chi_{(n/2, n/2)}(i, j) \leq \chi_\lambda(i, j) = \frac{n^2 - (2r + 1)n + 2r^2 - 2r}{n^2 - n} \leq \chi_{(n)}(i, j) = 1. \quad (143)$$

If  $n$  is odd, the lower bound is similar and can be calculated through Eq.(12) or (16). Thus Eq.(140) has non-positive terms due to

$$\left(\frac{\chi_\lambda(i, j)}{d_\lambda} - \frac{1}{2}\right)\left(\frac{\chi_\mu(i, j)}{d_\mu} - \frac{1}{2}\right) \quad (144)$$

when one of the characters is larger than  $\frac{1}{2}$  and the other is lower. The critical point for  $\frac{\chi_\lambda(i, j)}{d_\lambda} - \frac{1}{2} = 0$  happens when  $\lambda = (n - r_0, r_0)$  with

$$r_0 = \frac{n}{2} + \frac{1}{2} - \sqrt{\frac{3n}{4} + \frac{1}{4}}. \quad (145)$$

One the other hand, let  $\lambda = (n - r, r)$  we notice that (we set  $V = Z$  by Eq.(142))

$$\text{Tr}(\Pi_{\lambda, m_\lambda} Z_r^\dagger \Pi_{\mu, m_\mu} Z_r) = 0 \text{ unless } \mu = (n - r - 1, r + 1) \text{ or } (n - r + 1, r - 1). \quad (146)$$

That is,  $\lambda, \mu$  are consecutive two-row Young diagrams with respect to the dominance relation (Definition I.8). To see the reason,

$$\Pi_{\lambda, m_\lambda} \left( \sum_{i=1}^n Z_i \right) \Pi_{\mu, m_\mu} \quad (147)$$

is a zero matrix for any  $\lambda \neq \mu$  because the sum  $\sum_{i=1}^n Z_i$  of spin- $z$  operators is decomposed according to  $SU(2)$  irreps also labeled by  $\lambda, \mu$  by Schur-Weyl duality. Hence

$$\Pi_{\lambda, m_\lambda} Z_n \Pi_{\mu, m_\mu} = -\Pi_{\lambda, m_\lambda} \left( \sum_{i=1}^{n-1} Z_i \right) \Pi_{\mu, m_\mu} \quad (148)$$

is given by the spin- $z$  operator  $\sum_{i=1}^{n-1} Z_i$  on the first  $n - 1$  qubits. From the perspective of either  $SU(2)$  sequential coupling (Clebsch-Gordan decomposition) or  $S_n$  branching rule [2–5], it may have nonzero entries only when  $\lambda, \mu$  are consecutive because this is only way when they share equivalent  $SU(2)$  or  $S_{n-1}$  irreps on  $n - 1$  qubits (this argument fails when  $d \geq 3$  with even intricate branching behavior of Young diagrams). Otherwise, after taking trace,

$$\text{Tr}(\Pi_{\lambda, m_\lambda} Z_n^\dagger \Pi_{\mu, m_\mu} Z_n) = 0 \implies \text{Tr}(\Pi_{\lambda, m_\lambda} Z_r^\dagger \Pi_{\mu, m_\mu} Z_r) = 0 \quad (149)$$

as  $\Pi_{\lambda, m_\lambda}, \Pi_{\mu, m_\mu}$  are invariant under  $S_n$  permutations. Together with the previous analysis on  $S_n$  characters, non-positive terms in Eq.(140) only appear for the following pair of Young diagrams

$$\lambda_0 = (n - \lfloor r_0 \rfloor, \lfloor r_0 \rfloor), \quad \lambda_1 = (n - \lceil r_0 \rceil, \lceil r_0 \rceil). \quad (150)$$

Let  $\epsilon = r_0 - \lfloor r_0 \rfloor \in [0, 1)$ ,

$$\left| \left( \frac{\chi_{\lambda_0}(i, j)}{d_{\lambda_0}} - \frac{1}{2} \right) \left( \frac{\chi_{\lambda_1}(i, j)}{d_{\lambda_1}} - \frac{1}{2} \right) \right| = \frac{4\epsilon(1-\epsilon)(\epsilon + \sqrt{1+3n})(-1 + \epsilon + \sqrt{1+3n})}{n^4 - n^2} = O\left(\frac{1}{n^3}\right). \quad (151)$$

Making use of dimension comparison of  $S_n$  irreps of two-row Young diagram (Eq.(20)), we find that

$$\frac{1}{2^n} d_{\lambda_0} \approx \frac{1}{2^n} d_{\lambda_1} \approx \frac{1}{2^n} \frac{n - 2r_0 + 1}{n - r_0 + 1} \binom{n}{r_0} = \Theta\left(\frac{1}{n}\right). \quad (152)$$

Counting their multiplicity gives  $(n - 2r_0)^2 = \Theta(n)$  approximately and in summary, non-positive terms have the following scaling behavior:

$$\left| \frac{2}{2^n} \sum_{m_{\lambda_0}, m_{\lambda_1}} \left( \frac{\chi_{\lambda_0}(i, j)}{d_{\lambda_0}} - \frac{1}{2} \right) \left( \frac{\chi_{\lambda_1}(i, j)}{d_{\lambda_1}} - \frac{1}{2} \right) \text{Tr}(\Pi_{\lambda_0, m_{\lambda_0}} V_r^\dagger \Pi_{\lambda_1, m_{\lambda_1}} V_r) \right| = O\left(\frac{1}{n^3}\right). \quad (153)$$

We now show that the above non-positive term is dominated by positive terms with  $\lambda = \lambda_0$  in Eq.(141) which equals

$$\frac{1}{2^n} \sum_{m_{\lambda_0}} \frac{1}{d_{\lambda_0}^2 - 1} \left( d_{\lambda_0} - \frac{1}{d_{\lambda_0}} \chi_{\lambda_0}(i, j)^2 \right) \text{Tr}(\Pi_{\lambda, m_{\lambda_0}} Z_r) \text{Tr}(\Pi_{\lambda, m_{\lambda_1}} Z_r) \approx \frac{1}{2^n} \sum_{m_{\lambda_0}} \frac{1}{d_{\lambda_0}^2 - 1} \frac{3}{4} d_{\lambda_0} \text{Tr}(\Pi_{\lambda, m_{\lambda_0}} Z_r) \text{Tr}(\Pi_{\lambda, m_{\lambda_0}} Z_r) \quad (154)$$

for now. We perform a similar but simpler trick, which only depending on the permutation invariance of  $\Pi_{\lambda, m'_\lambda m_\lambda}$  as before:

$$\text{Tr}(\Pi_{\lambda, m'_\lambda m_\lambda} Z_r) = \frac{1}{n} \text{Tr}(\Pi_{\lambda, m'_\lambda m_\lambda} \sum_{i=1}^n Z_i) = \begin{cases} \frac{1}{n} m d_\lambda, & m'_\lambda = m_\lambda, \\ 0, & m'_\lambda \neq m_\lambda, \end{cases} \quad (155)$$

where  $m$  is the spin- $z$  component of basis states determined by the multiplicities  $m_\lambda$ . Suppose  $\lambda = (n - r, r)$ , it ranges among  $n - 2r, n - 2r - 2, \dots, -n + 2r + 2, -n + 2r$ . Let  $r = r_0$ . Substituting the above identity into Eq.(154), plus the previous dimension comparison, we obtain

$$\frac{1}{2^n} \sum_{m_{\lambda_0}} \frac{1}{d_{\lambda_0}^2 - 1} \frac{3}{4} d_{\lambda_0} \text{Tr}(\Pi_{\lambda, m_{\lambda_0}} Z_r) \text{Tr}(\Pi_{\lambda, m_{\lambda_0}} Z_r) \approx \frac{3}{2^{n+2}} \sum_{m=-n+2r_0}^{n-2r_0} \frac{d_\lambda^3}{d_{\lambda_0}^2 - 1} \frac{1}{n^2} m^2 = \Omega\left(\frac{1}{n^{3/2}}\right). \quad (156)$$

Therefore, the desired OTOC of  $W$  describing exchanging interaction, which is estimated by the sum of Eq.(140) and (141), is positive and at least  $\Omega(\frac{1}{n^{3/2}})$ . As a comparison, for general random circuits, as long as  $\text{Tr}(W) = 0, \text{Tr}(W^\dagger W) \leq d^n$ , OTOC always converges to zero exponentially fast with respect to the system size  $n$  (see Eq.(116)). We understand that the current estimation is merely a rough lower bound because there are Young diagrams  $\lambda, \mu \neq \lambda_0, \lambda_1$  remained for computation, which demands more advanced techniques to deal with the above summations and we leave it to future work.

#### OTOC under $SU(d)$ Symmetric Local Operator Basis

Even being able to span any operator acting on the  $d^n$ -dimensional space, generalized Pauli strings does not commute with the  $SU(d)$  tensor product action on qudits. Hence we also discuss conserved quantities spreading evaluated under  $SU(d)$  symmetric basis, which is defined to be an orthogonal basis capable of spanning all  $SU(d)$  symmetric operators. By double commutant theorem [3, 4]

$$\text{span}\{\sigma \in S_n\} = \{M \in \text{End}(H), MU^{\otimes n} = U^{\otimes n}M\}, \quad (157)$$

thus simply conducting Gram-Schmidt orthogonalization to these permutations synthesizes such a basis. Since we only focus on  $SU(d)$  symmetric local operators, especially those 2-local ones, we focus on the following basis elements:

$$\{I, \frac{1}{\sqrt{1-1/d^2}}(\tau - \frac{1}{d}I); \tau = (i, j) \in S_n\}. \quad (158)$$

Coincidentally, a single basis element  $\frac{1}{\sqrt{1-1/d^2}}(\tau - \frac{1}{d}I)$  is also taken as a conserved quantity before.

Applying Eq.(131) with the fact that  $\chi_\lambda$  is invariant for permutations of the same cycle type (Definition I.3), we abbreviate  $\chi_\lambda(i, j) = \chi_\lambda, \bar{\chi}_\lambda = \frac{\chi_\lambda}{d_\lambda}$  and obtain the following expansion:

$$\begin{aligned} \text{OTOC}_{\text{sym}} &= \frac{1}{d^n} \sum_{\lambda} \frac{\#(S^\lambda)}{d_\lambda^2 - 1} \frac{1}{1 - 1/d^2} \left( \left( \chi_\lambda - \frac{d_\lambda}{d} \right)^2 \left( \left( 1 + \frac{1}{d^2} \right) d_\lambda - \frac{2}{d} \chi_\lambda \right) + \left( \left( 1 + \frac{1}{d^2} \right) d_\lambda - \frac{2}{d} \chi_\lambda \right) \left( \chi_\lambda - \frac{d_\lambda}{d} \right)^2 \right. \\ &\quad \left. - \frac{1}{d_\lambda} \left( \chi_\lambda - \frac{d_\lambda}{d} \right)^4 - \frac{1}{d_\lambda} \left( \left( 1 + \frac{1}{d^2} \right) d_\lambda - \frac{2}{d} \chi_\lambda \right)^2 \right) \\ &= \frac{1}{d^n} \sum_{\lambda} \frac{\#(S^\lambda) d_\lambda^3}{d_\lambda^2 - 1} \frac{d^2}{d^2 - 1} \left( \left( \bar{\chi}_\lambda - \frac{1}{d} \right)^2 \left( 2 + \frac{1}{d^2} - \frac{2}{d} \bar{\chi}_\lambda - \bar{\chi}_\lambda^2 \right) - \frac{1}{d_\lambda^2} \left( 1 + \frac{1}{d^2} - \frac{2}{d} \bar{\chi}_\lambda \right)^2 \right) \\ &\approx \frac{1}{d^n} \sum_{\lambda} \#(S^\lambda) d_\lambda \frac{d^2}{d^2 - 1} \left( \bar{\chi}_\lambda - \frac{1}{d} \right)^2 \left( 2 + \frac{1}{d^2} - \frac{2}{d} \bar{\chi}_\lambda - \bar{\chi}_\lambda^2 \right) \end{aligned} \quad (159)$$

where we omit the last term as analogy to what we did in Eq.(139). As mentioned before, if  $S^\lambda$  is the 1-dimensional trivial representation,  $\bar{\chi}_\lambda = 1$  and we write

$$\text{Tr}(\Pi_\lambda W^\dagger) \text{Tr}(\Pi_\lambda W) \text{Tr}(\Pi_\lambda V^\dagger \Pi_\lambda V) = \left( 1 - \frac{1}{d} \right)^4 \quad (160)$$

which is already incorporated into the above approximation. Note that each term is positive now. To lower bound the OTOC under local symmetric basis, we take a closer look at the irrep  $S^\lambda$  for which

$$\lambda = \left( \frac{n-k}{d} + k, \frac{n-k}{d}, \dots, \frac{n-k}{d} \right) \quad (161)$$

where  $k$  is taken from  $\{0, \dots, d-1\}$  such that  $n-k$  can be divided by  $d$ . By Eq.(12),

$$\bar{\chi}_\lambda = -\frac{(d-1)((d-1)n - kd - k^2)}{n(n-1)d} \implies \left(\bar{\chi}_\lambda - \frac{1}{2}\right)^2 = \Theta\left(\frac{1}{n^2}\right). \quad (162)$$

Let  $\lambda_0 = (\frac{n-k}{d}, \frac{n-k}{d}, \dots, \frac{n-k}{d})$  obtained from  $\lambda$  by discarding  $k$  boxes from its first row. Assume  $d \leq \frac{n-k}{d}$ , the  $S_{n-k}$  irrep  $S^{\lambda_0}$  is obviously contained in  $S^\lambda$ . Then Eq.(21) indicates that

$$d_\lambda > d_{\lambda_0} \geq \frac{d^{n-k}}{(n-k)^{d(d+2)/2}} > \frac{d^n}{n^{d(d+4)/2}}. \quad (163)$$

On the other hand,

$$\min_\lambda \left(2 + \frac{1}{d^2} - \frac{2}{d}\bar{\chi}_\lambda - \bar{\chi}_\lambda^2\right) = \left(1 - \frac{1}{d}\right)^2, \quad (164)$$

where the minimum is attained on the trivial irrep. Therefore,

$$\text{OTOC}_{\text{sym}} \geq \frac{1}{d^n} d_\lambda \frac{d^2}{d^2 - 1} \left(\bar{\chi}_\lambda - \frac{1}{d}\right)^2 \left(1 - \frac{1}{d}\right)^2 = \Omega\left(\frac{1}{n^{(d+2)^2/2}}\right). \quad (165)$$

We wish to note that the calculation is not tight. In the case of qubit, it is still possible to further refine the above lower bound. We first carefully check the scaling behavior of characters of  $\lambda = \lambda_0$  or  $\lambda_1$  defined in (150):

$$\bar{\chi}_{\lambda_0} - \frac{1}{2} = \frac{2\epsilon(\sqrt{3n+1} + \epsilon)}{n^2 - n}, \quad \bar{\chi}_{\lambda_1} - \frac{1}{2} = -\frac{2(1-\epsilon)(\sqrt{3n+1} - 1 + \epsilon)}{n^2 - n}, \quad (166)$$

where we recall that  $\epsilon = r_0 - \lfloor r_0 \rfloor \in [0, 1)$ . We claim that at least one of these two  $S_n$  irrep sectors, together with all other sectors corresponding to two-row Young diagrams from  $n$ -qubit system satisfies

$$\left(\bar{\chi}_\lambda - \frac{1}{2}\right)^2 = \Omega\left(\frac{1}{n^3}\right). \quad (167)$$

Plugging into Eq.(159), we conclude that

$$\text{OTOC}_{\text{sym}} = \left(\frac{1}{2^n} \sum_{\lambda \neq \lambda_0} \#(S^\lambda) d_\lambda\right) \Omega\left(\frac{1}{n^3}\right) = \Omega\left(\frac{1}{n^3}\right) \quad (168)$$

where  $S^{\lambda_0}$  is omitted because  $\left(\bar{\chi}_{\lambda_0} - \frac{1}{2}\right)^2$  is assumed to be even smaller than the given scaling. Then the sum is solved using  $\sum_\lambda \#(S^\lambda) d_\lambda = 2^n$  by definition and

$$\frac{1}{2^n} d_{\lambda_0} = \Theta\left(\frac{1}{n}\right), \quad \#(S^{\lambda_0}) = \Theta(\sqrt{n}) \quad (169)$$

clarified in the previous subsection.

To demonstrate Eq.(167), we find by (143) that given any  $\epsilon \in [0, 1)$  the squares of

$$\bar{\chi}_{\lambda_2} - \frac{1}{2} = \frac{2(1+\epsilon)(\sqrt{3n+1} + 1 + \epsilon)}{n^2 - n}, \quad \bar{\chi}_{\lambda_3} - \frac{1}{2} = -\frac{2(2-\epsilon)(\sqrt{3n+1} - 2 + \epsilon)}{n^2 - n} \quad (170)$$

are  $\Omega\left(\frac{1}{n^3}\right)$  for

$$\lambda_2 := (n - \lfloor r_0 \rfloor + 1, \lfloor r_0 \rfloor - 1), \quad \lambda_3 := (n - \lceil r_0 \rceil - 1, \lceil r_0 \rceil + 1). \quad (171)$$

Other cases follows immediately by the frequently used fact that two-row Young diagrams, as well as the corresponding  $S_n$  characters, are totally ordered (Lemma I.9).

### C. Spreading of Local U(1) Conserved Quantities

The expansion of  $T_{k=2}^{\text{COA}}$  (Eq.(120) and (121)) as well as its restriction to conserved quantity (Eq.(131) and (132)) formally works for arbitrary compact Lie group  $G$  acting on an  $n$ -qudit system with the following generic irrep decomposition

$$H = V^{\otimes n} \cong \bigoplus_{\lambda} I_{m_{\lambda}} \otimes S^{\lambda} \quad (172)$$

where  $S^{\lambda}$  here denotes one irrep of  $G$  and  $I_{m_{\lambda}}$  denotes its multiplicities space. As a concrete example, let us compute the OTOC of  $W = (i, j) - \frac{1}{2}I$  under U(1) symmetry, where the concerned group  $G$  consists of all unitaries  $U$  for which

$$[U, \sum_i \frac{Z_i + I}{2}] = 0 \Leftrightarrow [U, \sum_i Z_i] = 0. \quad (173)$$

Accordingly, U(1) charge sectors are subspaces of quantum states with the same spin- $z$  components or magnetic quantum numbers. Under computational basis,

$$H = V^{\otimes n} \cong \bigoplus_{k=0}^n S^k, \quad S^k = \text{span}\{|i_1, \dots, i_n\rangle; k \text{ many of them equal } 0\}. \quad (174)$$

and there is obviously no nontrivial multiplicities space. Rewriting Eq.(131) and (132) for U(1) symmetry, we have

$$\begin{aligned} & \frac{1}{d_k^2 - 1} \left( \text{Tr}(\Pi_k W^\dagger) \text{Tr}(\Pi_k W) \text{Tr}(\Pi_k V^\dagger \Pi_k V) + \text{Tr}(\Pi_k W^\dagger \Pi_k W) \text{Tr}(\Pi_k V^\dagger) \text{Tr}(\Pi_k V) \right. \\ & \left. - \frac{1}{d_k} \text{Tr}(\Pi_k W^\dagger) \text{Tr}(\Pi_k W) \text{Tr}(\Pi_k V^\dagger) \text{Tr}(\Pi_k V) - \frac{1}{d_k} \text{Tr}(\Pi_k W^\dagger \Pi_k W) \text{Tr}(\Pi_k V^\dagger \Pi_k V) \right), \end{aligned} \quad (175)$$

with

$$\frac{1}{d_k d_l} \text{Tr}(\Pi_k W^\dagger) \text{Tr}(\Pi_l W) \text{Tr}(\Pi_k V^\dagger \Pi_l V). \quad (176)$$

With no necessity to care about multiplicities, these expansions looks more like that for the second moment over  $U(d^n)$  (see Eq.(112)). As a caveat, the argument using unitary similar transformation Eq.(142) does not hold here even after we average over U(1) symmetric Haar randomness, so we need to calculate for  $V = X, Y, Z$  independently (but the position of one-qubit Pauli operators is still insignificant).

When  $V = Z$ ,  $\Pi_k V \Pi_l V = 0$  unless  $k = l$ , so we simply calculate Eq.(175):

$$\text{Tr}(\Pi_k Z \Pi_k Z) = \text{Tr}(\Pi_k Z^2) = d_k = \binom{n}{k}, \quad \text{Tr}(\Pi_k Z) = \binom{n-1}{k-1} - \binom{n-1}{k} = \frac{2k-n}{n} \binom{n}{k}. \quad (177)$$

and

$$\text{Tr}(\Pi_k W^\dagger) = \text{Tr}\left(\Pi_k \left((i, j) - \frac{1}{2}I\right)\right) = \binom{n-2}{k-2} + \binom{n-2}{k} - \frac{1}{2} \binom{n}{k} = \frac{4k^2 - 4kn + n(n-1)}{2n(n-1)} \binom{n}{k}, \quad (178)$$

$$\text{Tr}(\Pi_k W^\dagger \Pi_k W) = \text{Tr}\left(\Pi_k \left((i, j) - \frac{1}{2}I\right)^2\right) = \frac{5}{4} \binom{n}{k} - \binom{n-2}{k-2} - \binom{n-2}{k} = \frac{-8k^2 + 8kn + n(n-1)}{4n(n-1)} \binom{n}{k}. \quad (179)$$

Before taking total summation, we check the last term in Eq.(175):

$$\begin{aligned} \sum_{k=1}^{n-1} \frac{1}{d_k^2 - 1} \frac{1}{d_k} \text{Tr}(\Pi_k W^\dagger \Pi_k W) \text{Tr}(\Pi_k V^\dagger \Pi_k V) &= \sum_{k=1}^{n-1} \frac{1}{d_k^2 - 1} \frac{1}{d_k} \frac{-8k^2 + 8kn + n(n-1)}{4n(n-1)} \binom{n}{k}^2 \\ &\approx \sum_{k=1}^{n-1} \frac{1}{\binom{n}{k}} \frac{-8k^2 + 8kn + n(n-1)}{4n(n-1)} \end{aligned} \quad (180)$$

which decays faster than any inverse polynomial after being normalized by the factor  $1/2^n$ . Other terms are approximately gathered to

$$\begin{aligned}
& \sum_{k=0}^n \frac{1}{d_k^2} \left( \left( \frac{4k^2 - 4kn + n(n-1)}{2n(n-1)} \binom{n}{k} \right)^2 \binom{n}{k} + \left( \frac{-8k^2 + 8kn + n(n-1)}{4n(n-1)} \binom{n}{k} \right) \left( \frac{2k-n}{n} \binom{n}{k} \right)^2 \right. \\
& \quad \left. - \frac{1}{d_k} \left( \frac{4k^2 - 4kn + n(n-1)}{2n(n-1)} \binom{n}{k} \right)^2 \left( \frac{2k-n}{n} \binom{n}{k} \right)^2 \right) \\
&= \sum_{k=0}^n \left( \left( \frac{4k^2 - 4kn + n(n-1)}{2n(n-1)} \right)^2 + \left( \frac{-8k^2 + 8kn + n(n-1)}{4n(n-1)} \right) \left( \frac{n-2k}{n} \right)^2 - \left( \frac{4k^2 - 4kn + n(n-1)}{2n(n-1)} \right)^2 \left( \frac{n-2k}{n} \right)^2 \right) \binom{n}{k} \\
&= \frac{2^{n-1}}{(n-1)n} + \frac{2^{n-2}(3n-4)}{n^2} - \frac{2^{n-1}(5n-8)}{(n-1)n^3} = \frac{3n^3 - 5n^2 - 6n + 16}{n^3(n-1)} 2^{n-2}. \tag{181}
\end{aligned}$$

This summation is solved by noticing that for fixed  $n$ , each term from above is merely a polynomial of  $k$  with degree no more than 4 product with  $\binom{n}{k}$ . To solve them, we use

$$\sum_{k=0}^n \binom{n}{k} e^{kx} = (1 + e^x)^n, \quad \frac{d}{dx^r} \Big|_{x=0} \sum_{k=0}^n \binom{n}{k} e^{kx} = \sum_{k=0}^n k^r \binom{n}{k}. \tag{182}$$

When  $V = X, Y$ ,  $\Pi_k V = 0$  by definition, so we simply calculate Eq.(176):

$$\text{Tr}(\Pi_k X \Pi_l X) = \text{Tr}(\Pi_k Y \Pi_l Y) = \begin{cases} \binom{n-1}{k-1} = \frac{k}{n} \binom{n}{k}, & l = k-1, \\ \binom{n-1}{k} = \frac{n-k}{n} \binom{n}{k}, & l = k+1, \\ 0, & \text{otherwise.} \end{cases} \tag{183}$$

with  $\text{Tr}(\Pi_k W^\dagger)$  being given above. For either  $X$  or  $Y$ , Eq.(176) equals

$$\begin{aligned}
& \sum_{k=0}^{n-1} \frac{1}{\binom{n}{k} \binom{n}{k+1}} \left( \frac{4k^2 - 4kn + n(n-1)}{2n(n-1)} \binom{n}{k} \right) \left( \frac{4(k+1)^2 - 4(k+1)n + n(n-1)}{2n(n-1)} \binom{n}{k+1} \right) \left( \frac{n-k}{n} \binom{n}{k} \right) \\
& \quad + \sum_{k=0}^{n-1} \frac{1}{\binom{n}{k+1} \binom{n}{k}} \left( \frac{4(k+1)^2 - 4(k+1)n + n(n-1)}{2n(n-1)} \binom{n}{k+1} \right) \left( \frac{4k^2 - 4kn + n(n-1)}{2n(n-1)} \binom{n}{k} \right) \left( \frac{k}{n} \binom{n}{k} \right) \\
&= \sum_{k=0}^{n-1} \left( \frac{4k^2 - 4kn + n(n-1)}{2n(n-1)} \right) \left( \frac{4(k+1)^2 - 4(k+1)n + n(n-1)}{2n(n-1)} \right) \binom{n}{k} \\
&= \frac{1}{n(n-1)} 2^{n-1} - \frac{n^2 + 3n + 4}{4n(n-1)} \tag{184}
\end{aligned}$$

In conclusion, the OTOC of  $W = (i, j) - \frac{1}{2}I$  under U(1) symmetry approximates

$$\frac{1}{3 \cdot 2^n} \left( \frac{3n^3 - 3n^2 - 6n + 16}{n^3(n-1)} 2^{n-2} - \frac{n^2 + 3n + 4}{4n(n-1)} \right) = \frac{3n^3 - 3n^2 - 6n + 16}{12n^3(n-1)} - \frac{n^2 + 3n + 4}{3n(n-1)2^n} = \Theta\left(\frac{1}{n}\right) \tag{185}$$

for large  $n$ .

#### D. SU( $d$ ) Covariant Error Correction Code

We estimate the *Choi error* of SU( $d$ ) covariant quantum error correction codes using computational techniques developed before. To be specific, we follow [35] and consider a system  $S$  of  $n$  qudits where we wish to encode the logical information from a logical space of  $k$  qudits and then decode it. The procedure is mathematically described similarly as in Section III A where we have logical states  $\rho_{R \cup A}$  entangled with the reference  $R$  and another initial state  $\rho_{\bar{A}}$  with no memory for now but commutes with  $U^{\dagger \otimes n-k}$  for any  $U \in \text{SU}(d)$ . Then given a global SU( $d$ ) symmetric unitary  $U$  acting on the system (with identity map acting on the reference), the following SU( $d$ ) *equivariance* or *covariance* is satisfied:

$$\begin{aligned}
U^{\otimes n} U \rho_{R \cup A} \otimes \rho_{\bar{A}} U^\dagger U^{\dagger \otimes n} &= U (U^{\otimes n} \rho_{R \cup A} \otimes \rho_{\bar{A}} U^{\dagger \otimes n}) U^\dagger = U (U^{\otimes k} \rho_{R \cup A} U^{\dagger \otimes k}) \otimes (U^{\otimes n-k} \rho_{\bar{A}} U^{\dagger \otimes n-k}) U^\dagger \\
&= U (U^{\otimes k} \rho_{R \cup A} U^{\dagger \otimes k}) \otimes \rho_{\bar{A}} U^\dagger. \tag{186}
\end{aligned}$$

As an immediate result from Schur-Weyl duality and double commutant theorem (see Section IB or [3, 4] for more details),  $\rho_{\bar{A}}$  is generally expanded as

$$\rho_{\bar{A}} = \sum_i p_i \sigma_{\bar{A},i}, \quad (187)$$

where the combination coefficients satisfy  $\sum_i p_i \text{Tr}(\sigma_{\bar{A},i}) = 1$  with other conditions making  $\rho_{\bar{A}}$  a valid density matrix. For instance, it can be defined by SWAPs

$$\rho_{\bar{A}} = \frac{1}{d^{n-k-1} + d^{n-k}} ((i, j) + I_{\bar{A}}). \quad (188)$$

or more generally,

$$\rho_{\bar{A}} = \frac{1}{2(d^{\#\text{cycles}(\sigma_{\bar{A}})} + d^{n-k})} (\sigma_{\bar{A}} + I_{\bar{A}})(\sigma_{\bar{A}}^{-1} + I_{\bar{A}}) = \frac{1}{2(d^{\#\text{cycles}(\sigma_{\bar{A}})} + d^{n-k})} (\sigma_{\bar{A}} + \sigma_{\bar{A}}^{-1} + 2I_{\bar{A}}) \quad (189)$$

where  $\#\text{cycles}(\sigma_{\bar{A}})$  counts the number of cycles (including trivial 1-cycles) of  $\sigma$  on  $n - k$  qudits. Even might be surprising at the first glance, it can also be crafted into the following form:

$$\rho_{\bar{A}} = \frac{1}{\#(S_0^\lambda)} I_{W_{\lambda_0}} \otimes |\psi_{\lambda_0}\rangle \langle \psi_{\lambda_0}| \quad (190)$$

with  $|\psi_{\lambda}\rangle$  being a pure state (e.g., a Young basis element) restricted to a certain  $S_{n-k}$  irrep of Young diagram  $\lambda_0$  and  $I_{W_{\lambda_0}}$  being the identity matrix recording its multiplicities according to Schur-Weyl duality Eq.(24). This perspective is used later when computing Eq.(198).

Then we decode the processed information by a decoding map  $\mathcal{D}$  acting on  $n - t$  qudits, denoted by  $B$ , of the system. Our objective is appraising the performance the code by calculating the Choi error

$$F_{\text{Choi}} = \max_{\mathcal{D}} F((\text{id}_R \otimes \mathcal{D}) \text{Tr}_B(U \rho_{R \cup A} \otimes \mu_{\bar{A}} U^\dagger), \rho_{R \cup A}), \quad (191)$$

$$\epsilon_{\text{Choi}} = \sqrt{1 - F_{\text{Choi}}^2} = \min_{\mathcal{D}} P((\text{id}_R \otimes \mathcal{D}) \text{Tr}_B(U \rho_{R \cup A} \otimes \mu_{\bar{A}} U^\dagger), \rho_{R \cup A}), \quad (192)$$

where  $\rho_{R \cup A}$  is assumed to be maximally entangled and  $F(\rho, \sigma) = \text{Tr} \sqrt{\sqrt{\rho} \sigma \sqrt{\rho}}$  is the *state fidelity with purified distance*  $P(\rho, \sigma) = \sqrt{1 - F(\rho, \sigma)^2}$ .

Using the so-called *complementary channel formalism* [35, 59], we have

$$\min_{\mathcal{D}} P((\text{id}_R \otimes \mathcal{D}) \text{Tr}_B(U \rho_{R \cup A} \otimes \mu_{\bar{A}} U^\dagger), \rho_{R \cup A}) = \min_{\zeta} P(\text{Tr}_B(U \rho_{R \cup A} \otimes \mu_{\bar{A}} U^\dagger), \text{Tr}_A(\rho_{R \cup A}) \otimes \zeta), \quad (193)$$

where  $\zeta$  is a variable density matrix to minimize the concerned purified distance. For maximally entangled state,  $\text{Tr}_A(\rho_{R \cup A}) = \frac{1}{d_A} I_R$ . Let us denote  $\text{Tr}_B(U \rho_{R \cup A} \otimes \mu_{\bar{A}} U^\dagger)$  by  $\rho_{R \cup B}$ . By triangular inequality

$$\begin{aligned} \epsilon_{\text{Choi}} &= \min_{\zeta} P(\rho_{R \cup B}, \frac{1}{d_A} I_R \otimes \zeta) \leq P(\rho_{R \cup B}, \rho_{R \cup B, \text{avg}}) + \min_{\zeta} P(\rho_{R \cup B, \text{avg}}, \frac{1}{d_A} I_R \otimes \zeta) \\ &\leq \sqrt{2 \|\rho_{R \cup B} - \rho_{R \cup B, \text{avg}}\|_1} + \min_{\zeta} P(\rho_{R \cup B, \text{avg}}, \frac{1}{d_A} I_R \otimes \zeta), \end{aligned} \quad (194)$$

with  $\rho_{R \cup B, \text{avg}} = \int \rho_{R \cup B} dU$  being averaged over the group  $U(\bigoplus_{\lambda} S^{\lambda})$  of  $\text{SU}(d)$  symmetric unitaries. We divide the following context into two part to calculate the second term on the RHS of the above inequality, which is just a constant and to average the first term to obtain the expectation of  $\epsilon_{\text{Choi}}$ .

#### Computation of $\rho_{R \cup B, \text{avg}}^2$

To illustrate the idea, we assume that the erasure part  $\bar{B}$  contains one qudit ( $t = 1$ ) while  $A$  is allowed to encode arbitrary  $k$  qudits (later we shall assume that  $k = o(n)$ ). By comparing commutant algebras (Section II), the 1-design projection  $T_{k=1}^{\text{Haar}} = T_{k=1}^{\text{CQA}}$  can be easily replaced by that using  $S_n$  group elements (however this is not true for higher order moments), so

$$\rho_{R \cup B \cup \bar{B}, \text{avg}} = \frac{1}{n!} \sum_{\sigma \in S_n} \sigma(\rho_{R \cup A} \otimes \rho_{\bar{A}}) \sigma^{-1} = \frac{1}{n!} \sum_i p_i \sigma(\rho_{R \cup A} \otimes \sigma_{\bar{A},i}) \sigma^{-1}. \quad (195)$$



Let  $\rho_{R \cup \{i_1, \dots, i_k\}}$  denotes the maximally entangled state of  $R$  and sites  $i_1, \dots, i_k$  permuted from  $A$ . The above expansion can be divided into two cases depending on whether  $\{i_1, \dots, i_k\} \cap \bar{B}$  is  $\emptyset$  or not. For nonempty case, taking partial trace over  $B$  yields

$$\frac{1}{n} \sum_{a=1}^k \rho_{R \cup \bar{B}, a} \quad (196)$$

where  $\rho_{R \cup \bar{B}, a}$  is defined as when the  $a$ th qudit in  $A$  being permuted to  $\bar{B}$  with all left ones getting traced out. We instantiate the case when  $a = 1$ :

$$\begin{aligned} \rho_{R \cup \bar{B}, 1} &= \text{Tr}_{2, \dots, k} \left( \frac{1}{d^k} \sum_{i_1, \dots, i_k, j_1, \dots, j_k} |i_1^R i_2^R \dots i_k^R, i_1^A i_2^A \dots i_k^A\rangle \langle j_1^R j_2^R \dots j_k^R, j_1^A j_2^A \dots j_k^A| \right) \\ &= \frac{1}{d^{k-1}} \sum_{i_1, \dots, i_k, j_1, \dots, j_k} |i_1^R i_2^R \dots i_k^R, i_1^A\rangle \langle j_1^R i_2^R \dots i_k^R, j_1^A| \\ &= \left( \frac{1}{d} \sum_{i, j} |i_1^R, i_1^A\rangle \langle j_1^R, j_1^A| \right) \frac{1}{d^{k-1}} \sum_{i_2, \dots, i_k} |i_2^R \dots i_k^R\rangle \langle i_2^A \dots i_k^A| \end{aligned} \quad (197)$$

which equals the maximal entangled state between  $a$ th register in  $R$  with  $\bar{B}$  coupled with the maximally mixed state for remaining qudits in  $R$ .

When  $\{i_1, \dots, i_k\} \cap \bar{B} = \emptyset$ , we expand  $\rho_{\bar{A}}$  by Eq.(187) and analyze partial trace for arbitrary permutations  $\sigma_{\bar{A}, i}$ :

$$\begin{aligned} \text{Tr}_B \left( \sigma(\rho_{R \cup A} \otimes \sigma_{\bar{A}, i}) \sigma^{-1} \right) &= \frac{1}{d^k} I_R \otimes d^{\#\text{cycles}(\sigma_{\bar{A}, i})-1} I_{\bar{B}} = d^{\#\text{cycles}(\sigma_{\bar{A}, i})} \frac{1}{d^k} I_R \otimes \frac{1}{d} I_{\bar{B}} \\ \implies \text{Tr}_B \left( \sigma(\rho_{R \cup A} \otimes \rho_{\bar{A}}) \sigma^{-1} \right) &= \sum_i p_i d^{\#\text{cycles}(\sigma_{\bar{A}, i})} \frac{1}{d^k} I_R \otimes \frac{1}{d} I_{\bar{B}} = \frac{1}{d^k} I_R \otimes \frac{1}{d} I_{\bar{B}}. \end{aligned} \quad (198)$$

Therefore,

$$\rho_{R \cup \bar{B}, \text{avg}} = \frac{1}{n} \sum_{a=1}^k \rho_{R \cup \bar{B}, a} + \frac{n-k}{n} \frac{1}{d^k} I_R \otimes \frac{1}{d} I_{\bar{B}} = \frac{1}{n} \sum_{a=1}^k \frac{1}{d^{k-1}} I_{R-a} \otimes |\Psi_{a, \bar{B}}\rangle \langle \Psi_{a, \bar{B}}| + \frac{n-k}{n} \frac{1}{d^k} I_R \otimes \frac{1}{d} I_{\bar{B}} \quad (199)$$

where  $|\Psi_{a, \bar{B}}\rangle$  denotes the maximal entangled state. Let  $k = 1$ , the above result is already obtained in [35] with further computation demonstrating that

$$\mathbb{E}_{\text{Choi}} \leq \frac{\sqrt{d^2 - 1}}{2n} + O(n^{-2}). \quad (200)$$

Let  $\zeta = \frac{1}{d} I_{\bar{B}}$ , by Eq.(191) and (193),

$$\begin{aligned} F(\rho_{R \cup \bar{B}, \text{avg}}, \frac{1}{d_A} I_R \otimes \zeta) &= \text{Tr} \sqrt{\sqrt{\frac{1}{d_A} I_R \otimes \frac{1}{d} I_{\bar{B}}} \rho_{R \cup \bar{B}, \text{avg}} \sqrt{\frac{1}{d_A} I_R \otimes \frac{1}{d} I_{\bar{B}}}} = \text{Tr} \left( \sqrt{\frac{1}{d^{k+1}} \rho_{R \cup \bar{B}, \text{avg}}} \right) \\ \implies P(\rho_{R \cup \bar{B}, \text{avg}}, \frac{1}{d_A} I_R \otimes \zeta) &= \sqrt{1 - \frac{1}{d^{k+1}} \text{Tr}(\sqrt{\rho_{R \cup \bar{B}, \text{avg}}})^2}. \end{aligned} \quad (201)$$

To estimate the trace of the square root of  $\rho_{R \cup \bar{B}, \text{avg}}$ , we take the following strategy using a kind of matrix *arithmetical mean - quadratic mean inequality*. Let  $A_1, A_2$  be positive semidefinite matrices. Then

$$A_1^2 + A_2^2 - \frac{1}{2}(A_1 + A_2)^2 = \frac{1}{2}(A_1^2 + A_2^2 - A_1 A_2 - A_2 A_1) = \frac{1}{2}(A_1 - A_2)^2 \geq 0 \quad (202)$$

$$\implies A_1^2 + A_2^2 \geq \frac{1}{2}(A_1 + A_2)^2, \quad (203)$$

where  $A \geq B$  means  $A - B$  is positive semidefinite. Inductively, we assume

$$\sum_{i=1}^k A_i^2 \geq \frac{1}{k} \left( \sum_{i=1}^k A_i \right)^2. \quad (204)$$

The inequality for  $k + 1$  follows directly by simplifying

$$k(A_1^2 + A_2^2 + \dots + A_{k-1}^2 + A_k^2) + (A_1^2 + \dots + A_{k-1}^2 + A_{k+1}^2) + \dots + (A_2^2 + \dots + A_{k-1}^2 + A_k^2) \geq ((A_1 + \dots + A_{k-1} + A_k)^2 + (A_1 + \dots + A_{k-1} + A_{k+1})^2 + \dots + (A_2 + \dots + A_{k-1} + A_k)^2). \quad (205)$$

To cope with our problem, we rewrite

$$\begin{aligned} \rho_{R \cup \bar{B}, \text{avg}} &= \frac{1}{n} \sum_{a=1}^k \frac{1}{d^{k-1}} I_{R-a} \otimes |\Psi_{a, \bar{B}}\rangle \langle \Psi_{a, \bar{B}}| + \frac{n-k}{n} \frac{1}{d^k} I_R \otimes \frac{1}{d} I_{\bar{B}} \\ &= \frac{1}{k} \sum_{a=1}^k \left( \frac{k}{n} \frac{1}{d^{k-1}} I_{R-a} \otimes |\Psi_{a, \bar{B}}\rangle \langle \Psi_{a, \bar{B}}| + \frac{n-k}{n} \frac{1}{d^k} I_R \otimes \frac{1}{d} I_{\bar{B}} \right) \\ &= \sum_{i=1}^k P_i. \end{aligned} \quad (206)$$

Substituting  $A_i$  by  $\sqrt{P_i}$ , we have

$$\sum_{i=1}^k P_i \geq \frac{1}{k} \left( \sum_{i=1}^k \sqrt{P_i} \right)^2. \quad (207)$$

Since  $A \geq B$  indicates that  $\lambda_i(A) \geq \lambda_i(B)$  when the eigenvalues are ordered in the same way. Taking square root on both sides from above, we can confirm that

$$\text{Tr}(\sqrt{\rho_{R \cup \bar{B}, \text{avg}}}) = \text{Tr}\left(\sqrt{\sum_{i=1}^k P_i}\right) \geq \frac{1}{\sqrt{k}} \text{Tr}\left(\sum_{i=1}^k \sqrt{P_i}\right) = \frac{1}{\sqrt{k}} \sum_{i=1}^k \text{Tr}(\sqrt{P_i}). \quad (208)$$

It is straightforward to evaluate, by definition, that

$$\text{Tr}(\sqrt{P_i}) = \frac{1}{\sqrt{k}} \left( \sqrt{\frac{k}{n} \frac{1}{d^{k-1}} + \frac{n-k}{n} \frac{1}{d^{k+1}}} d^{k-1} + \sqrt{\frac{n-k}{n} \frac{1}{d^{k+1}}} (d^{k+1} - d^{k-1}) \right) \quad (209)$$

for any  $i = 1, \dots, k$ . Thus taking large  $n$  limit,

$$\begin{aligned} \sqrt{1 - \frac{1}{d^{k+1}} \text{Tr}(\sqrt{\rho_{R \cup \bar{B}, \text{avg}}})^2} &\leq \sqrt{1 - \frac{1}{d^{k+1}} \left( \sqrt{\frac{k}{n} \frac{1}{d^{k-1}} + \frac{n-k}{n} \frac{1}{d^{k+1}}} d^{k-1} + \sqrt{\frac{n-k}{n} \frac{1}{d^{k+1}}} (d^{k+1} - d^{k-1}) \right)^2} \\ &= \sqrt{1 - \frac{1}{d^2} \left( \sqrt{\frac{k}{n} + \frac{n-k}{n} \frac{1}{d^2}} + \sqrt{\frac{n-k}{n} \frac{1}{d^2}} (d^2 - 1) \right)^2} \leq \frac{\sqrt{d^2 - 1}k}{2n}. \end{aligned} \quad (210)$$

*Remark.* One potential issue to generalize  $\bar{B}$  to arbitrary  $t$  qudits occurs when computing Eq.(198): if  $t > 1$ , the form of  $\text{Tr}_B(\sigma(\rho_{R \cup A} \otimes \sigma_{\bar{A}, i}) \sigma^{-1})$  becomes depending on the intersection of  $\bar{B}$  and the *nontrivial support* of  $\sigma \sigma_{\bar{A}, i} \sigma^{-1}$ . If the interaction contains at most one qudits, the result is the same as before. Otherwise, after taking partial trace,  $\sigma \sigma_{\bar{A}, i} \sigma^{-1}$  is partially contracted and degenerate to lower order, but nontrivial, cycles. One may consider initializing a state like Eq.(188), but that conflicts our approach to bound  $\|\rho_{R \cup \bar{B}} - \rho_{R \cup \bar{B}, \text{avg}}\|_1$  in the following and we leave problem to future research work.

#### Computation Using Abstract Indices

By matrix Hölder inequality [60, 61],

$$\|\rho_{R \cup \bar{B}} - \rho_{R \cup \bar{B}, \text{avg}}\|_1 \leq (d_R d_{\bar{B}})^{\frac{1}{2}} \|\rho_{R \cup \bar{B}} - \rho_{R \cup \bar{B}, \text{avg}}\|_2^{\frac{1}{2}}. \quad (211)$$

Moreover,

$$\mathbb{E}[\|\rho_{R \cup \bar{B}} - \rho_{R \cup \bar{B}, \text{avg}}\|_2] = \mathbb{E}[\text{Tr}((\rho_{R \cup \bar{B}} - \rho_{R \cup \bar{B}, \text{avg}})^2)^{\frac{1}{2}}]. \quad (212)$$

We then use Jensen's inequality to get

$$\mathbb{E}[\|\rho_{R\cup\bar{B}} - \rho_{R\cup\bar{B},\text{avg}}\|_2] \leq \mathbb{E}[\text{Tr}((\rho_{R\cup\bar{B}} - \rho_{R\cup\bar{B},\text{avg}})^2)]^{\frac{1}{2}} = \left(\mathbb{E}[\text{Tr}(\rho_{R\cup\bar{B}}^2)] - \text{Tr}(\rho_{R\cup\bar{B},\text{avg}}^2)\right)^{\frac{1}{2}}. \quad (213)$$

As a result,

$$\mathbb{E}[\sqrt{\|\rho_{R\cup\bar{B}} - \rho_{R\cup\bar{B},\text{avg}}\|_1}] \leq \sqrt{\mathbb{E}[\|\rho_{R\cup\bar{B}} - \rho_{R\cup\bar{B},\text{avg}}\|_1]} \leq \sqrt{(d_R d_{\bar{B}})^{1/2} (\mathbb{E}[\text{Tr}(\rho_{R\cup\bar{B}}^2)] - \text{Tr}(\rho_{R\cup\bar{B},\text{avg}}^2))^{1/2}}. \quad (214)$$

A precise calculation of  $\mathbb{E}[\text{Tr}(\rho_{R\cup\bar{B}}^2)] - \text{Tr}(\rho_{R\cup\bar{B},\text{avg}}^2)$  not only enables us to estimate  $\mathbb{E}[\epsilon_{\text{Choi}}]$  but also bounds the probability for large Choi error by Markov inequality. Ref.[35] tackles the problem by the *partial decoupling theorem* established in [62]. We elucidate our attempts based on results of SU( $d$ )-symmetric 2-design developed before.

Using abstract indices, the initial state under action is

$$D^{RB\bar{B}}_{R'B'\bar{B}'} = U^{B\bar{B}}_{A\bar{A}} Q^{RA} P^{\bar{A}}_{\bar{A}'} Q_{R'A'} U_{B'\bar{B}'}^{A'\bar{A}'}. \quad (215)$$

It should be careful that  $Q^{RA}$  is a state purified by the reference  $R$  but  $P^{\bar{A}}_{\bar{A}'}$  is a general (mixed) state with no entanglement to other qudits for a convenient definition of group equivariance (see Eq.(186)).

By definition

$$\text{Tr}(\rho_{R\cup\bar{B},\text{avg}}^2) = \left(\int D^{RB\bar{B}}_{R'B'\bar{B}'} dU\right) \left(\int D^{R'B'\bar{B}'}_{RB'\bar{B}} dV\right) = \left(\int D^{R\bar{B}}_{R'\bar{B}'} dU\right) \left(\int D^{R'\bar{B}'}_{R\bar{B}} dV\right). \quad (216)$$

We denote  $P^{\bar{A}}_{\bar{A}'} = \rho^{\bar{A}}_{\bar{A}'}$ ,  $Q^{RA} Q_{RA'''} = \mu^A_{A'''}$  as in Section III A, then the integrand is expanded as

$$\begin{aligned} & D(U)^{RB\bar{B}}_{R'B'\bar{B}'} D(V)^{R'B'\bar{B}'}_{RB'\bar{B}} \\ &= (U^{B\bar{B}}_{A\bar{A}} Q^{RA} P^{\bar{A}}_{\bar{A}'} Q_{R'A'} U_{B'\bar{B}'}^{A'\bar{A}'})(V^{B'\bar{B}'}_{A''\bar{A}''} Q^{R'A''} P^{\bar{A}''}_{\bar{A}'''} Q_{RA'''} V_{B'\bar{B}'}^{A'''\bar{A}''''}) \\ &= \mu^A_{A'''} \mu^{A''}_{A'''} \rho^{\bar{A}}_{\bar{A}'} \rho^{\bar{A}''}_{\bar{A}'''} U^{B\bar{B}}_{A\bar{A}} U_{B\bar{B}'}^{A'\bar{A}'} V^{B'\bar{B}'}_{A''\bar{A}''} V_{B'\bar{B}'}^{A'''\bar{A}''''} \\ &= (U^{B\bar{B}}_{A\bar{A}} \mu^A_{A'''} \rho^{\bar{A}}_{\bar{A}'} U_{B\bar{B}'}^{A'\bar{A}'})(V^{B'\bar{B}'}_{A''\bar{A}''} \mu^{A''}_{A'''} \rho^{\bar{A}''}_{\bar{A}'''} V_{B'\bar{B}'}^{A'''\bar{A}''''}) \\ &= \tilde{U}^{B\bar{B}}_{A'''\bar{A}'} U_{B\bar{B}'}^{A'\bar{A}'} \tilde{V}^{B'\bar{B}'}_{A''\bar{A}''} V_{B'\bar{B}'}^{A'''\bar{A}''''}. \end{aligned} \quad (217)$$

It would be further cleaned up by taking transpositions  $T^{Q_A'' Q_A'}_{A'A'''}, T^{Q_B' Q_B}_{BB'}$  (Pauli matrices are denoted by  $P, Q$  for now):

$$\begin{aligned} & T^{Q_A'' Q_A'}_{A'A'''} T^{Q_B' Q_B}_{BB'} \tilde{U}^{B\bar{B}}_{A'''\bar{A}'} U_{Q_B\bar{B}'}^{A'\bar{A}'} \tilde{V}^{B'\bar{B}'}_{A''\bar{A}''} V_{Q_B'\bar{B}}^{A'''\bar{A}''''} \\ &= \frac{1}{d_A d_B} \sum_{P,Q} P^{Q_A''}_{A'} P^{Q_A'}_{A'''} Q^{Q_B}_{B'} Q^{Q_B}_{B''} \tilde{U}^{B\bar{B}}_{A'''\bar{A}'} (U^{B\bar{B}}_{A\bar{A}} \mu^A_{A'''} \rho^{\bar{A}}_{\bar{A}'} U_{Q_B\bar{B}'}^{A'\bar{A}'})(V^{B'\bar{B}'}_{A''\bar{A}''} \mu^{A''}_{A'''} \rho^{\bar{A}''}_{\bar{A}'''} V_{Q_B'\bar{B}}^{A'''\bar{A}''''}) \\ &= \frac{1}{d_A d_B d_A^2} \sum_{P,Q} (U^{B\bar{B}}_{A\bar{A}} P^A_{A'} \rho^{\bar{A}}_{\bar{A}'} U_{Q_B\bar{B}'}^{A'\bar{A}'} Q^{Q_B}_{B'} (V^{B'\bar{B}'}_{A''\bar{A}''} P^{A''}_{A'''} \rho^{\bar{A}''}_{\bar{A}'''} V_{Q_B'\bar{B}}^{A'''\bar{A}''''} Q^{Q_B}_{B''} \end{aligned} \quad (218)$$

Rewritten in a concise form we get

$$\text{Tr}(\rho_{R\cup\bar{B},\text{avg}}^2) = \frac{1}{d_A^3 d_B} \sum_{P_A, P_B} \int \text{Tr}(U(P_A \otimes \rho_{\bar{A}}) U^\dagger P_B V (P_A^\dagger \otimes \rho_{\bar{A}}) V^\dagger P_B^\dagger) dU dV. \quad (219)$$

By exactly the same method, we immediately have

$$\mathbb{E}[\text{Tr}(\rho_{R\cup\bar{B}}^2)] = \frac{1}{d_A^3 d_B} \sum_{P_A, P_B} \int \text{Tr}(U(P_A \otimes \rho_{\bar{A}}) U^\dagger P_B U (P_A^\dagger \otimes \rho_{\bar{A}}) U^\dagger P_B^\dagger) dU. \quad (220)$$

We hope to perform similar techniques to evaluate the above integrals as in the last subsection, but the matrix  $P_A \otimes \rho_{\bar{A}}$  does not admit SU( $d$ ) symmetry on the entire system of  $n$  qudits which leads to intractable terms when expanding by  $T_{k=2}^{\text{CQA}}$ . One possible strategy to remedy the problem is selecting  $\rho_{\bar{A}}$  from any trivial SU( $d$ ) trivial irrep decomposed from  $n - k$  qudits, which demands  $n - k$  to be divided by the integer  $d$  according to Littlewood-Richardson rule [1, 3]. The advantage is that  $\rho_{\bar{A}}$ , as a 1-dimensional density matrix in some SU( $d$ ) trivial irrep sector, is obviously pure and we explain in the following that

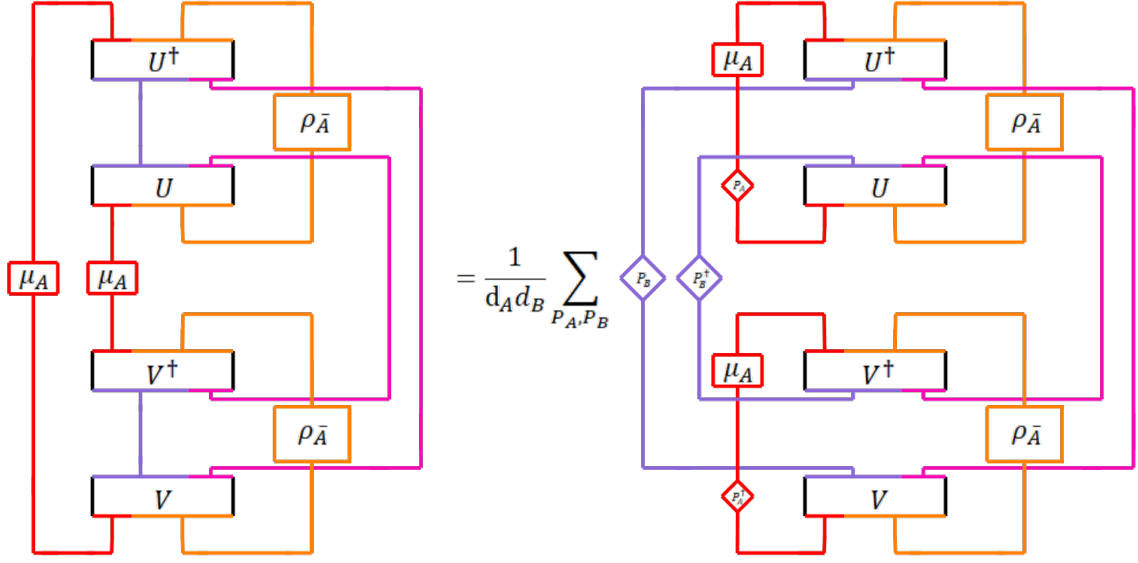

FIG. 2. Tensor network diagram illustrating the deduction from Eq.(217) to (219).

this choice helps to overcome the mathematical difficulty when averaging the  $\text{Tr}(\rho_{R \cup \bar{B}}^2)$  over the group  $U(\bigoplus_{\lambda} S^{\lambda})$  of  $SU(d)$  symmetric unitaries. For instance, when  $d = 2$  or  $3$ , we initialize  $\rho_{\bar{A}} = |\psi_{\bar{A}}\rangle \langle \psi_{\bar{A}}|$  as tensor products of  $SU(2)$  or  $SU(3)$  singlets:

$$\left( \frac{1}{\sqrt{2}}(|01\rangle - |10\rangle) \right)^{\otimes(n-k)/2}, \quad \left( \frac{1}{\sqrt{6}}(|uds\rangle - |usd\rangle + |dsu\rangle - |dus\rangle + |sud\rangle - |sdu\rangle) \right)^{\otimes(n-k)/3}. \quad (221)$$

With this assumption, it is now legal to decompose  $P_{\bar{A}'}^{\bar{A}}$  as  $P_{\bar{A}'}^{\bar{A}} P_{\bar{A}'}^{\bar{A}'}$ . Then we rewrite Eq.(217):

$$\begin{aligned} & D(U)^{RB\bar{B}}_{R'B\bar{B}'} D(V)^{R'B'\bar{B}'}_{RB'\bar{B}'} \\ &= (U^{B\bar{B}}_{A\bar{A}} Q^{RA}_{\bar{A}'} P_{\bar{A}'}^{\bar{A}} Q_{R'A'} U_{B\bar{B}'}^{A'\bar{A}'}) (V^{B'\bar{B}'}_{A''\bar{A}''} Q^{R'A''} P_{\bar{A}''}^{\bar{A}''} Q_{RA''} V_{B'\bar{B}'}^{A''\bar{A}''}) \\ &= \mu_{A'''}^A \mu_{A'''}^{A''} \rho_{A'''}^{\bar{A}} \rho_{\bar{A}'''}^{\bar{A}''} U_{A\bar{A}}^{B\bar{B}} U_{B\bar{B}'}^{A'\bar{A}'} V_{A''\bar{A}''}^{B'\bar{B}'} V_{B'\bar{B}'}^{A''\bar{A}''} \\ &= (U_{A\bar{A}}^{B\bar{B}} \mu_{A'''}^A \rho_{\bar{A}'''}^{\bar{A}}) (U_{B\bar{B}'}^{A'\bar{A}'} \mu_{A'''}^{A''} \rho_{\bar{A}''}^{\bar{A}''}) V_{A''\bar{A}''}^{B'\bar{B}'} V_{B'\bar{B}'}^{A''\bar{A}''} \\ &= \tilde{U}_{A'''\bar{A}'''}^{B\bar{B}} \tilde{U}_{B\bar{B}'}^{A'\bar{A}'} V_{A''\bar{A}''}^{B'\bar{B}'} V_{B'\bar{B}'}^{A''\bar{A}''} \end{aligned} \quad (222)$$

The difference happens when we write  $\rho_{\bar{A}'''}^{\bar{A}} \rho_{\bar{A}''}^{\bar{A}''}$  instead of  $\rho_{\bar{A}'}^{\bar{A}} \rho_{\bar{A}''}^{\bar{A}''}$  in Eq.(217). This simple modification allows us to swap only a pair of indices now e.g.,  $\bar{B}$  and  $\bar{B}'$ :

$$\begin{aligned} & T^{\bar{Q}'_B \bar{Q}_B}_{\bar{B}\bar{B}'} \tilde{U}_{A'''\bar{A}'''}^{B\bar{B}} \tilde{U}_{B\bar{Q}'_B}^{A'\bar{A}'} V_{A''\bar{A}''}^{B'\bar{B}'} V_{B'\bar{Q}_B}^{A''\bar{A}''} \\ &= \frac{1}{d_{\bar{B}} d_A^2} \sum_P P_{\bar{B}}^{\bar{Q}'_B} P_{\bar{B}'}^{\bar{Q}_B} (U_{A'''\bar{A}'''}^{B\bar{B}} \rho_{\bar{A}'''}^{\bar{A}}) (U_{B\bar{Q}'_B}^{A'\bar{A}'} \rho_{\bar{A}''}^{\bar{A}''}) V_{A''\bar{A}''}^{B'\bar{B}'} V_{B'\bar{Q}_B}^{A''\bar{A}''} \\ &= \frac{1}{d_{\bar{B}} d_A^2} \sum_P (U_{A'''\bar{A}'''}^{B\bar{B}} \rho_{\bar{A}'''}^{\bar{A}}) V_{B'\bar{Q}_B}^{A''\bar{A}''} P_{\bar{B}'}^{\bar{Q}_B} V_{A''\bar{A}''}^{B'\bar{B}'} (U_{B\bar{Q}'_B}^{A'\bar{A}'} \rho_{\bar{A}''}^{\bar{A}''}) P_{\bar{B}}^{\bar{Q}'_B}. \end{aligned} \quad (223)$$

Thus

$$\text{Tr}(\rho_{R \cup \bar{B}}^2)_{\text{avg}} = \frac{1}{d_A^2 d_B} \sum_{P_B} \int \text{Tr} \left( U(I_A \otimes \rho_{\bar{A}}) V^\dagger P_B V (I_A \otimes \rho_{\bar{A}}) U^\dagger P_B^\dagger \right) dU dV \quad (224)$$

with

$$\mathbb{E}[\text{Tr}(\rho_{R \cup \bar{B}}^2)] = \frac{1}{d_A^2 d_B} \sum_{P_B} \int \text{Tr} \left( U(I_A \otimes \rho_{\bar{A}}) U^\dagger P_B U (I_A \otimes \rho_{\bar{A}}) U^\dagger P_B^\dagger \right) dU. \quad (225)$$

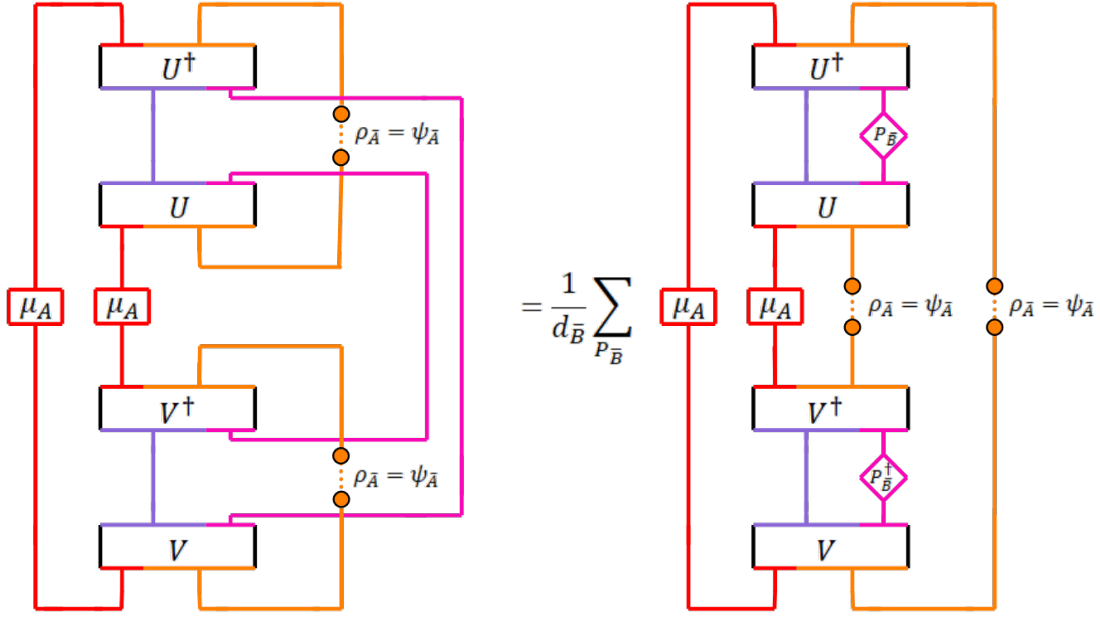

FIG. 3. Tensor network diagram illustrating how to obtain Eq.(224) when  $\rho_{\bar{A}}$  is initialized as a pure state represented as dots connected by dashed line in the diagram.

We first integrate Eq.(225) by the expansion of  $T_{k=2}^{\text{CQA}}$  in Eq.(120) and (121), which has been decorated for SU( $d$ ) symmetric conserved quantities in Eq.(131) and (132) and can be directly reused here:

$$\begin{aligned}
 & \frac{1}{d_\lambda^2 - 1} \left( \text{Tr}(\Pi_{\lambda, m_\lambda}(I_A \otimes \rho_{\bar{A}})) \text{Tr}(\Pi_{\lambda, m'_\lambda}(I_A \otimes \rho_{\bar{A}})) \text{Tr}(\Pi_{\lambda, m_\lambda} P_{\bar{B}} \Pi_{\lambda, m'_\lambda} P_{\bar{B}}^\dagger) \right. \\
 & \quad + \text{Tr}(\Pi_{\lambda, m_\lambda}(I_A \otimes \rho_{\bar{A}}) \Pi_{\lambda, m_\lambda, m'_\lambda}(I_A \otimes \rho_{\bar{A}})) \text{Tr}(\Pi_{\lambda, m'_\lambda, m_\lambda} P_{\bar{B}}) \text{Tr}(\Pi_{\lambda, m_\lambda, m'_\lambda} P_{\bar{B}}^\dagger) \\
 & \quad - \frac{1}{d_\lambda} \text{Tr}(\Pi_{\lambda, m_\lambda} W^\dagger) \text{Tr}(\Pi_{\lambda, m'_\lambda}(I_A \otimes \rho_{\bar{A}})) \text{Tr}(\Pi_{\lambda, m'_\lambda, m_\lambda} P_{\bar{B}}) \text{Tr}(\Pi_{\lambda, m_\lambda, m'_\lambda} P_{\bar{B}}^\dagger) \\
 & \quad \left. - \frac{1}{d_\lambda} \text{Tr}(\Pi_{\lambda, m_\lambda}(I_A \otimes \rho_{\bar{A}})) \Pi_{\lambda, m_\lambda, m'_\lambda}(I_A \otimes \rho_{\bar{A}}) \text{Tr}(\Pi_{\lambda, m_\lambda} P_{\bar{B}} \Pi_{\lambda, m'_\lambda} P_{\bar{B}}^\dagger), \right) \quad (226)
 \end{aligned}$$

with

$$\frac{1}{d_\lambda d_\mu} \text{Tr}(\Pi_{\lambda, m_\lambda}(I_A \otimes \rho_{\bar{A}})) \text{Tr}(\Pi_{\mu, m_\mu}(I_A \otimes \rho_{\bar{A}})) \text{Tr}(\Pi_{\lambda, m_\lambda} P_{\bar{B}} \Pi_{\mu, m_\mu} P_{\bar{B}}^\dagger). \quad (227)$$

On the other hand, the integrand of  $\text{Tr}(\rho_{R \cup \bar{B}, \text{avg}}^2)$  embraces product of  $T_{k=1}^{\text{CQA}}(P_{\bar{B}}), T_{k=1}^{\text{CQA}}(P_{\bar{B}}^\dagger)$  (1-design) which is straightforward to be expanded as:

$$\frac{1}{d_\lambda} \text{Tr} \left( \left( \sum_i E_{(\alpha_i^\lambda, m_1), (\alpha_i^\lambda, m_2)} \right) P_{\bar{B}} \right) \left( \sum_i E_{(\alpha_i^\lambda, m_1), (\alpha_i^\lambda, m_2)} \right), \quad \frac{1}{d_\mu} \text{Tr} \left( \left( \sum_j E_{(\alpha_j^\mu, m'_1), (\alpha_j^\mu, m'_2)} \right) P_{\bar{B}}^\dagger \right) \left( \sum_j E_{(\alpha_j^\mu, m'_1), (\alpha_j^\mu, m'_2)} \right) \quad (228)$$

with contractions with  $(I_A \otimes \rho_{\bar{A}})$  and yielding

$$\begin{aligned}
 & \frac{1}{d_\lambda d_\mu} \text{Tr} \left( \left( \sum_i E_{(\alpha_i^\lambda, m_1), (\alpha_i^\lambda, m_2)} \right) P_{\bar{B}} \right) \text{Tr} \left( \left( \sum_j E_{(\alpha_j^\mu, m'_1), (\alpha_j^\mu, m'_2)} \right) P_{\bar{B}}^\dagger \right) \\
 & \quad \text{Tr} \left( \left( \sum_i E_{(\alpha_i^\lambda, m_1), (\alpha_i^\lambda, m_2)} \right) (I_A \otimes \rho_{\bar{A}}) \left( \sum_j E_{(\alpha_j^\mu, m'_1), (\alpha_j^\mu, m'_2)} \right) (I_A \otimes \rho_{\bar{A}}) \right). \quad (229)
 \end{aligned}$$

Since  $I_A \otimes \rho_{\bar{A}}$  is SU( $d$ ) symmetric, we need  $\lambda = \mu$  with  $m_2 = m'_1 = m_\lambda, m_1 = m'_2 = m'_\lambda$  to get nonzero trace from the RHS

from above, which equals

$$\begin{aligned} & \text{Tr} \left( \left( \sum_i E_{(\alpha_i^\lambda, m'_\lambda), (\alpha_i^\lambda, m_\lambda)} \right) (I_A \otimes \rho_{\bar{A}}) \left( \sum_j E_{(\alpha_j^\lambda, m_\lambda), (\alpha_j^\lambda, m'_\lambda)} \right) (I_A \otimes \rho_{\bar{A}}) \right) \\ &= \sum_{i,j} (I_A \otimes \rho_{\bar{A}})_{(\alpha_i^\lambda, m_\lambda), (\alpha_j^\lambda, m_\lambda)} (I \otimes \rho_{\bar{A}})_{(\alpha_j^\lambda, m'_\lambda), (\alpha_i^\lambda, m'_\lambda)}. \end{aligned} \quad (230)$$

As a result, Eq.(229) is rewritten as

$$\frac{1}{d_\lambda^2} \text{Tr}(\Pi_{\lambda, m'_\lambda, m_\lambda} P_{\bar{B}}) \text{Tr}(\Pi_{\lambda, m_\lambda, m'_\lambda} P_{\bar{B}}^\dagger) \text{Tr}(\Pi_{\lambda, m_\lambda} (I_A \otimes \rho_{\bar{A}}) \Pi_{\lambda, m_\lambda, m'_\lambda} (I_A \otimes \rho_{\bar{A}})), \quad (231)$$

which is used to cancel the second term in Eq.(227) because  $d_\lambda^2 - 1 \approx d_\lambda^2$  for nontrivial  $S_n$  irrep. For the trivial  $S_n$  irrep, we reformulate the 2-design expansion in Eq.(227) and find that these terms are still identical. Finally,

$$\begin{aligned} & \mathbb{E}[\text{Tr}(\rho_{R \cup \bar{B}}^2)] - \text{Tr}(\rho_{R \cup \bar{B}, \text{avg}}^2) \\ & \approx \frac{1}{d_A^2 d_{\bar{B}}} \sum_{P_{\bar{B}}} \left( \sum_{\lambda, \mu, m_\lambda, m_\mu} \frac{1}{d_\lambda d_\mu} \text{Tr}(\Pi_{\lambda, m_\lambda} (I_A \otimes \rho_{\bar{A}})) \text{Tr}(\Pi_{\mu, m_\mu} (I_A \otimes \rho_{\bar{A}})) \text{Tr}(\Pi_{\lambda, m_\lambda} P_{\bar{B}} \Pi_{\mu, m_\mu} P_{\bar{B}}^\dagger) \right. \\ & \quad - \sum_{\lambda, m_\lambda, m'_\lambda} \frac{1}{(d_\lambda^2 - 1) d_\lambda} \text{Tr}(\Pi_{\lambda, m_\lambda} (I_A \otimes \rho_{\bar{A}})) \text{Tr}(\Pi_{\lambda, m'_\lambda} (I_A \otimes \rho_{\bar{A}})) \text{Tr}(\Pi_{\lambda, m'_\lambda, m_\lambda} P_{\bar{B}}) \text{Tr}(\Pi_{\lambda, m_\lambda, m'_\lambda} P_{\bar{B}}^\dagger) \\ & \quad \left. - \frac{1}{(d_\lambda^2 - 1) d_\lambda} \text{Tr}(\Pi_{\lambda, m_\lambda} (I_A \otimes \rho_{\bar{A}}) \Pi_{\lambda, m_\lambda, m'_\lambda} (I_A \otimes \rho_{\bar{A}})) \text{Tr}(\Pi_{\lambda, m_\lambda} P_{\bar{B}} \Pi_{\lambda, m'_\lambda} P_{\bar{B}}^\dagger) \right) \end{aligned} \quad (232)$$

We analyze the scaling behavior for each term in the above identity as we did in Section III B:

1. Obviously,

$$0 \leq \text{Tr}(\Pi_{\lambda, m_\lambda} (I_A \otimes \rho_{\bar{A}})) \leq \text{Tr}(I_A \otimes \rho_{\bar{A}}) = d_A, \quad 0 \leq \text{Tr}(\Pi_{\lambda, m_\lambda} P_{\bar{B}} \Pi_{\mu, m_\mu} P_{\bar{B}}^\dagger) \leq \min\{d_\mu, d_\lambda\}. \quad (233)$$

2. Since the initial state  $\rho_{\bar{A}}$  is selected from the  $SU(d)$  trivial irrep, or by Schur-Weyl duality, the  $S_n$  irrep to the Young diagram  $\lambda_0 = (\frac{n-k}{d}, \dots, \frac{n-k}{d})$ . Using  $S_n$  branching rule [2, 3], the matrix  $I_A \otimes \rho_{\bar{A}}$  is exactly decomposed into  $S_n$  irreps of Young diagrams  $\lambda$  built by adding  $k$  more boxes to  $\lambda_0$ , which satisfy  $\lambda_1, \lambda'_1 \approx \frac{n}{d}$  as long as  $k = o(n)$ . Their dimension is lower bounded by (see the end of Section I A)

$$\dim S^\lambda = d_\lambda \geq \frac{d^n}{n^{d(d+2)/2}}. \quad (234)$$

3. The total number of  $\lambda$  stemmed from  $\lambda_0$  is  $p(k, d)$  (Definition I.4), which is upper bounded by Eq.(7) with  $n$  being replaced by  $k$ . The multiplicity for each of these irreps is also polynomially bounded in  $n$ .

In summary, given  $k = o(n)$

$$\mathbb{E}[\text{Tr}(\rho_{R \cup \bar{B}}^2)] - \text{Tr}(\rho_{R \cup \bar{B}, \text{avg}}^2) \leq d_{\bar{B}} \sum_{\lambda, \mu, m_\lambda, m_\mu} \frac{1}{d_\lambda d_\mu} \min\{d_\mu, d_\lambda\} = \frac{1}{e^{\Omega(n)}}. \quad (235)$$

### E. Overparametrization Regime with $SU(d)$ Symmetric Local Quantities

We now discuss the application of the unitary  $k$ -design to the trainability of the variational ansatz. Let us consider the CQA ansatz  $U(\theta)$  that respects the symmetry of  $SU(d)$ :

$$\begin{aligned} U(\theta) &= \exp(-iH_{\text{YJM}}(\beta)) \exp(-iH_S(\gamma)) = \exp(-i \sum_{k,l} \beta_{kl} X_k X_l) \exp(-i\gamma \sum_{j=1}^{n-1} (j, j+1)) \\ &= \left( \prod_{k,l} \exp(-i\beta_{kl} X_k X_l) \right) \exp(-i\gamma \sum_{j=1}^{n-1} (j, j+1)), \end{aligned} \quad (236)$$

where  $X_k X_l$  are product of YJM-elements (Definition I.2) and  $(j, j+1)$  are adjacent SWAPs with parameters  $\theta = (\beta_{kl}, \gamma)$ . Since YJM-elements commutes with each other, we have  $\exp(-i \sum_{k,l} \beta_{kl} X_k X_l) = \prod_{k,l} \exp(-i \beta_{kl} X_k X_l)$ . Decomposing the second exponential of adjacent SWAPs however introduces Trotter errors. Then we consider some state initialization  $|\psi^\lambda\rangle = |\alpha_T^\lambda, m\rangle$  in one  $S_n$  irrep sector  $S^\lambda$ . We would also consider the statistical ensemble  $\rho_\lambda$  of these states later.

For a given observable  $\hat{O}$  that is  $SU(d)$  symmetric, e.g., the Heisenberg Hamiltonian where we could write down:

$$\hat{O} = \sum_{i=1}^N O_i, \quad (237)$$

where each  $O_i$  contains a single term. In the case of quantum many-body with locality assumption, we typically assume the number  $N$  of  $O_i$  scales linearly or polynomially with the number of qubits. Then we define the loss:

$$\frac{1}{2} \left( \text{Tr}(U(\theta) \rho_\lambda U^\dagger(\theta) \hat{O}) - E_0 \right)^2 = \left( \text{Tr}(\rho_\lambda U^\dagger(\theta) \hat{O} U(\theta)) - E_0 \right)^2 \equiv \frac{1}{2} \varepsilon^2. \quad (238)$$

It is proved in [12] that this ansatz approximate  $SU(d)$ -symmetric  $k$ -designs where  $k = \Omega(n^2)$  the square of the number of qudits. Note that for the particular form of the ansatz, we can write:

$$U(\theta)_{\text{CQA}} = U_{-,l} U_{+,l}, \quad (239)$$

where  $l = 1, \dots, L$  is the index for the variational angles. Note that our ansatz can be further Trotterized into products of time evolution of unitaries and each of which is only parameterized by one variational angle. Then the differentiation with chain rule easily reads:

$$\frac{\partial U(\theta)}{\partial \theta_l} = U_{-,l} (-i H_{\text{CQA},l}) U_{+,l}, \quad \frac{\partial U^\dagger(\theta)}{\partial \theta_l} = U_{+,l}^\dagger (i H_{\text{CQA},l}) U_{-,l}^\dagger, \quad (240)$$

where  $H_{\text{CQA},l}$  denotes the generator (YJM-elements or SWAPs) of the CQA ansatz driven by the parameter  $\theta_l$ . The QNTK is given by:

$$\begin{aligned} K &= \sum_l \frac{\partial \bar{\varepsilon}}{\partial \theta_l} \frac{\partial \varepsilon}{\partial \theta_l} = \sum_l \left| \langle \psi^\lambda | U_{+,l}^\dagger \left[ H_{\text{CQA},l}, U_{-,l}^\dagger \hat{O} U_{-,l} \right] U_{+,l} | \psi^\lambda \rangle \right|^2 \\ &= - \left( \langle \psi^\lambda | U_{+,l}^\dagger \left[ H_{\text{CQA},l}, U_{-,l}^\dagger \hat{O} U_{-,l} \right] U_{+,l} | \psi^\lambda \rangle \right)^2, \\ &= - \left( \sum_{i=1}^N \langle \psi^\lambda | U_{+,l}^\dagger \left[ H_{\text{CQA},l}, U_{-,l}^\dagger O_i U_{-,l} \right] U_{+,l} | \psi^\lambda \rangle \right)^2, \end{aligned} \quad (241)$$

since the trace of products of Hermitian and anti-Hermitian matrices is pure imaginary. Recall that the observable  $\hat{O}$  is  $SU(d)$  symmetric and  $|\psi^\lambda\rangle$  (or  $\rho_\lambda$ ) is taken from one  $S_n$  irrep sector, we exclusively concern the unitary  $U^\lambda$  restricted to that irrep block and

$$K = - \sum_l \sum_{i,j=1}^N \text{Tr}(\rho_\lambda U_{+,l}^{\lambda\dagger} [H_{\text{CQA},l}^\lambda, O_i^{\lambda,I}] U_{+,l}^\lambda \rho_\lambda U_{+,l}^{\lambda\dagger} [H_{\text{CQA},l}^\lambda, O_j^{\lambda,I}] U_{+,l}^\lambda), \quad (242)$$

where we define the interaction picture observable  $\hat{O}^I = U_{-,l}^{\lambda\dagger} \hat{O} U_{-,l}^\lambda$  (and similarly for  $O_i^{\lambda,I}$ ) with general statistical ensemble  $\rho_\lambda$ . The assumption to respecting  $SU(d)$  symmetry is practical in the experiment which also provides an accessible way to average the above identity by Haar randomness of  $SU(d)$  symmetric unitaries. As explained in the previous context, twirling a general operator  $M$  with no assumption on symmetry leads to most intricate properties in this topic (see Section II D and III A).

We now compute the average  $\bar{K}$  when  $U_+, U_-$  are independent  $SU(d)$  symmetric unitaries and match the Haar measure up to the second moment:

$$\bar{K} = - \sum_l \int \left( \int \text{Tr}(\rho_\lambda U_{+,l}^{\lambda\dagger} [H_{\text{CQA},l}^\lambda, O^{\lambda,I}] U_{+,l}^\lambda \rho_\lambda U_{+,l}^{\lambda\dagger} [H_{\text{CQA},l}^\lambda, O^{\lambda,I}] U_{+,l}^\lambda) dU_{+,l} \right) dU_{-,l}. \quad (243)$$

The integral involving  $U_{+,l}$  is evaluated by first projecting  $[H_{\text{CQA},l}^\lambda, O^{\lambda,I}] \otimes [H_{\text{CQA},l}^\lambda, O^{\lambda,I}]$  by the 2th-fold channel  $T_{k=2}^{\text{CQA}}$  and then we contract with  $\rho_\lambda \otimes \rho_\lambda$ . Then we integrate  $U_{-,l}$  similarly. Since we assume the symmetry and restrict to one  $S_n$  irrep,  $T_{k=2}^{\text{CQA}}(M)$  takes a quite simple form resembling the Haar projection with no symmetry (cf. Eq. (112)):

$$T_{k=2}^{\text{CQA}}(M) = \frac{1}{d_\lambda^2 - 1} (\text{Tr}(M) I_\lambda^{\otimes 2} + \text{Tr}(S_\lambda M) S_\lambda - \frac{1}{d_\lambda} \text{Tr}(M) S_\lambda - \frac{1}{d_\lambda} \text{Tr}(S_\lambda M) I_\lambda^{\otimes 2}), \quad (244)$$



where  $I_\lambda$  is the identity matrix restrict to the irrep  $S^\lambda$  and  $S_\lambda$  exchanges tensor products from  $S^\lambda \otimes S^\lambda$  (cf. Eq.(111)). In our cases,

$$T_{k=2}^{\text{CQA}}([H_{\text{CQA},l}^\lambda, O^{\lambda,I}]^{\otimes 2}) = \frac{1}{d_\lambda^2 - 1} (\text{Tr}([H_{\text{CQA},l}^\lambda, O^{\lambda,I}]^2 I_\lambda^{\otimes 2}) + \text{Tr}([H_{\text{CQA},l}^\lambda, O^{\lambda,I}]^2) S_\lambda - \frac{1}{d_\lambda} \text{Tr}([H_{\text{CQA},l}^\lambda, O^{\lambda,I}]^2) S_\lambda - \frac{1}{d_\lambda} \text{Tr}([H_{\text{CQA},l}^\lambda, O^{\lambda,I}]^2) I_\lambda^{\otimes 2}) \quad (245)$$

Since the trace of any Lie bracket vanishes, contracting with  $\rho_\lambda^{\otimes 2}$ , we obtain

$$\begin{aligned} & \int \text{Tr}(\rho_\lambda U_{+,l}^{\lambda\dagger} [H_{\text{CQA},l}^\lambda, O^{\lambda,I}] U_{+,l}^\lambda \rho_\lambda U_{+,l}^{\lambda\dagger} [H_{\text{CQA},l}^\lambda, O^{\lambda,I}] U_{+,l}^\lambda) dU_{+,l} \\ &= \frac{1}{d_\lambda^2 - 1} \left( \text{Tr}([H_{\text{CQA},l}^\lambda, O^{\lambda,I}]^2) \text{Tr}(\rho_\lambda)^2 - \frac{1}{d_\lambda} \text{Tr}([H_{\text{CQA},l}^\lambda, O^{\lambda,I}]^2) \text{Tr}(\rho_\lambda^2) \right). \end{aligned} \quad (246)$$

To integrate  $U_{-,l}$ , we note that  $\text{Tr}([H_{\text{CQA},l}^\lambda, O^{\lambda,I}]^2) = 2\text{Tr}(H_{\text{CQA},l}^\lambda O^{\lambda,I} H_{\text{CQA},l}^\lambda O^{\lambda,I}) - 2\text{Tr}((H_{\text{CQA},l}^\lambda)^2 (O^{\lambda,I})^2)$  and apply the above method again:

$$\begin{aligned} & \int \text{Tr}(H_{\text{CQA},l}^\lambda O^{\lambda,I} dU_{-,l}) \\ &= \frac{1}{d_\lambda^2 - 1} \left( \text{Tr}(O^{\lambda,2}) \text{Tr}(H_{\text{CQA},l}^{\lambda,2}) + \text{Tr}(O^{\lambda,2}) \text{Tr}(H_{\text{CQA},l}^\lambda)^2 - \frac{1}{d_\lambda} \text{Tr}(O^{\lambda,2}) \text{Tr}(H_{\text{CQA},l}^\lambda)^2 - \frac{1}{d_\lambda} \text{Tr}(O^{\lambda,2}) \text{Tr}(H_{\text{CQA},l}^{\lambda,2}) \right). \end{aligned} \quad (247)$$

On the other hand  $\text{Tr}((H_{\text{CQA},l}^\lambda)^2 (O^{\lambda,I})^2) = \text{Tr}((H_{\text{CQA},l}^\lambda)^2 U_{-,l}^\dagger O^{\lambda,2} U_{-,l})$  is evaluated by the 1-design projection  $T_{k=1}^{\text{CQA}}$ :

$$\int \text{Tr}((H_{\text{CQA},l}^\lambda)^2 (O^{\lambda,I})^2) dU_{-,l} = \frac{1}{d_\lambda} \text{Tr}(O^{\lambda,2}) \text{Tr}((H_{\text{CQA},l}^\lambda)^2). \quad (248)$$

When  $\rho_\lambda$  is pure, the results are gathered as

$$\begin{aligned} & \frac{2}{d_\lambda^2 + d_\lambda} \sum_l \left( \frac{d_\lambda \text{Tr}(O^{\lambda,2}) - \text{Tr}(O^{\lambda,2})}{d_\lambda^2 - 1} \text{Tr}(H_{\text{CQA},l}^{\lambda,2}) - \frac{d_\lambda \text{Tr}(O^{\lambda,2}) - \text{Tr}(O^{\lambda,2})}{d_\lambda^3 - d_\lambda} \text{Tr}(H_{\text{CQA},l}^\lambda)^2 \right) \\ &= \frac{2}{(d_\lambda + 1)(d_\lambda^2 - 1)} \left( \text{Tr}(O^{\lambda,2}) - \frac{\text{Tr}(O^{\lambda,2})}{d_\lambda} \right) \sum_l \left( \text{Tr}(H_{\text{CQA},l}^{\lambda,2}) - \frac{\text{Tr}(H_{\text{CQA},l}^\lambda)^2}{d_\lambda} \right). \end{aligned} \quad (249)$$

By power mean inequality

$$\left( \frac{1}{n} \sum \lambda_i^2 \right)^{\frac{1}{2}} \geq \frac{1}{n} \sum |\lambda_i|, \quad (250)$$

the above term is always nonnegative. As a easy way to bound  $\text{Tr}(H_{\text{CQA},l}^{\lambda,2}) - \frac{\text{Tr}(H_{\text{CQA},l}^\lambda)^2}{d_\lambda}$ , we may assume the ansatz is Trotterized consisting of time evolution of 2-, 3-, (2, 2)-cycles due to YJM-elements. Then

$$\text{Tr}((i, j)^2) - \frac{\text{Tr}((i, j))^2}{d_\lambda} = (1 - \bar{\chi}_\lambda(i, j)) d_\lambda, \quad (251)$$

$$\text{Tr}(((i, j, k) + (k, j, i))^{\lambda,2}) - \frac{\text{Tr}((i, j, k) + (k, j, i))^2}{d_\lambda} = 2(1 - \bar{\chi}_\lambda(i, j, k)) d_\lambda, \quad (252)$$

$$\text{Tr}(((i, j)(k, l))^2) - \frac{\text{Tr}((i, j)(k, l))^2}{d_\lambda} = (1 - \bar{\chi}_\lambda(i, j)(k, l)) d_\lambda, \quad (253)$$

where  $(i, j, k) + (k, j, i)$  is defined to make the operator Hermitian. For qubits ( $d = 2$ ) and two-row Young diagrams  $\lambda = (n - r, r)$  [19–21],

$$\bar{\chi}_\lambda(i, j, k) = \frac{n^2 - (3r + 1)n + 3r^2 - 3r}{n(n - 1)}, \quad (254)$$

$$\bar{\chi}_\lambda(i, j)(k, l) = \frac{n^4 - 2(2r + 3)n^3 + (8r^2 + 12r + 11)n^2 - 2(4r^3 + 4r^2 + 4r + 3)n + 4r^4 - 8r^3 + 28r^2 - 24r}{n(n - 1)(n - 2)(n - 3)}. \quad (255)$$

For  $S_n$  irreps with large dimension ( $r \rightarrow \frac{n}{2}$ ), these character values tend to  $c \cdot d_\lambda$  as we saw in Section III B where  $\bar{\chi}_\lambda(i, j)$  is nearly  $\frac{1}{2}d_\lambda$ . Therefore,

$$\bar{K} \approx \sum_{ij}^N \frac{L}{d_\lambda^2} \left( \text{Tr}(O_i^\lambda O_j^\lambda) - \frac{\text{Tr}(O_i^\lambda) \text{Tr}(O_j^\lambda)}{d_\lambda} \right) \approx \frac{N^2 L}{d_\lambda}, \quad (256)$$

where we assume that the observable is a sum of SWAPs. Then we use again the fact that the character of these local operators scales as  $c \cdot d_\lambda$  for large  $d_\lambda$  given by

$$d_\lambda = \dim S^{(n-r, r)} = \binom{n}{r} - \binom{n}{r-1} = \frac{n-2r+1}{n-r+1} \binom{n}{r} \quad (257)$$

in Section I A.

- 
- [1] W. Fulton, *Young tableaux: with applications to representation theory and geometry* (Cambridge University Press, Cambridge [England], 1997).
  - [2] B. E. Sagan, *The symmetric group*, 2nd ed., Graduate Texts in Mathematics, Vol. 203 (Springer-Verlag, New York, 2001) pp. xvi+238, representations, combinatorial algorithms, and symmetric functions.
  - [3] R. Goodman and N. R. Wallach, *Symmetry, Representations, and Invariants* (Springer New York, 2009).
  - [4] T. Ceccherini-Silberstein, F. Scarabotti, and F. Tolli, *Representation Theory of the Symmetric Groups* (Cambridge University Press, 2009).
  - [5] H. Zheng, Z. Li, J. Liu, S. Strelchuk, and R. Kondor, PRX Quantum **4**, 020327 (2023).
  - [6] A. Young, *The Collected Papers of Alfred Young 1873–1940*, edited by G. de Beauregard Robinson (University of Toronto Press, 1977).
  - [7] A.-A. Jucys, Reports on Mathematical Physics **5**, 107 (1974).
  - [8] G. Murphy, Journal of Algebra **69**, 287 (1981).
  - [9] A. Okounkov and A. Vershik, Selecta Mathematica **2**, 581 (1996).
  - [10] M. Clausen and U. Baum, Mathematics of Computation **61**, 833 (1993).
  - [11] D. K. Maslen, Math. Comp **67**, 1121 (1998).
  - [12] Z. Li, H. Zheng, J. Liu, L. Jiang, and Z.-W. Liu, arXiv preprint arXiv:2309.0815 (2023).
  - [13] G. H. Hardy and S. Ramanujan, Proceedings of the London Mathematical Society **s2-17**, 75 (1918).
  - [14] J. V. Uspensky, Bulletin de l'Academie des Sciences de Russie. VI serie **14**, 199 (1920).
  - [15] H. Rademacher, Proceedings of the London Mathematical Society **s2-43**, 241 (1938).
  - [16] P. Erdos, The Annals of Mathematics **43**, 437 (1942).
  - [17] A. Maróti, Integers **3** (2003).
  - [18] W. De Azevedo Pribitkin, The Ramanujan Journal **18**, 113 (2009).
  - [19] S. R. E. Ingram, Proceedings of the American Mathematical Society **1**, 358 (1950).
  - [20] Y. Roichman, Inventiones Mathematicae **125**, 451 (1996).
  - [21] M. Lassalle, Mathematische Annalen **340**, 383 (2008).
  - [22] J. Gallier, *Discrete Mathematics* (Springer New York, 2011).
  - [23] S. P. Mishchenko, Sbornik: Mathematics **187**, 81 (1996).
  - [24] A. Giambruno and S. Mishchenko, Proceedings of the American Mathematical Society **144**, 943 (2015).
  - [25] H. Krovi, Quantum **3**, 122 (2019).
  - [26] A. Y. Vlasov, Phys. Rev. A **63**, 054302 (2001).
  - [27] F. G. Brandao, A. W. Harrow, and M. Horodecki, Communications in Mathematical Physics **346**, 397 (2016).
  - [28] A. Harrow and S. Mehraban, arXiv preprint arXiv:1809.06957 (2018).
  - [29] I. Marin, Annales de l'Institut Fourier **53**, 1323 (2003).
  - [30] I. Marin, Journal of Algebra **310**, 742 (2007).
  - [31] I. Marvian, H. Liu, and A. Hulse, arXiv e-prints, arXiv:2105.12877 (2021), arXiv:2105.12877 [quant-ph].
  - [32] J. Watrous, *The Theory of Quantum Information* (Cambridge University Press, 2018).
  - [33] S. Xu and B. Swingle, arXiv e-prints, arXiv:2202.07060 (2022), arXiv:2202.07060 [quant-ph].
  - [34] H. Tajima, R. Takagi, and Y. Kuramochi, arXiv e-prints, arXiv:2206.11086 (2022), arXiv:2206.11086 [quant-ph].
  - [35] L. Kong and Z.-W. Liu, PRX Quantum **3**, 020314 (2022).
  - [36] A. W. Harrow and R. A. Low, in *Approximation, Randomization, and Combinatorial Optimization. Algorithms and Techniques*, edited by I. Dinur, K. Jansen, J. Naor, and J. Rolim (Springer Berlin Heidelberg, Berlin, Heidelberg, 2009) pp. 548–561.
  - [37] M. Hastings and A. Harrow, Quantum Information and Computation **9**, 336 (2009).
  - [38] D. Gross, S. Nezami, and M. Walter, Communications in Mathematical Physics **385**, 1325 (2021).
  - [39] J. Haferkamp and N. Hunter-Jones, Physical Review A **104**, 022417 (2021).
  - [40] D. Gross, K. Audenaert, and J. Eisert, Journal of Mathematical Physics **48**, 052104 (2007).
  - [41] D. A. Roberts and B. Yoshida, Journal of High Energy Physics **2017**, 121 (2017).

- [42] J. Cotler, N. Hunter-Jones, J. Liu, and B. Yoshida, *Journal of High Energy Physics* **2017**, 1 (2017).
- [43] N. Hunter-Jones, arXiv preprint arXiv:1905.12053 (2019).
- [44] J. Liu, *Phys. Rev. Research* **2**, 043164 (2020).
- [45] S.-K. Jian, G. Bentsen, and B. Swingle, “Linear growth of circuit complexity from brownian dynamics,” (2022).
- [46] W. Van Dam, *On Quantum Computation Theory*, Ph.D. thesis (2002).
- [47] R. A. Low, *Pseudo-randomness and Learning in Quantum Computation*, Ph.D. thesis (2010).
- [48] P. Diaconis, *Group representations in probability and statistics*, Lecture notes-monograph series No. v. 11 (Institute of Mathematical Statistics, Hayward, Calif, 1988).
- [49] D. Applebaum, *Probability on Compact Lie Groups*, Probability Theory and Stochastic Modelling, Vol. 70 (Springer International Publishing, 2014).
- [50] E. S. Meckes, *The random matrix theory of the classical compact groups*, Cambridge tracts in mathematics No. 212 (Cambridge University Press, Cambridge ; New York, NY, 2019).
- [51] E. M. Rains, *The Electronic Journal of Combinatorics* **5**, R12 (1998).
- [52] K. Schmüdgen, arXiv preprint arXiv:2008.12698 (2020).
- [53] B. Collins, *International Mathematics Research Notices* **2003**, 953 (2003).
- [54] H. Tasaki, *Physics and Mathematics of Quantum Many-Body Systems* (Springer International Publishing, 2020).
- [55] R. Rasala, *Journal of Algebra* **45**, 132 (1977).
- [56] M. Sellke, arXiv e-prints , arXiv:2004.05283 (2020), arXiv:2004.05283 [math.CO].
- [57] D. Bacon, I. L. Chuang, and A. W. Harrow, *PRL* **97**, 170502 (2006), arXiv:quant-ph/0407082 [quant-ph].
- [58] V. Havlíček and S. Strelchuk, *Physical Review Letters* **121** (2018), 10.1103/physrevlett.121.060505.
- [59] C. Bény and O. Oreshkov, *Phys. Rev. Lett.* **104**, 120501 (2010).
- [60] S. M. Manjegani, *Positivity* **11**, 239 (2007).
- [61] B. Baumgartner, arXiv e-prints , arXiv:1106.6189 (2011), arXiv:1106.6189 [math-ph].
- [62] E. Wakakuwa and Y. Nakata, *Communications in Mathematical Physics* **386**, 589 (2021).
